# Supplementary material for: First-Passage Time Fluctuation Theorem and Thermodynamic Bound in Cooperative Biomolecular Networks
Source: arXiv:2501.09087 ancillary file (2026-11-19)
Supplement: Supplementary file 1 [file supplemental-material.pdf]

# Supplemental Material for First-Passage Time Fluctuation Theorem and Thermodynamic Bound in Cooperative Biomolecular Networks

D. Evan Piephoff and Jianshu Cao*
*Department of Chemistry, Massachusetts Institute of Technology, Cambridge, Massachusetts 02139, United States*

## PATHWAY ANALYSIS FOR ENZYMATIC MODEL

Here, we describe our pathway analysis framework (that reduces to the transition rate matrix approach but is more general) [1, 2] and adapt it to the enzymatic model in Fig. 1(a) of the main text. In Fig. 1(a) of the main text, let $B_0$ represent the free enzyme state manifold, and let $B_1$ represent the substrate-bound enzymatic complex. Let the $B_0$-to-$B_1$ ($B_1$-to-$B_0$) manifold transition for substrate binding (unbinding) be described by the waiting time matrix $\check{\mathbf{W}}^{(0+)}(z)$ ($\check{\mathbf{W}}^{(1-)}(z)$). Also, let the $B_1$-to-$B_0$ ($B_0$-to-$B_1$) manifold transition for product formation (reverse product formation) be described by the waiting time matrix $\check{\mathbf{W}}^{(1+)}(z)$ ($\check{\mathbf{W}}^{(0-)}(z)$). The chain of manifolds is unfolded about $B_0$ into an equivalent representation (shown in Fig. S1) that has two pathways (involving manifolds $\{B'_m\}$ with underlying states $\{A_{l,m}\}$) representing the forward and backward observable processes, with $\check{\mathbf{W}}^{(-1\pm)}(z) = \check{\mathbf{W}}^{(1\pm)}(z)$ by symmetry. Here, transitions for the observable (hidden) process are described by waiting time distribution functions $\left\{\check{Q}^{k,l}_{m\pm}(z)\right\}$ ($\left\{\check{R}^{(m)}_{k,l}(z)\right\}$), with $\check{Q}^{l,1}_{-1\pm}(z) = \check{Q}^{l,1}_{1\pm}(z)$. Since the transitions are rate processes, $\check{Q}^{k,l}_{m\pm}(z) = k^{k,l}_{m\pm} / \left(z + \sum_k \left[\gamma^{(m)}_{k,l} + k^{k,l}_{m+} + k^{k,l}_{m-}\right]\right)$ and $\check{R}^{(m)}_{k,l}(z) = \gamma^{(m)}_{k,l} / \left(z + \sum_k \left[\gamma^{(m)}_{k,l} + k^{k,l}_{m+} + k^{k,l}_{m-}\right]\right)$, where $k^{k,l}_{m\pm}$ and $\gamma^{(m)}_{k,l}$ represent the rates corresponding to $\check{Q}^{k,l}_{m\pm}(z)$ and $\check{R}^{(m)}_{k,l}(z)$, respectively, with $k^{l,1}_{-1\pm} = k^{l,1}_{1\pm}$. In terms of the rates in Fig. 1(a) of the main text, $k^{1,l}_{0+} = k^{(l)}_1$, $k^{1,l}_{0-} = k^{(l)}_{-2}$, $k^{l,1}_{1+} = k^{(l)}_2$, $k^{l,1}_{1-} = k^{(l)}_{-1}$, $\gamma^{(0)}_{2,1} = \gamma_1$, and $\gamma^{(0)}_{1,2} = \gamma_{-1}$.

We define $\check{\mathbf{R}}^{(m)}(z)$ (which has the element $\check{R}^{(m)}_{k,l}(z)$) as a square waiting time matrix for the hidden process. We define the waiting time matrix $\check{\mathbf{T}}^{(m\pm)}(z)$, which need not be square, as $\check{T}^{(m\pm)}_{j,k}(z) = \check{Q}^{j,k}_{m\pm}(z)$. The matrix $\check{\mathbf{W}}^{(m\pm)}(z)$ is then given by

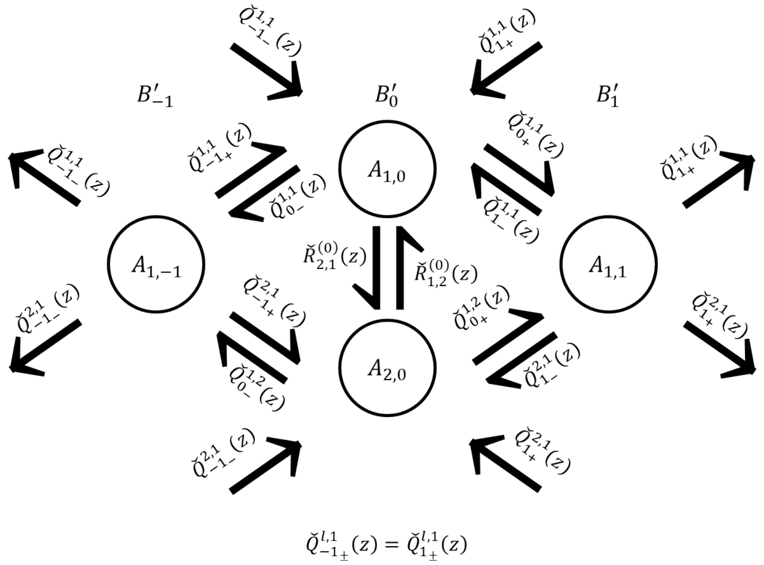


Figure S1. Unfolded representation of the enzymatic scheme in Fig. 1(a) of the main text (see text below for details).

$$\check{\mathbf{W}}^{(m_\pm)}(z) = \check{\mathbf{T}}^{(m_\pm)}(z)\left[\mathbf{I}_{L_m} - \check{\mathbf{R}}^{(m)}(z)\right]^{-1} \tag{S1}$$

where $L_m$ is the number of states within $B'_m$, and $\mathbf{I}_{L_m}$ is the identity matrix of order $L_m$. The matrix $\underline{\check{\mathbf{W}}}^{(m_+)}(z)$ ($\underline{\check{\mathbf{W}}}^{(m_-)}(z)$) accounts for branching, and is defined as the waiting time matrix for completing the transition corresponding to $\check{\mathbf{W}}^{(m_+)}(z)$ ($\check{\mathbf{W}}^{(m_-)}(z)$) after having passed out of and back to $B'_m$ to the left (right) in a manner that avoids the completion of the backward (forward) process. We express $\underline{\check{\mathbf{W}}}^{(m_\pm)}(z)$ in the recurrence relation

$$\underline{\check{\mathbf{W}}}^{(m_\pm)}(z) = \check{\mathbf{W}}^{(m_\pm)}(z) + \underline{\check{\mathbf{W}}}^{(m_\pm)}(z)\,\underline{\check{\mathbf{W}}}^{([m\mp1]_\pm)}(z)\,\check{\mathbf{W}}^{(m_\mp)}(z) \tag{S2}$$

which is solved self-consistently as

$$\underline{\check{\mathbf{W}}}^{(m_\pm)}(z) = \check{\mathbf{W}}^{(m_\pm)}(z)\left[\mathbf{I}_{L_m} - \underline{\check{\mathbf{W}}}^{([m\mp1]_\pm)}(z)\,\check{\mathbf{W}}^{(m_\mp)}(z)\right]^{-1} \tag{S3}$$

where $\underline{\check{\mathbf{W}}}^{(\pm1_\mp)}(z) = \check{\mathbf{W}}^{(\pm1_\mp)}(z)$ here.

We can concatenate these expressions to form the forward/backward first-passage time pathway matrix as

$$\check{\mathbf{\Omega}}_\pm(z) = \underline{\check{\mathbf{W}}}^{(\pm1_\pm)}(z)\,\underline{\check{\mathbf{W}}}^{(0_\pm)}(z) \tag{S4}$$

It is noted that the waiting time matrices in Eqs. (S2)–(S4) are written in a particular order. The unnormalized forward/backward first-passage time PDF is then given by

$$\check{P}_\pm(z) = \sum_{j=1}^{L_0}\left[\check{\mathbf{\Omega}}_\pm(z)\,\bar{\mathbf{P}}^{\mathrm{ev},0}\right]_j \tag{S5}$$

Here, the event-averaged initial population distribution vector is given by the solution to

$$\bar{\mathbf{P}}^{\mathrm{ev},0} = \check{\mathbf{\Omega}}(0)\,\bar{\mathbf{P}}^{\mathrm{ev},0} \tag{S6}$$

subject to the constraint

$$\sum_{l=1}^{L_0}\bar{P}_l^{\mathrm{ev},0} = 1 \tag{S7}$$

where the total first-passage time pathway matrix is expressed as $\check{\mathbf{\Omega}}(z) = \check{\mathbf{\Omega}}_+(z) + \check{\mathbf{\Omega}}_-(z)$.

## EVALUATION OF FIRST-PASSAGE TIME DISTRIBUTIONS

Continuing with the scheme in Fig. S1, we now use our pathway technique to calculate the first-passage time distributions. We first consider the waiting time matrix $\check{\mathbf{W}}^{(m_\pm)}(z)$ [see Eq. (S1)]. For a $2\times2$ matrix $\mathbf{M}$ that is nonsingular,

$$\mathbf{M}^{-1} = \frac{1}{\det[\mathbf{M}]}\begin{pmatrix} M_{2,2} & -M_{1,2} \\ -M_{2,1} & M_{1,1}\end{pmatrix} \tag{S8}$$

Since the only nonzero elements of $\check{\mathbf{R}}^{(0)}(z)$ are the off-diagonal ones, from Eq. (S8), we see that $\left[\mathbf{I}_2 - \check{\mathbf{R}}^{(0)}(z)\right]^{-1} = \left[\mathbf{I}_2 + \check{\mathbf{R}}^{(0)}(z)\right]/\det\left[\mathbf{I}_2 - \check{\mathbf{R}}^{(0)}(z)\right]$. Using the definitions of $\check{\mathbf{R}}^{(m)}(z)$ and $\check{\mathbf{T}}^{(m_\pm)}(z)$ given above, we can then write $\check{\mathbf{W}}^{(0_\pm)}(z)$ as

$$\check{\mathbf{W}}^{(0_\pm)}(z) = \frac{1}{1-\check{R}^{(0)}_{1,2}(z)\,\check{R}^{(0)}_{2,1}(z)}\left(\check{Q}^{1,1}_{0_\pm}(z)+\check{Q}^{1,2}_{0_\pm}(z)\,\check{R}^{(0)}_{2,1}(z)\quad \check{Q}^{1,2}_{0_\pm}(z)+\check{Q}^{1,1}_{0_\pm}(z)\,\check{R}^{(0)}_{1,2}(z)\right) \tag{S9}$$

Additionally, it is seen that $\check{\mathbf{W}}^{(1_\pm)}(z)=\check{\mathbf{T}}^{(1_\pm)}(z)$.

Next, we consider the matrix $\underline{\check{\mathbf{W}}}^{(m_\pm)}(z)$. Using Eqs. (S3) and (S9), as well as the definition of $\check{\mathbf{T}}^{(m_\pm)}(z)$, we can write

$$\begin{aligned}\underline{\check{\mathbf{W}}}^{(0_\pm)}(z) &= \check{\mathbf{W}}^{(0_\pm)}(z)\left[\mathbf{I}_2-\check{\mathbf{T}}^{(1_\pm)}(z)\check{\mathbf{W}}^{(0_\mp)}(z)\right]^{-1}\\ &= \tfrac{1}{\mathscr{D}_{0_\pm}}\Big(\check{Q}^{1,1}_{0_\pm}(z)\Big(1-\check{Q}^{2,1}_{1_\pm}(z)\check{Q}^{1,2}_{0_\mp}(z)\Big)+\check{Q}^{1,2}_{0_\pm}(z)\Big(\check{Q}^{2,1}_{1_\pm}(z)\check{Q}^{1,1}_{0_\mp}(z)+\check{R}^{(0)}_{2,1}(z)\Big)\quad \check{Q}^{1,2}_{0_\pm}(z)\Big(1-\check{Q}^{1,1}_{1_\pm}(z)\check{Q}^{1,1}_{0_\mp}(z)\Big)+\check{Q}^{1,1}_{0_\pm}(z)\Big(\check{Q}^{1,1}_{1_\pm}(z)\check{Q}^{1,2}_{0_\mp}(z)+\check{R}^{(0)}_{1,2}(z)\Big)\Big)\end{aligned} \tag{S10}$$

where

$$\mathscr{D}_{0_\pm} = 1-\left(\check{Q}^{1,1}_{1_\pm}(z)+\check{R}^{(0)}_{1,2}(z)\,\check{Q}^{2,1}_{1_\pm}(z)\right)\check{Q}^{1,1}_{0_\mp}(z)-\left(\check{Q}^{2,1}_{1_\pm}(z)+\check{R}^{(0)}_{2,1}(z)\,\check{Q}^{1,1}_{1_\pm}(z)\right)\check{Q}^{1,2}_{0_\mp}(z)-\check{R}^{(0)}_{1,2}(z)\,\check{R}^{(0)}_{2,1}(z) \tag{S11}$$

With an expression for $\underline{\check{\mathbf{W}}}^{(0_\pm)}(z)$, it is then straightforward to construct $\underline{\check{\mathbf{W}}}^{(\pm 1_\pm)}(z)$ and $\check{\boldsymbol{\Omega}}_\pm(z)$ as

$$\underline{\check{\mathbf{W}}}^{(\pm 1_\pm)}(z) = \frac{\check{\mathbf{T}}^{(1_\pm)}(z)}{1-\underline{\check{\mathbf{W}}}^{(0_\pm)}(z)\cdot\check{\mathbf{T}}^{(1_\mp)}(z)} \tag{S12}$$

$$\check{\boldsymbol{\Omega}}_\pm(z) = \frac{\check{\mathbf{T}}^{(1_\pm)}(z)\,\underline{\check{\mathbf{W}}}^{(0_\pm)}(z)}{1-\underline{\check{\mathbf{W}}}^{(0_\pm)}(z)\cdot\check{\mathbf{T}}^{(1_\mp)}(z)} \tag{S13}$$

From Eq. (S6), it is seen that $\bar{\mathbf{P}}^{\mathrm{ev},0}$ is the eigenvector of $\check{\boldsymbol{\Omega}}(0)$ having an eigenvalue of unity. Thus, using the definitions of $\left\{\check{Q}^{k,l}_{m_\pm}(z)\right\}$ and $\left\{\check{R}^{(m)}_{k,l}(z)\right\}$ above, as well as that for $\check{\boldsymbol{\Omega}}(z)$, $\bar{\mathbf{P}}^{\mathrm{ev},0}$ is given by the solution to the equation

$$\left[\check{\boldsymbol{\Omega}}(0)-\mathbf{I}_2\right]\bar{\mathbf{P}}^{\mathrm{ev},0}=\mathbf{0} \tag{S14}$$

subject to the constraint in Eq. (S7), with $\mathbf{0}$ representing the null vector. Using Eq. (S5), we achieve the expressions for $\check{P}_+(z)$ and $\check{P}_-(z)$ provided in the attached Mathematica [3] printout [referred to as Pplus (see Out[37] and, equivalently, In[38]) and Pminus (see Out[40] and, equivalently, In[41]), respectively], where the notation employed for transition quantities is described as follows (with s used in place of $z$): $\check{Q}^{1,1}_{0_+}(z)\to$ Q0plus11[s], $\check{Q}^{1,2}_{0_+}(z)\to$ Q0plus12[s], $\check{Q}^{1,1}_{1_-}(z)\to$ Q1minus11[s], $\check{Q}^{2,1}_{1_-}(z)\to$ Q1minus21[s], $\check{Q}^{1,1}_{1_+}(z)\to$ Q1plus11[s], $\check{Q}^{2,1}_{1_+}(z)\to$ Q1plus21[s], $\check{Q}^{1,1}_{0_-}(z)\to$ Q0minus11[s], $\check{Q}^{1,2}_{0_-}(z)\to$ Q0minus12[s], $\check{R}^{(0)}_{2,1}(z)\to$ R210[s], $\check{R}^{(0)}_{1,2}(z)\to$ R120[s], $k^{(1)}_1\to$ k11, $k^{(2)}_1\to$ k12, $k^{(1)}_{-1}\to$ km11, $k^{(2)}_{-1}\to$ km12, $k^{(1)}_2\to$ k21, $k^{(2)}_2\to$ k22, $k^{(1)}_{-2}\to$ km21, $k^{(2)}_{-2}\to$ km22, $\gamma_1\to$ gamma1, and $\gamma_{-1}\to$ gammam1. In addition, using $p_\pm=\check{P}_\pm(0)$, the expressions for $p_+$ and $p_-$ included in the attached Mathematica [3] printout [referred to as pplus (see Out[42]) and pminus (see Out[43]), respectively] are attained.

As indicated in the main text, we substitute in the local detailed balance constraints [Eqs. (2) and (3) in the main text] with $k^{(2)}_1$ and $\gamma_{-1}$ (this choice is arbitrary), resulting in $\exp\left[\Delta s^{\mathrm{tot}}/k_{\mathrm{B}}\right]=k^{(1)}_1k^{(1)}_2/\left(k^{(1)}_{-1}k^{(1)}_{-2}\right)$ and $J\propto\left[k^{(1)}_2/k^{(1)}_{-1}-k^{(2)}_2/k^{(2)}_{-1}\right]$. We then arrive at Eq. (4) in the main text by evaluating $\check{P}_+(z)/\check{P}_-(z)-k^{(1)}_1k^{(1)}_2/\left(k^{(1)}_{-1}k^{(1)}_{-2}\right)$, the complete expression for which is provided in the attached Mathematica [3] printout (see Out[55]). Similarly, we arrive at Eqs. (8)–(10) in the main text by evaluating $p_+/p_--k^{(1)}_1k^{(1)}_2/\left(k^{(1)}_{-1}k^{(1)}_{-2}\right)$.

Consider the scenario in which there is an arbitrarily large number of states in $B'_0$, as well as hidden loops between them and $A_{1,\pm1}$. We can map such a scheme onto Fig. S1, where $A_{1,0}$ and $A_{2,0}$ now represent aggregates of states undergoing non-Poissonian decay. When hidden detailed balance is satisfied in all but one of the hidden loops (resulting in only one nonzero hidden current $J$), then the kinetics of the balanced hidden loops can be treated implicitly [2], such that the basic form of Eq. (4) in the main text is recovered [the same is true for Eq. (8) in the main text]; however, the complete expression for $\check{\alpha}(z)\,J$ (as well as that for $-\zeta^{\mathrm{eff}}J^2$) will presumably be much lengthier. When

there is also an arbitrarily large number of states in $B'_{\pm 1}$, as well as hidden loops between them and $B'_0$, we can again map this scheme onto Fig. S1, where all the states are now aggregates that undergo non-Poissonian decay. Again, when hidden detailed balance is satisfied in all but one of the hidden loops (with hidden current $J$), then the kinetics of the balanced hidden loops can be treated implicitly [2], again recovering the basic forms of Eqs. (4) and (8) in the main text. Thus, these forms are quite general (holding for any single unbalanced hidden loop between $B'_0$ and $B'_{\pm 1}$), and our signature of hidden detailed balance breaking applies to all schemes corresponding to the generic model in Fig. 2(a) of the main text.

## CALCULATION OF HIDDEN CURRENT

In order to obtain a complete expression for $J$, we first need the stationary population distribution vector $\boldsymbol{\rho}^{\mathrm{s}}$, which is given by the solution to $\mathbf{K}\boldsymbol{\rho}^{\mathrm{s}} = \mathbf{0}$, subject to the constraint $\sum_j \rho_j^{\mathrm{s}} = 1$. Here, the matrix $\mathbf{K}$ has the element $K_{i,j} = (2\delta_{i,j} - 1)\sum_\nu k_{i,j}^{(\nu)}$, where $k_{i,j}^{(\nu)}$ is the rate of transition $\nu$ from state $j$ to state $i$, with the depletion rate for state $j$ given by $\sum_\nu k_{j,j}^{(\nu)} = \sum_{i\neq j,\nu} k_{i,j}^{(\nu)}$. For the model in Fig. 1(a) of the main text, we can write $\mathbf{K}$ as

$$\mathbf{K} = \begin{pmatrix} k_1^{(1)} + k_{-2}^{(1)} + \gamma_1 & -\gamma_{-1} & -\left(k_{-1}^{(1)} + k_2^{(1)}\right) \\ -\gamma_1 & k_1^{(2)} + k_{-2}^{(2)} + \gamma_{-1} & -\left(k_{-1}^{(2)} + k_2^{(2)}\right) \\ -\left(k_1^{(1)} + k_{-2}^{(1)}\right) & -\left(k_1^{(2)} + k_{-2}^{(2)}\right) & k_{-1}^{(1)} + k_2^{(1)} + k_{-1}^{(2)} + k_2^{(2)} \end{pmatrix} \tag{S15}$$

The vector $\boldsymbol{\rho}^{\mathrm{s}}$ is then given by

$$\boldsymbol{\rho}^{\mathrm{s}} = \mathscr{D}^{-1} \begin{pmatrix} \gamma_{-1}k_{-1}^{(1)} + \gamma_{-1}k_{-1}^{(2)} + k_{-1}^{(1)}k_1^{(2)} + k_{-1}^{(1)}k_{-2}^{(2)} + \gamma_{-1}k_2^{(1)} + k_1^{(2)}k_2^{(1)} + k_{-2}^{(2)}k_2^{(1)} + \gamma_{-1}k_2^{(2)} \\ \gamma_1 k_{-1}^{(1)} + \gamma_1 k_{-1}^{(2)} + k_{-1}^{(2)}k_1^{(1)} + k_{-1}^{(2)}k_{-2}^{(1)} + \gamma_1 k_2^{(1)} + \gamma_1 k_2^{(2)} + k_1^{(1)}k_2^{(2)} + k_{-2}^{(1)}k_2^{(2)} \\ \gamma_{-1}k_1^{(1)} + \gamma_1 k_1^{(2)} + k_1^{(1)}k_1^{(2)} + \gamma_{-1}k_{-2}^{(1)} + k_1^{(2)}k_{-2}^{(1)} + \gamma_1 k_{-2}^{(2)} + k_1^{(1)}k_{-2}^{(2)} + k_{-2}^{(1)}k_{-2}^{(2)} \end{pmatrix} \tag{S16}$$

where

$$\begin{aligned} \mathscr{D} = {} & \gamma_{-1}k_{-1}^{(1)} + \gamma_{-1}k_{-1}^{(2)} + k_{-1}^{(1)}k_1^{(2)} + k_{-1}^{(1)}k_{-2}^{(2)} + \gamma_{-1}k_2^{(1)} + k_1^{(2)}k_2^{(1)} + k_{-2}^{(2)}k_2^{(1)} + \gamma_{-1}k_2^{(2)} \\ & + \gamma_1 k_{-1}^{(1)} + \gamma_1 k_{-1}^{(2)} + k_{-1}^{(2)}k_1^{(1)} + k_{-1}^{(2)}k_{-2}^{(1)} + \gamma_1 k_2^{(1)} + \gamma_1 k_2^{(2)} + k_1^{(1)}k_2^{(2)} + k_{-2}^{(1)}k_2^{(2)} \\ & + \gamma_{-1}k_1^{(1)} + \gamma_1 k_1^{(2)} + k_1^{(1)}k_1^{(2)} + \gamma_{-1}k_{-2}^{(1)} + k_1^{(2)}k_{-2}^{(1)} + \gamma_1 k_{-2}^{(2)} + k_1^{(1)}k_{-2}^{(2)} + k_{-2}^{(1)}k_{-2}^{(2)} \end{aligned} \tag{S17}$$

with $\rho_1^{\mathrm{s}} = \rho_{\mathrm{E}_1}^{\mathrm{s}}$ and $\rho_2^{\mathrm{s}} = \rho_{\mathrm{E}_2}^{\mathrm{s}}$. Using the definition of $J$ given in the main text,

$$J = \gamma^{-1}\mathscr{D}^{-1}\left(\gamma_1 u_1^{(2)}u_{-1}^{(1)} - \gamma_{-1}u_{-1}^{(2)}u_1^{(1)}\right) \tag{S18}$$

Upon substituting in the local detailed balance constraints with $k_1^{(2)}$ and $\gamma_{-1}$ [note that they have not yet been substituted into Eqs. (S15)–(S18)], we achieve the updated expression for $J$ provided in the attached Mathematica [3] printout [referred to as J (see Out[57])]. In addition, using $\zeta^{\mathrm{eff}} = \left(k_1^{(1)}k_2^{(1)}/\left(k_{-1}^{(1)}k_{-2}^{(1)}\right) - p_+/p_-\right)/J^2$, the expression for $\zeta^{\mathrm{eff}}$ included in the attached Mathematica [3] printout [referred to as zetaeff (see Out[58])] is attained.

---

* jianshu@mit.edu

[1] J. Cao and R. J. Silbey, Generic schemes for single-molecule kinetics. 1: Self-consistent pathway solutions for renewal processes, J. Phys. Chem. B **112**, 12867 (2008).
[2] D. E. Piephoff and J. Cao, Generic schemes for single-molecule kinetics. 3: Self-consistent pathway solutions for nonrenewal processes, J. Phys. Chem. B **122**, 4601 (2018).
[3] Wolfram Research, Inc., Mathematica, Version 13.2, Champaign, IL (2022).

```
In[1]:= R0 = Function[s, {{0, R120[s]}, {R210[s], 0}}]

Out[1]= Function[s, {{0, R120[s]}, {R210[s], 0}}]

In[2]:= T0plus = Function[s, {{Q0plus11[s], Q0plus12[s]}}]

Out[2]= Function[s, {{Q0plus11[s], Q0plus12[s]}}]

In[3]:= T0minus = Function[s, {{Q0minus11[s], Q0minus12[s]}}]

Out[3]= Function[s, {{Q0minus11[s], Q0minus12[s]}}]

In[4]:= T1plus = Function[s, {{Q1plus11[s]}, {Q1plus21[s]}}]

Out[4]= Function[s, {{Q1plus11[s]}, {Q1plus21[s]}}]

In[5]:= T1minus = Function[s, {{Q1minus11[s]}, {Q1minus21[s]}}]

Out[5]= Function[s, {{Q1minus11[s]}, {Q1minus21[s]}}]

In[6]:= W0plus = Function[s, 1 / (1 - R120[s] * R210[s]) * T0plus[s].(IdentityMatrix[2] + R0[s])]
```

Out[6]= $\text{Function}\left[s, \frac{\text{T0plus}[s].(\text{IdentityMatrix}[2]+\text{R0}[s])}{1-\text{R120}[s]\times\text{R210}[s]}\right]$

```
In[7]:= Simplify[W0plus[s]]
```

Out[7]= $\left\{\left\{\frac{\text{Q0plus11}[s]+\text{Q0plus12}[s]\times\text{R210}[s]}{1-\text{R120}[s]\times\text{R210}[s]}, \frac{\text{Q0plus12}[s]+\text{Q0plus11}[s]\times\text{R120}[s]}{1-\text{R120}[s]\times\text{R210}[s]}\right\}\right\}$

```
In[8]:= W0minus =
         Function[s, 1 / (1 - R120[s] * R210[s]) * T0minus[s].(IdentityMatrix[2] + R0[s])]
```

Out[8]= $\text{Function}\left[s, \frac{\text{T0minus}[s].(\text{IdentityMatrix}[2]+\text{R0}[s])}{1-\text{R120}[s]\times\text{R210}[s]}\right]$

```
In[9]:= Simplify[W0minus[s]]
```

Out[9]= $\left\{\left\{\frac{\text{Q0minus11}[s]+\text{Q0minus12}[s]\times\text{R210}[s]}{1-\text{R120}[s]\times\text{R210}[s]}, \frac{\text{Q0minus12}[s]+\text{Q0minus11}[s]\times\text{R120}[s]}{1-\text{R120}[s]\times\text{R210}[s]}\right\}\right\}$

```
In[10]:= W0plusund =
          Function[s, W0plus[s].Inverse[IdentityMatrix[2] - (T1plus[s].W0minus[s])]]

Out[10]=
         Function[s, W0plus[s].Inverse[IdentityMatrix[2] - T1plus[s].W0minus[s]]]
```

```
In[11]:= Simplify[W0plusund[s]]
Out[11]=
{{(Q0plus11[s] (-1 + Q0minus12[s] × Q1plus21[s]) -
      Q0plus12[s] (Q0minus11[s] × Q1plus21[s] + R210[s])) /
    (-1 + Q0minus11[s] (Q1plus11[s] + Q1plus21[s] × R120[s]) + R120[s] × R210[s] +
      Q0minus12[s] (Q1plus21[s] + Q1plus11[s] × R210[s])),
   (Q0plus12[s] (-1 + Q0minus11[s] × Q1plus11[s]) -
      Q0plus11[s] (Q0minus12[s] × Q1plus11[s] + R120[s])) /
    (-1 + Q0minus11[s] (Q1plus11[s] + Q1plus21[s] × R120[s]) + R120[s] × R210[s] +
      Q0minus12[s] (Q1plus21[s] + Q1plus11[s] × R210[s]))}}

In[12]:= W0minusund =
  Function[s, W0minus[s].Inverse[IdentityMatrix[2] - (T1minus[s].W0plus[s])]]
Out[12]=
Function[s, W0minus[s].Inverse[IdentityMatrix[2] - T1minus[s].W0plus[s]]]

In[13]:= Simplify[W0minusund[s]]
Out[13]=
{{(Q0minus11[s] (-1 + Q0plus12[s] × Q1minus21[s]) -
      Q0minus12[s] (Q0plus11[s] × Q1minus21[s] + R210[s])) /
    (-1 + Q0plus11[s] (Q1minus11[s] + Q1minus21[s] × R120[s]) + R120[s] × R210[s] +
      Q0plus12[s] (Q1minus21[s] + Q1minus11[s] × R210[s])),
   (Q0minus12[s] (-1 + Q0plus11[s] × Q1minus11[s]) -
      Q0minus11[s] (Q0plus12[s] × Q1minus11[s] + R120[s])) /
    (-1 + Q0plus11[s] (Q1minus11[s] + Q1minus21[s] × R120[s]) + R120[s] × R210[s] +
      Q0plus12[s] (Q1minus21[s] + Q1minus11[s] × R210[s]))}}

In[14]:= W1plusund = Function[s, T1plus[s] * 1 / (1 - (W0plusund[s].T1minus[s])⟦1, 1⟧)]
Out[14]=
Function[s, T1plus[s] / (1 - (W0plusund[s].T1minus[s])⟦1, 1⟧)]

In[15]:= Wm1minusund = Function[s, T1minus[s] * 1 / (1 - (W0minusund[s].T1plus[s])⟦1, 1⟧)]
Out[15]=
Function[s, T1minus[s] / (1 - (W0minusund[s].T1plus[s])⟦1, 1⟧)]

In[16]:= Omegaplusfunc = Function[s, W1plusund[s].W0plusund[s]]
Out[16]=
Function[s, W1plusund[s].W0plusund[s]]

In[17]:= Omegaminusfunc = Function[s, Wm1minusund[s].W0minusund[s]]
Out[17]=
Function[s, Wm1minusund[s].W0minusund[s]]
```

In[18]:= **Q0plus11 = Function[s, k11 / (s + k11 + km21 + gamma1)]**

Out[18]=

$$\text{Function}\left[s, \frac{k11}{s + k11 + km21 + gamma1}\right]$$

In[19]:= **Q0minus11 = Function[s, km21 / (s + k11 + km21 + gamma1)]**

Out[19]=

$$\text{Function}\left[s, \frac{km21}{s + k11 + km21 + gamma1}\right]$$

In[20]:= **R210 = Function[s, gamma1 / (s + k11 + km21 + gamma1)]**

Out[20]=

$$\text{Function}\left[s, \frac{gamma1}{s + k11 + km21 + gamma1}\right]$$

In[21]:= **Q0plus12 = Function[s, k12 / (s + k12 + km22 + gammam1)]**

Out[21]=

$$\text{Function}\left[s, \frac{k12}{s + k12 + km22 + gammam1}\right]$$

In[22]:= **Q0minus12 = Function[s, km22 / (s + k12 + km22 + gammam1)]**

Out[22]=

$$\text{Function}\left[s, \frac{km22}{s + k12 + km22 + gammam1}\right]$$

In[23]:= **R120 = Function[s, gammam1 / (s + k12 + km22 + gammam1)]**

Out[23]=

$$\text{Function}\left[s, \frac{gammam1}{s + k12 + km22 + gammam1}\right]$$

In[24]:= **Q1minus11 = Function[s, km11 / (s + km11 + k21 + km12 + k22)]**

Out[24]=

$$\text{Function}\left[s, \frac{km11}{s + km11 + k21 + km12 + k22}\right]$$

In[25]:= **Q1plus11 = Function[s, k21 / (s + km11 + k21 + km12 + k22)]**

Out[25]=

$$\text{Function}\left[s, \frac{k21}{s + km11 + k21 + km12 + k22}\right]$$

In[26]:= **Q1minus21 = Function[s, km12 / (s + km11 + k21 + km12 + k22)]**

Out[26]=

$$\text{Function}\left[s, \frac{km12}{s + km11 + k21 + km12 + k22}\right]$$

In[27]:= **Q1plus21 = Function[s, k22 / (s + km11 + k21 + km12 + k22)]**

Out[27]=

$$\text{Function}\left[s, \frac{k22}{s + km11 + k21 + km12 + k22}\right]$$

In[28]:= **Simplify[Together[Omegaplusfunc[s]]]**

Out[28]=

```
{{(k21 (k11 k12 k21 + k11 k12 k22 + k11 k12 km11 + k11 k12 km12 +
      k12 k22 km21 + k11 k21 km22 + k11 km11 km22 + k11 km12 km22 + k11 k12 s +
      k11 k21 s + k11 k22 s + k11 km11 s + k11 km12 s + k11 km22 s + k11 s^2 +
      gammam1 k11 (k21 + k22 + km11 + km12 + s) + gamma1 k12 (k21 + k22 + km11 + km12 + s))) /
   (k11 k12 k21^2 + 2 k11 k12 k21 k22 + k11 k12 k22^2 + k11 k12 k21 km11 + k11 k12 k22 km11 +
    k11 k12 k21 km12 + k11 k12 k22 km12 + k12 k21 k22 km21 + k12 k22^2 km21 +
    k12 k21 km11 km21 + k12 k22 km11 km21 + k12 km11^2 km21 + k12 k21 km12 km21 +
    k12 k22 km12 km21 + k12 km11 km12 km21 + k11 k21^2 km22 + k11 k21 k22 km22 +
    k11 k21 km11 km22 + k11 k22 km11 km22 + k11 k21 km12 km22 + k11 k22 km12 km22 +
    k11 km11 km12 km22 + k11 km12^2 km22 + k21 km11 km21 km22 + k22 km11 km21 km22 +
    km11^2 km21 km22 + k21 km12 km21 km22 + k22 km12 km21 km22 + 2 km11 km12 km21 km22 +
    km12^2 km21 km22 + 2 k11 k12 k21 s + k11 k21^2 s + k12 k21^2 s + 2 k11 k12 k22 s +
    2 k11 k21 k22 s + 2 k12 k21 k22 s + k11 k22^2 s + k12 k22^2 s + k11 k12 km11 s +
    k11 k21 km11 s + 2 k12 k21 km11 s + k11 k22 km11 s + 2 k12 k22 km11 s + k12 km11^2 s +
    k11 k12 km12 s + 2 k11 k21 km12 s + k12 k21 km12 s + 2 k11 k22 km12 s + k12 k22 km12 s +
    k11 km11 km12 s + k12 km11 km12 s + k11 km12^2 s + k12 k21 km21 s + 2 k12 k22 km21 s +
    k21 k22 km21 s + k22^2 km21 s + 2 k12 km11 km21 s + k21 km11 km21 s + 2 k22 km11 km21 s +
    km11^2 km21 s + k12 km12 km21 s + k21 km12 km21 s + 2 k22 km12 km21 s + 2 km11 km12 km21 s +
    km12^2 km21 s + 2 k11 k21 km22 s + k21^2 km22 s + k11 k22 km22 s + k21 k22 km22 s +
    k11 km11 km22 s + 2 k21 km11 km22 s + k22 km11 km22 s + km11^2 km22 s + 2 k11 km12 km22 s +
    2 k21 km12 km22 s + k22 km12 km22 s + 2 km11 km12 km22 s + km12^2 km22 s + k21 km21 km22 s +
    k22 km21 km22 s + 2 km11 km21 km22 s + 2 km12 km21 km22 s + k11 k12 s^2 + 2 k11 k21 s^2 +
    2 k12 k21 s^2 + k21^2 s^2 + 2 k11 k22 s^2 + 2 k12 k22 s^2 + 2 k21 k22 s^2 + k22^2 s^2 + k11 km11 s^2 +
    2 k12 km11 s^2 + 2 k21 km11 s^2 + 2 k22 km11 s^2 + km11^2 s^2 + 2 k11 km12 s^2 + k12 km12 s^2 +
    2 k21 km12 s^2 + 2 k22 km12 s^2 + 2 km11 km12 s^2 + km12^2 s^2 + k12 km21 s^2 + k21 km21 s^2 +
    2 k22 km21 s^2 + 2 km11 km21 s^2 + 2 km12 km21 s^2 + k11 km22 s^2 + 2 k21 km22 s^2 + k22 km22 s^2 +
    2 km11 km22 s^2 + 2 km12 km22 s^2 + km21 km22 s^2 + k11 s^3 + k12 s^3 + 2 k21 s^3 + 2 k22 s^3 +
    2 km11 s^3 + 2 km12 s^3 + km21 s^3 + km22 s^3 + s^4 + gammam1 (k21 + k22 + km11 + km12 + s)
      (km12 km21 + k21 s + k22 s + km12 s + km21 s + s^2 + k11 (k21 + k22 + s) + km11 (km21 + s)) +
    gamma1 (k21 + k22 + km11 + km12 + s)
      (km12 km22 + k21 s + k22 s + km12 s + km22 s + s^2 + k12 (k21 + k22 + s) + km11 (km22 + s))),
  (k21 (k11 k12 k21 + k11 k12 k22 + k11 k12 km11 + k11 k12 km12 + k12 k22 km21 +
      k12 km11 km21 + k12 km12 km21 + k11 k21 km22 + k11 k12 s +
      k12 k21 s + k12 k22 s + k12 km11 s + k12 km12 s + k12 km21 s + k12 s^2 +
      gammam1 k11 (k21 + k22 + km11 + km12 + s) + gamma1 k12 (k21 + k22 + km11 + km12 + s))) /
   (k11 k12 k21^2 + 2 k11 k12 k21 k22 + k11 k12 k22^2 + k11 k12 k21 km11 + k11 k12 k22 km11 +
    k11 k12 k21 km12 + k11 k12 k22 km12 + k12 k21 k22 km21 + k12 k22^2 km21 +
    k12 k21 km11 km21 + k12 k22 km11 km21 + k12 km11^2 km21 + k12 k21 km12 km21 +
    k12 k22 km12 km21 + k12 km11 km12 km21 + k11 k21^2 km22 + k11 k21 k22 km22 +
    k11 k21 km11 km22 + k11 k22 km11 km22 + k11 k21 km12 km22 + k11 k22 km12 km22 +
    k11 km11 km12 km22 + k11 km12^2 km22 + k21 km11 km21 km22 + k22 km11 km21 km22 +
```

```
km11^2 km21 km22 + k21 km12 km21 km22 + k22 km12 km21 km22 + 2 km11 km12 km21 km22 +
km12^2 km21 km22 + 2 k11 k12 k21 s + k11 k21^2 s + k12 k21^2 s + 2 k11 k12 k22 s +
2 k11 k21 k22 s + 2 k12 k21 k22 s + k11 k22^2 s + k12 k22^2 s + k11 k12 km11 s +
k11 k21 km11 s + 2 k12 k21 km11 s + k11 k22 km11 s + 2 k12 k22 km11 s + k12 km11^2 s +
k11 k12 km12 s + 2 k11 k21 km12 s + k12 k21 km12 s + 2 k11 k22 km12 s + k12 k22 km12 s +
k11 km11 km12 s + k12 km11 km12 s + k11 km12^2 s + k12 k21 km21 s + 2 k12 k22 km21 s +
k21 k22 km21 s + k22^2 km21 s + 2 k12 km11 km21 s + k21 km11 km21 s + 2 k22 km11 km21 s +
km11^2 km21 s + k12 km12 km21 s + k21 km12 km21 s + 2 k22 km12 km21 s + 2 km11 km12 km21 s +
km12^2 km21 s + 2 k11 k21 km22 s + k21^2 km22 s + k11 k22 km22 s + k21 k22 km22 s +
k11 km11 km22 s + 2 k21 km11 km22 s + k22 km11 km22 s + km11^2 km22 s + 2 k11 km12 km22 s +
2 k21 km12 km22 s + k22 km12 km22 s + 2 km11 km12 km22 s + km12^2 km22 s + k21 km21 km22 s +
k22 km21 km22 s + 2 km11 km21 km22 s + 2 km12 km21 km22 s + k11 k12 s^2 + 2 k11 k21 s^2 +
2 k12 k21 s^2 + k21^2 s^2 + 2 k11 k22 s^2 + 2 k12 k22 s^2 + 2 k21 k22 s^2 + k22^2 s^2 + k11 km11 s^2 +
2 k12 km11 s^2 + 2 k21 km11 s^2 + 2 k22 km11 s^2 + km11^2 s^2 + 2 k11 km12 s^2 + k12 km12 s^2 +
2 k21 km12 s^2 + 2 k22 km12 s^2 + 2 km11 km12 s^2 + km12^2 s^2 + k12 km21 s^2 + k21 km21 s^2 +
2 k22 km21 s^2 + 2 km11 km21 s^2 + 2 km12 km21 s^2 + k11 km22 s^2 + 2 k21 km22 s^2 + k22 km22 s^2 +
2 km11 km22 s^2 + 2 km12 km22 s^2 + km21 km22 s^2 + k11 s^3 + k12 s^3 + 2 k21 s^3 + 2 k22 s^3 +
2 km11 s^3 + 2 km12 s^3 + km21 s^3 + km22 s^3 + s^4 + gammam1 (k21 + k22 + km11 + km12 + s)
  (km12 km21 + k21 s + k22 s + km12 s + km21 s + s^2 + k11 (k21 + k22 + s) + km11 (km21 + s)) +
gamma1 (k21 + k22 + km11 + km12 + s) (km12 km22 + k21 s + k22 s +
    km12 s + km22 s + s^2 + k12 (k21 + k22 + s) + km11 (km22 + s)))},
{(k22 (k11 k12 k21 + k11 k12 k22 + k11 k12 km11 + k11 k12 km12 + k12 k22 km21 +
      k11 k21 km22 + k11 km11 km22 + k11 km12 km22 + k11 k12 s +
      k11 k21 s + k11 k22 s + k11 km11 s + k11 km12 s + k11 km22 s + k11 s^2 +
      gammam1 k11 (k21 + k22 + km11 + km12 + s) + gamma1 k12 (k21 + k22 + km11 + km12 + s))) /
  (k11 k12 k21^2 + 2 k11 k12 k21 k22 + k11 k12 k22^2 + k11 k12 k21 km11 + k11 k12 k22 km11 +
   k11 k12 k21 km12 + k11 k12 k22 km12 + k12 k21 k22 km21 + k12 k22^2 km21 +
   k12 k21 km11 km21 + k12 k22 km11 km21 + k12 km11^2 km21 + k12 k21 km12 km21 +
   k12 k22 km12 km21 + k12 km11 km12 km21 + k11 k21^2 km22 + k11 k21 k22 km22 +
   k11 k21 km11 km22 + k11 k22 km11 km22 + k11 k21 km12 km22 + k11 k22 km12 km22 +
   k11 km11 km12 km22 + k11 km12^2 km22 + k21 km11 km21 km22 + k22 km11 km21 km22 +
   km11^2 km21 km22 + k21 km12 km21 km22 + k22 km12 km21 km22 + 2 km11 km12 km21 km22 +
   km12^2 km21 km22 + 2 k11 k12 k21 s + k11 k21^2 s + k12 k21^2 s + 2 k11 k12 k22 s +
   2 k11 k21 k22 s + 2 k12 k21 k22 s + k11 k22^2 s + k12 k22^2 s + k11 k12 km11 s +
   k11 k21 km11 s + 2 k12 k21 km11 s + k11 k22 km11 s + 2 k12 k22 km11 s + k12 km11^2 s +
   k11 k12 km12 s + 2 k11 k21 km12 s + k12 k21 km12 s + 2 k11 k22 km12 s + k12 k22 km12 s +
   k11 km11 km12 s + k12 km11 km12 s + k11 km12^2 s + k12 k21 km21 s + 2 k12 k22 km21 s +
   k21 k22 km21 s + k22^2 km21 s + 2 k12 km11 km21 s + k21 km11 km21 s + 2 k22 km11 km21 s +
   km11^2 km21 s + k12 km12 km21 s + k21 km12 km21 s + 2 k22 km12 km21 s +
   2 km11 km12 km21 s + km12^2 km21 s + 2 k11 k21 km22 s + k21^2 km22 s + k11 k22 km22 s +
   k21 k22 km22 s + k11 km11 km22 s + 2 k21 km11 km22 s + k22 km11 km22 s + km11^2 km22 s +
   2 k11 km12 km22 s + 2 k21 km12 km22 s + k22 km12 km22 s + 2 km11 km12 km22 s +
   km12^2 km22 s + k21 km21 km22 s + k22 km21 km22 s + 2 km11 km21 km22 s +
```

```
2 km12 km21 km22 s + k11 k12 s^2 + 2 k11 k21 s^2 + 2 k12 k21 s^2 + k21^2 s^2 + 2 k11 k22 s^2 +
2 k12 k22 s^2 + 2 k21 k22 s^2 + k22^2 s^2 + k11 km11 s^2 + 2 k12 km11 s^2 + 2 k21 km11 s^2 +
2 k22 km11 s^2 + km11^2 s^2 + 2 k11 km12 s^2 + k12 km12 s^2 + 2 k21 km12 s^2 + 2 k22 km12 s^2 +
2 km11 km12 s^2 + km12^2 s^2 + k12 km21 s^2 + k21 km21 s^2 + 2 k22 km21 s^2 + 2 km11 km21 s^2 +
2 km12 km21 s^2 + k11 km22 s^2 + 2 k21 km22 s^2 + k22 km22 s^2 + 2 km11 km22 s^2 +
2 km12 km22 s^2 + km21 km22 s^2 + k11 s^3 + k12 s^3 + 2 k21 s^3 + 2 k22 s^3 + 2 km11 s^3 +
2 km12 s^3 + km21 s^3 + km22 s^3 + s^4 + gammam1 (k21 + k22 + km11 + km12 + s)
  (km12 km21 + k21 s + k22 s + km12 s + km21 s + s^2 + k11 (k21 + k22 + s) + km11 (km21 + s)) +
gamma1 (k21 + k22 + km11 + km12 + s)
  (km12 km22 + k21 s + k22 s + km12 s + km22 s + s^2 + k12 (k21 + k22 + s) + km11 (km22 + s))),
(k22 (k11 k12 k21 + k11 k12 k22 + k11 k12 km11 + k11 k12 km12 + k12 k22 km21 +
   k12 km11 km21 + k12 km12 km21 + k11 k21 km22 + k11 k12 s +
   k12 k21 s + k12 k22 s + k12 km11 s + k12 km12 s + k12 km21 s + k12 s^2 +
   gammam1 k11 (k21 + k22 + km11 + km12 + s) + gamma1 k12 (k21 + k22 + km11 + km12 + s))) /
 (k11 k12 k21^2 + 2 k11 k12 k21 k22 + k11 k12 k22^2 + k11 k12 k21 km11 + k11 k12 k22 km11 +
  k11 k12 k21 km12 + k11 k12 k22 km12 + k12 k21 k22 km21 + k12 k22^2 km21 +
  k12 k21 km11 km21 + k12 k22 km11 km21 + k12 km11^2 km21 + k12 k21 km12 km21 +
  k12 k22 km12 km21 + k12 km11 km12 km21 + k11 k21^2 km22 + k11 k21 k22 km22 +
  k11 k21 km11 km22 + k11 k22 km11 km22 + k11 k21 km12 km22 + k11 k22 km12 km22 +
  k11 km11 km12 km22 + k11 km12^2 km22 + k21 km11 km21 km22 + k22 km11 km21 km22 +
  km11^2 km21 km22 + k21 km12 km21 km22 + k22 km12 km21 km22 + 2 km11 km12 km21 km22 +
  km12^2 km21 km22 + 2 k11 k12 k21 s + k11 k21^2 s + k12 k21^2 s + 2 k11 k12 k22 s +
  2 k11 k21 k22 s + 2 k12 k21 k22 s + k11 k22^2 s + k12 k22^2 s + k11 k12 km11 s +
  k11 k21 km11 s + 2 k12 k21 km11 s + k11 k22 km11 s + 2 k12 k22 km11 s + k12 km11^2 s +
  k11 k12 km12 s + 2 k11 k21 km12 s + k12 k21 km12 s + 2 k11 k22 km12 s + k12 k22 km12 s +
  k11 km11 km12 s + k12 km11 km12 s + k11 km12^2 s + k12 k21 km21 s + 2 k12 k22 km21 s +
  k21 k22 km21 s + k22^2 km21 s + 2 k12 km11 km21 s + k21 km11 km21 s + 2 k22 km11 km21 s +
  km11^2 km21 s + k12 km12 km21 s + k21 km12 km21 s + 2 k22 km12 km21 s +
  2 km11 km12 km21 s + km12^2 km21 s + 2 k11 k21 km22 s + k21^2 km22 s + k11 k22 km22 s +
  k21 k22 km22 s + k11 km11 km22 s + 2 k21 km11 km22 s + k22 km11 km22 s + km11^2 km22 s +
  2 k11 km12 km22 s + 2 k21 km12 km22 s + k22 km12 km22 s + 2 km11 km12 km22 s +
  km12^2 km22 s + k21 km21 km22 s + k22 km21 km22 s + 2 km11 km21 km22 s +
  2 km12 km21 km22 s + k11 k12 s^2 + 2 k11 k21 s^2 + 2 k12 k21 s^2 + k21^2 s^2 + 2 k11 k22 s^2 +
  2 k12 k22 s^2 + 2 k21 k22 s^2 + k22^2 s^2 + k11 km11 s^2 + 2 k12 km11 s^2 + 2 k21 km11 s^2 +
  2 k22 km11 s^2 + km11^2 s^2 + 2 k11 km12 s^2 + k12 km12 s^2 + 2 k21 km12 s^2 + 2 k22 km12 s^2 +
  2 km11 km12 s^2 + km12^2 s^2 + k12 km21 s^2 + k21 km21 s^2 + 2 k22 km21 s^2 + 2 km11 km21 s^2 +
  2 km12 km21 s^2 + k11 km22 s^2 + 2 k21 km22 s^2 + k22 km22 s^2 + 2 km11 km22 s^2 +
  2 km12 km22 s^2 + km21 km22 s^2 + k11 s^3 + k12 s^3 + 2 k21 s^3 + 2 k22 s^3 + 2 km11 s^3 +
  2 km12 s^3 + km21 s^3 + km22 s^3 + s^4 + gammam1 (k21 + k22 + km11 + km12 + s)
    (km12 km21 + k21 s + k22 s + km12 s + km21 s + s^2 + k11 (k21 + k22 + s) + km11 (km21 + s)) +
  gamma1 (k21 + k22 + km11 + km12 + s) (km12 km22 + k21 s + k22 s +
     km12 s + km22 s + s^2 + k12 (k21 + k22 + s) + km11 (km22 + s)))}}
```

In[29]:=
```
Omegaplus =
  Function[s, {{(k21 (k11 k12 k21 + k11 k12 k22 + k11 k12 km11 + k11 k12 km12 + k12 k22 km21 +
```

k11 k21 km22 + k11 km11 km22 + k11 km12 km22 + k11 k12 s + k11 k21 s +
k11 k22 s + k11 km11 s + k11 km12 s + k11 km22 s + k11 s$^2$ + gammam1 k11
(k21 + k22 + km11 + km12 + s) + gamma1 k12 (k21 + k22 + km11 + km12 + s))) /
(k11 k12 k21$^2$ + 2 k11 k12 k21 k22 + k11 k12 k22$^2$ + k11 k12 k21 km11 + k11 k12 k22 km11 +
k11 k12 k21 km12 + k11 k12 k22 km12 + k12 k21 k22 km21 + k12 k22$^2$ km21 +
k12 k21 km11 km21 + k12 k22 km11 km21 + k12 km11$^2$ km21 + k12 k21 km12 km21 +
k12 k22 km12 km21 + k12 km11 km12 km21 + k11 k21$^2$ km22 + k11 k21 k22 km22 +
k11 k21 km11 km22 + k11 k22 km11 km22 + k11 k21 km12 km22 + k11 k22 km12 km22 +
k11 km11 km12 km22 + k11 km12$^2$ km22 + k21 km11 km21 km22 + k22 km11 km21 km22 +
km11$^2$ km21 km22 + k21 km12 km21 km22 + k22 km12 km21 km22 + 2 km11 km12 km21 km22 +
km12$^2$ km21 km22 + 2 k11 k12 k21 s + k11 k21$^2$ s + k12 k21$^2$ s + 2 k11 k12 k22 s +
2 k11 k21 k22 s + 2 k12 k21 k22 s + k11 k22$^2$ s + k12 k22$^2$ s + k11 k12 km11 s +
k11 k21 km11 s + 2 k12 k21 km11 s + k11 k22 km11 s + 2 k12 k22 km11 s + k12 km11$^2$ s +
k11 k12 km12 s + 2 k11 k21 km12 s + k12 k21 km12 s + 2 k11 k22 km12 s + k12 k22 km12 s +
k11 km11 km12 s + k12 km11 km12 s + k11 km12$^2$ s + k12 k21 km21 s + 2 k12 k22 km21 s +
k21 k22 km21 s + k22$^2$ km21 s + 2 k12 km11 km21 s + k21 km11 km21 s + 2 k22 km11 km21 s +
km11$^2$ km21 s + k12 km12 km21 s + k21 km12 km21 s + 2 k22 km12 km21 s +
2 km11 km12 km21 s + km12$^2$ km21 s + 2 k11 k21 km22 s + k21$^2$ km22 s + k11 k22 km22 s +
k21 k22 km22 s + k11 km11 km22 s + 2 k21 km11 km22 s + k22 km11 km22 s + km11$^2$ km22 s +
2 k11 km12 km22 s + 2 k21 km12 km22 s + k22 km12 km22 s + 2 km11 km12 km22 s +
km12$^2$ km22 s + k21 km21 km22 s + k22 km21 km22 s + 2 km11 km21 km22 s +
2 km12 km21 km22 s + k11 k12 s$^2$ + 2 k11 k21 s$^2$ + 2 k12 k21 s$^2$ + k21$^2$ s$^2$ + 2 k11 k22 s$^2$ +
2 k12 k22 s$^2$ + 2 k21 k22 s$^2$ + k22$^2$ s$^2$ + k11 km11 s$^2$ + 2 k12 km11 s$^2$ + 2 k21 km11 s$^2$ +
2 k22 km11 s$^2$ + km11$^2$ s$^2$ + 2 k11 km12 s$^2$ + k12 km12 s$^2$ + 2 k21 km12 s$^2$ + 2 k22 km12 s$^2$ +
2 km11 km12 s$^2$ + km12$^2$ s$^2$ + k12 km21 s$^2$ + k21 km21 s$^2$ + 2 k22 km21 s$^2$ + 2 km11 km21 s$^2$ +
2 km12 km21 s$^2$ + k11 km22 s$^2$ + 2 k21 km22 s$^2$ + k22 km22 s$^2$ + 2 km11 km22 s$^2$ +
2 km12 km22 s$^2$ + km21 km22 s$^2$ + k11 s$^3$ + k12 s$^3$ + 2 k21 s$^3$ + 2 k22 s$^3$ + 2 km11 s$^3$ +
2 km12 s$^3$ + km21 s$^3$ + km22 s$^3$ + s$^4$ + gammam1 (k21 + k22 + km11 + km12 + s) (km12 km21 +
k21 s + k22 s + km12 s + km21 s + s$^2$ + k11 (k21 + k22 + s) + km11 (km21 + s)) +
gamma1 (k21 + k22 + km11 + km12 + s) (km12 km22 + k21 s + k22 s + km12 s +
km22 s + s$^2$ + k12 (k21 + k22 + s) + km11 (km22 + s))),
(k21 (k11 k12 k21 + k11 k12 k22 + k11 k12 km11 + k11 k12 km12 + k12 k22 km21 +
k12 km11 km21 + k12 km12 km21 + k11 k21 km22 + k11 k12 s + k12 k21 s +
k12 k22 s + k12 km11 s + k12 km12 s + k12 km21 s + k12 s$^2$ + gammam1 k11
(k21 + k22 + km11 + km12 + s) + gamma1 k12 (k21 + k22 + km11 + km12 + s))) /
(k11 k12 k21$^2$ + 2 k11 k12 k21 k22 + k11 k12 k22$^2$ + k11 k12 k21 km11 +
k11 k12 k22 km11 + k11 k12 k21 km12 + k11 k12 k22 km12 + k12 k21 k22 km21 +
k12 k22$^2$ km21 + k12 k21 km11 km21 + k12 k22 km11 km21 + k12 km11$^2$ km21 +
k12 k21 km12 km21 + k12 k22 km12 km21 + k12 km11 km12 km21 + k11 k21$^2$ km22 +
k11 k21 k22 km22 + k11 k21 km11 km22 + k11 k22 km11 km22 + k11 k21 km12 km22 +
k11 k22 km12 km22 + k11 km11 km12 km22 + k11 km12$^2$ km22 + k21 km11 km21 km22 +
k22 km11 km21 km22 + km11$^2$ km21 km22 + k21 km12 km21 km22 + k22 km12 km21 km22 +
2 km11 km12 km21 km22 + km12$^2$ km21 km22 + 2 k11 k12 k21 s + k11 k21$^2$ s +

```
k12 k21^2 s + 2 k11 k12 k22 s + 2 k11 k21 k22 s + 2 k12 k21 k22 s + k11 k22^2 s +
k12 k22^2 s + k11 k12 km11 s + k11 k21 km11 s + 2 k12 k21 km11 s + k11 k22 km11 s +
2 k12 k22 km11 s + k12 km11^2 s + k11 k12 km12 s + 2 k11 k21 km12 s + k12 k21 km12 s +
2 k11 k22 km12 s + k12 k22 km12 s + k11 km11 km12 s + k12 km11 km12 s +
k11 km12^2 s + k12 k21 km21 s + 2 k12 k22 km21 s + k21 k22 km21 s + k22^2 km21 s +
2 k12 km11 km21 s + k21 km11 km21 s + 2 k22 km11 km21 s + km11^2 km21 s +
k12 km12 km21 s + k21 km12 km21 s + 2 k22 km12 km21 s + 2 km11 km12 km21 s +
km12^2 km21 s + 2 k11 k21 km22 s + k21^2 km22 s + k11 k22 km22 s + k21 k22 km22 s +
k11 km11 km22 s + 2 k21 km11 km22 s + k22 km11 km22 s + km11^2 km22 s +
2 k11 km12 km22 s + 2 k21 km12 km22 s + k22 km12 km22 s + 2 km11 km12 km22 s +
km12^2 km22 s + k21 km21 km22 s + k22 km21 km22 s + 2 km11 km21 km22 s +
2 km12 km21 km22 s + k11 k12 s^2 + 2 k11 k21 s^2 + 2 k12 k21 s^2 + k21^2 s^2 + 2 k11 k22 s^2 +
2 k12 k22 s^2 + 2 k21 k22 s^2 + k22^2 s^2 + k11 km11 s^2 + 2 k12 km11 s^2 + 2 k21 km11 s^2 +
2 k22 km11 s^2 + km11^2 s^2 + 2 k11 km12 s^2 + k12 km12 s^2 + 2 k21 km12 s^2 + 2 k22 km12 s^2 +
2 km11 km12 s^2 + km12^2 s^2 + k12 km21 s^2 + k21 km21 s^2 + 2 k22 km21 s^2 + 2 km11 km21 s^2 +
2 km12 km21 s^2 + k11 km22 s^2 + 2 k21 km22 s^2 + k22 km22 s^2 + 2 km11 km22 s^2 +
2 km12 km22 s^2 + km21 km22 s^2 + k11 s^3 + k12 s^3 + 2 k21 s^3 + 2 k22 s^3 + 2 km11 s^3 +
2 km12 s^3 + km21 s^3 + km22 s^3 + s^4 + gammam1 (k21 + k22 + km11 + km12 + s) (km12 km21 +
   k21 s + k22 s + km12 s + km21 s + s^2 + k11 (k21 + k22 + s) + km11 (km21 + s)) +
gamma1 (k21 + k22 + km11 + km12 + s) (km12 km22 + k21 s + k22 s + km12 s +
   km22 s + s^2 + k12 (k21 + k22 + s) + km11 (km22 + s)))},
{(k22 (k11 k12 k21 + k11 k12 k22 + k11 k12 km11 + k11 k12 km12 + k12 k22 km21 +
     k11 k21 km22 + k11 km11 km22 + k11 km12 km22 + k11 k12 s + k11 k21 s +
     k11 k22 s + k11 km11 s + k11 km12 s + k11 km22 s + k11 s^2 + gammam1 k11
      (k21 + k22 + km11 + km12 + s) + gamma1 k12 (k21 + k22 + km11 + km12 + s))) /
  (k11 k12 k21^2 + 2 k11 k12 k21 k22 + k11 k12 k22^2 + k11 k12 k21 km11 +
   k11 k12 k22 km11 + k11 k12 k21 km12 + k11 k12 k22 km12 + k12 k21 k22 km21 +
   k12 k22^2 km21 + k12 k21 km11 km21 + k12 k22 km11 km21 + k12 km11^2 km21 +
   k12 k21 km12 km21 + k12 k22 km12 km21 + k12 km11 km12 km21 + k11 k21^2 km22 +
   k11 k21 k22 km22 + k11 k21 km11 km22 + k11 k22 km11 km22 + k11 k21 km12 km22 +
   k11 k22 km12 km22 + k11 km11 km12 km22 + k11 km12^2 km22 + k21 km11 km21 km22 +
   k22 km11 km21 km22 + km11^2 km21 km22 + k21 km12 km21 km22 + k22 km12 km21 km22 +
   2 km11 km12 km21 km22 + km12^2 km21 km22 + 2 k11 k12 k21 s + k11 k21^2 s +
   k12 k21^2 s + 2 k11 k12 k22 s + 2 k11 k21 k22 s + 2 k12 k21 k22 s + k11 k22^2 s +
   k12 k22^2 s + k11 k12 km11 s + k11 k21 km11 s + 2 k12 k21 km11 s + k11 k22 km11 s +
   2 k12 k22 km11 s + k12 km11^2 s + k11 k12 km12 s + 2 k11 k21 km12 s + k12 k21 km12 s +
   2 k11 k22 km12 s + k12 k22 km12 s + k11 km11 km12 s + k12 km11 km12 s +
   k11 km12^2 s + k12 k21 km21 s + 2 k12 k22 km21 s + k21 k22 km21 s + k22^2 km21 s +
   2 k12 km11 km21 s + k21 km11 km21 s + 2 k22 km11 km21 s + km11^2 km21 s +
   k12 km12 km21 s + k21 km12 km21 s + 2 k22 km12 km21 s + 2 km11 km12 km21 s +
   km12^2 km21 s + 2 k11 k21 km22 s + k21^2 km22 s + k11 k22 km22 s + k21 k22 km22 s +
   k11 km11 km22 s + 2 k21 km11 km22 s + k22 km11 km22 s + km11^2 km22 s +
   2 k11 km12 km22 s + 2 k21 km12 km22 s + k22 km12 km22 s + 2 km11 km12 km22 s +
```

Printed by Wolfram Mathematica Student Edition

km12$^{2}$ km22 s + k21 km21 km22 s + k22 km21 km22 s + 2 km11 km21 km22 s +
2 km12 km21 km22 s + k11 k12 s$^{2}$ + 2 k11 k21 s$^{2}$ + 2 k12 k21 s$^{2}$ + k21$^{2}$ s$^{2}$ + 2 k11 k22 s$^{2}$ +
2 k12 k22 s$^{2}$ + 2 k21 k22 s$^{2}$ + k22$^{2}$ s$^{2}$ + k11 km11 s$^{2}$ + 2 k12 km11 s$^{2}$ + 2 k21 km11 s$^{2}$ +
2 k22 km11 s$^{2}$ + km11$^{2}$ s$^{2}$ + 2 k11 km12 s$^{2}$ + k12 km12 s$^{2}$ + 2 k21 km12 s$^{2}$ + 2 k22 km12 s$^{2}$ +
2 km11 km12 s$^{2}$ + km12$^{2}$ s$^{2}$ + k12 km21 s$^{2}$ + k21 km21 s$^{2}$ + 2 k22 km21 s$^{2}$ + 2 km11 km21 s$^{2}$ +
2 km12 km21 s$^{2}$ + k11 km22 s$^{2}$ + 2 k21 km22 s$^{2}$ + k22 km22 s$^{2}$ + 2 km11 km22 s$^{2}$ +
2 km12 km22 s$^{2}$ + km21 km22 s$^{2}$ + k11 s$^{3}$ + k12 s$^{3}$ + 2 k21 s$^{3}$ + 2 k22 s$^{3}$ + 2 km11 s$^{3}$ +
2 km12 s$^{3}$ + km21 s$^{3}$ + km22 s$^{3}$ + s$^{4}$ + gammam1 (k21 + k22 + km11 + km12 + s) (km12 km21 +
k21 s + k22 s + km12 s + km21 s + s$^{2}$ + k11 (k21 + k22 + s) + km11 (km21 + s)) +
gamma1 (k21 + k22 + km11 + km12 + s) (km12 km22 + k21 s + k22 s + km12 s +
km22 s + s$^{2}$ + k12 (k21 + k22 + s) + km11 (km22 + s))),
(k22 (k11 k12 k21 + k11 k12 k22 + k11 k12 km11 + k11 k12 km12 + k12 k22 km21 +
k12 km11 km21 + k12 km12 km21 + k11 k21 km22 + k11 k12 s + k12 k21 s +
k12 k22 s + k12 km11 s + k12 km12 s + k12 km21 s + k12 s$^{2}$ + gammam1 k11
(k21 + k22 + km11 + km12 + s) + gamma1 k12 (k21 + k22 + km11 + km12 + s))) /
(k11 k12 k21$^{2}$ + 2 k11 k12 k21 k22 + k11 k12 k22$^{2}$ + k11 k12 k21 km11 +
k11 k12 k22 km11 + k11 k12 k21 km12 + k11 k12 k22 km12 + k12 k21 k22 km21 +
k12 k22$^{2}$ km21 + k12 k21 km11 km21 + k12 k22 km11 km21 + k12 km11$^{2}$ km21 +
k12 k21 km12 km21 + k12 k22 km12 km21 + k12 km11 km12 km21 + k11 k21$^{2}$ km22 +
k11 k21 k22 km22 + k11 k21 km11 km22 + k11 k22 km11 km22 + k11 k21 km12 km22 +
k11 k22 km12 km22 + k11 km11 km12 km22 + k11 km12$^{2}$ km22 + k21 km11 km21 km22 +
k22 km11 km21 km22 + km11$^{2}$ km21 km22 + k21 km12 km21 km22 + k22 km12 km21 km22 +
2 km11 km12 km21 km22 + km12$^{2}$ km21 km22 + 2 k11 k12 k21 s + k11 k21$^{2}$ s +
k12 k21$^{2}$ s + 2 k11 k12 k22 s + 2 k11 k21 k22 s + 2 k12 k21 k22 s + k11 k22$^{2}$ s +
k12 k22$^{2}$ s + k11 k12 km11 s + k11 k21 km11 s + 2 k12 k21 km11 s + k11 k22 km11 s +
2 k12 k22 km11 s + k12 km11$^{2}$ s + k11 k12 km12 s + 2 k11 k21 km12 s + k12 k21 km12 s +
2 k11 k22 km12 s + k12 k22 km12 s + k11 km11 km12 s + k12 km11 km12 s +
k11 km12$^{2}$ s + k12 k21 km21 s + 2 k12 k22 km21 s + k21 k22 km21 s + k22$^{2}$ km21 s +
2 k12 km11 km21 s + k21 km11 km21 s + 2 k22 km11 km21 s + km11$^{2}$ km21 s +
k12 km12 km21 s + k21 km12 km21 s + 2 k22 km12 km21 s + 2 km11 km12 km21 s +
km12$^{2}$ km21 s + 2 k11 k21 km22 s + k21$^{2}$ km22 s + k11 k22 km22 s + k21 k22 km22 s +
k11 km11 km22 s + 2 k21 km11 km22 s + k22 km11 km22 s + km11$^{2}$ km22 s +
2 k11 km12 km22 s + 2 k21 km12 km22 s + k22 km12 km22 s + 2 km11 km12 km22 s +
km12$^{2}$ km22 s + k21 km21 km22 s + k22 km21 km22 s + 2 km11 km21 km22 s +
2 km12 km21 km22 s + k11 k12 s$^{2}$ + 2 k11 k21 s$^{2}$ + 2 k12 k21 s$^{2}$ + k21$^{2}$ s$^{2}$ + 2 k11 k22 s$^{2}$ +
2 k12 k22 s$^{2}$ + 2 k21 k22 s$^{2}$ + k22$^{2}$ s$^{2}$ + k11 km11 s$^{2}$ + 2 k12 km11 s$^{2}$ + 2 k21 km11 s$^{2}$ +
2 k22 km11 s$^{2}$ + km11$^{2}$ s$^{2}$ + 2 k11 km12 s$^{2}$ + k12 km12 s$^{2}$ + 2 k21 km12 s$^{2}$ + 2 k22 km12 s$^{2}$ +
2 km11 km12 s$^{2}$ + km12$^{2}$ s$^{2}$ + k12 km21 s$^{2}$ + k21 km21 s$^{2}$ + 2 k22 km21 s$^{2}$ + 2 km11 km21 s$^{2}$ +
2 km12 km21 s$^{2}$ + k11 km22 s$^{2}$ + 2 k21 km22 s$^{2}$ + k22 km22 s$^{2}$ + 2 km11 km22 s$^{2}$ +
2 km12 km22 s$^{2}$ + km21 km22 s$^{2}$ + k11 s$^{3}$ + k12 s$^{3}$ + 2 k21 s$^{3}$ + 2 k22 s$^{3}$ + 2 km11 s$^{3}$ +
2 km12 s$^{3}$ + km21 s$^{3}$ + km22 s$^{3}$ + s$^{4}$ + gammam1 (k21 + k22 + km11 + km12 + s) (km12 km21 +
k21 s + k22 s + km12 s + km21 s + s$^{2}$ + k11 (k21 + k22 + s) + km11 (km21 + s)) +

```
gamma1 (k21 + k22 + km11 + km12 + s) (km12 km22 + k21 s + k22 s + km12 s +
    km22 s + s^2 + k12 (k21 + k22 + s) + km11 (km22 + s)))}}]
```

Out[29]=

```
Function[s,
 {{(k21 (k11 k12 k21 + k11 k12 k22 + k11 k12 km11 + k11 k12 km12 + k12 k22 km21 + k11 k21 km22 +
        k11 km11 km22 + k11 km12 km22 + k11 k12 s + k11 k21 s +
        k11 k22 s + k11 km11 s + k11 km12 s + k11 km22 s + k11 s^2 +
        gammam1 k11 (k21 + k22 + km11 + km12 + s) + gamma1 k12 (k21 + k22 + km11 + km12 + s))) /
    (k11 k12 k21^2 + 2 k11 k12 k21 k22 + k11 k12 k22^2 + k11 k12 k21 km11 + k11 k12 k22 km11 +
      k11 k12 k21 km12 + k11 k12 k22 km12 + k12 k21 k22 km21 + k12 k22^2 km21 +
      k12 k21 km11 km21 + k12 k22 km11 km21 + k12 km11^2 km21 + k12 k21 km12 km21 +
      k12 k22 km12 km21 + k12 km11 km12 km21 + k11 k21^2 km22 + k11 k21 k22 km22 +
      k11 k21 km11 km22 + k11 k22 km11 km22 + k11 k21 km12 km22 + k11 k22 km12 km22 +
      k11 km11 km12 km22 + k11 km12^2 km22 + k21 km11 km21 km22 + k22 km11 km21 km22 +
      km11^2 km21 km22 + k21 km12 km21 km22 + k22 km12 km21 km22 + 2 km11 km12 km21 km22 +
      km12^2 km21 km22 + 2 k11 k12 k21 s + k11 k21^2 s + k12 k21^2 s + 2 k11 k12 k22 s +
      2 k11 k21 k22 s + 2 k12 k21 k22 s + k11 k22^2 s + k12 k22^2 s + k11 k12 km11 s +
      k11 k21 km11 s + 2 k12 k21 km11 s + k11 k22 km11 s + 2 k12 k22 km11 s + k12 km11^2 s +
      k11 k12 km12 s + 2 k11 k21 km12 s + k12 k21 km12 s + 2 k11 k22 km12 s + k12 k22 km12 s +
      k11 km11 km12 s + k12 km11 km12 s + k11 km12^2 s + k12 k21 km21 s + 2 k12 k22 km21 s +
      k21 k22 km21 s + k22^2 km21 s + 2 k12 km11 km21 s + k21 km11 km21 s + 2 k22 km11 km21 s +
      km11^2 km21 s + k12 km12 km21 s + k21 km12 km21 s + 2 k22 km12 km21 s +
      2 km11 km12 km21 s + km12^2 km21 s + 2 k11 k21 km22 s + k21^2 km22 s + k11 k22 km22 s +
      k21 k22 km22 s + k11 km11 km22 s + 2 k21 km11 km22 s + k22 km11 km22 s + km11^2 km22 s +
      2 k11 km12 km22 s + 2 k21 km12 km22 s + k22 km12 km22 s + 2 km11 km12 km22 s +
      km12^2 km22 s + k21 km21 km22 s + k22 km21 km22 s + 2 km11 km21 km22 s +
      2 km12 km21 km22 s + k11 k12 s^2 + 2 k11 k21 s^2 + 2 k12 k21 s^2 + k21^2 s^2 + 2 k11 k22 s^2 +
      2 k12 k22 s^2 + 2 k21 k22 s^2 + k22^2 s^2 + k11 km11 s^2 + 2 k12 km11 s^2 + 2 k21 km11 s^2 +
      2 k22 km11 s^2 + km11^2 s^2 + 2 k11 km12 s^2 + k12 km12 s^2 + 2 k21 km12 s^2 + 2 k22 km12 s^2 +
      2 km11 km12 s^2 + km12^2 s^2 + k12 km21 s^2 + k21 km21 s^2 + 2 k22 km21 s^2 + 2 km11 km21 s^2 +
      2 km12 km21 s^2 + k11 km22 s^2 + 2 k21 km22 s^2 + k22 km22 s^2 + 2 km11 km22 s^2 +
      2 km12 km22 s^2 + km21 km22 s^2 + k11 s^3 + k12 s^3 + 2 k21 s^3 + 2 k22 s^3 + 2 km11 s^3 +
      2 km12 s^3 + km21 s^3 + km22 s^3 + s^4 + gammam1 (k21 + k22 + km11 + km12 + s)
        (km12 km21 + k21 s + k22 s + km12 s + km21 s + s^2 + k11 (k21 + k22 + s) + km11 (km21 + s)) +
      gamma1 (k21 + k22 + km11 + km12 + s) (km12 km22 + k21 s + k22 s +
          km12 s + km22 s + s^2 + k12 (k21 + k22 + s) + km11 (km22 + s))),
   (k21 (k11 k12 k21 + k11 k12 k22 + k11 k12 km11 + k11 k12 km12 + k12 k22 km21 +
        k12 km11 km21 + k12 km12 km21 + k11 k21 km22 + k11 k12 s +
        k12 k21 s + k12 k22 s + k12 km11 s + k12 km12 s + k12 km21 s + k12 s^2 +
        gammam1 k11 (k21 + k22 + km11 + km12 + s) + gamma1 k12 (k21 + k22 + km11 + km12 + s))) /
    (k11 k12 k21^2 + 2 k11 k12 k21 k22 + k11 k12 k22^2 + k11 k12 k21 km11 + k11 k12 k22 km11 +
      k11 k12 k21 km12 + k11 k12 k22 km12 + k12 k21 k22 km21 + k12 k22^2 km21 +
      k12 k21 km11 km21 + k12 k22 km11 km21 + k12 km11^2 km21 + k12 k21 km12 km21 +
```

```
k12 k22 km12 km21 + k12 km11 km12 km21 + k11 k21^2 km22 + k11 k21 k22 km22 +
k11 k21 km11 km22 + k11 k22 km11 km22 + k11 k21 km12 km22 + k11 k22 km12 km22 +
k11 km11 km12 km22 + k11 km12^2 km22 + k21 km11 km21 km22 + k22 km11 km21 km22 +
km11^2 km21 km22 + k21 km12 km21 km22 + k22 km12 km21 km22 + 2 km11 km12 km21 km22 +
km12^2 km21 km22 + 2 k11 k12 k21 s + k11 k21^2 s + k12 k21^2 s + 2 k11 k12 k22 s +
2 k11 k21 k22 s + 2 k12 k21 k22 s + k11 k22^2 s + k12 k22^2 s + k11 k12 km11 s +
k11 k21 km11 s + 2 k12 k21 km11 s + k11 k22 km11 s + 2 k12 k22 km11 s + k12 km11^2 s +
k11 k12 km12 s + 2 k11 k21 km12 s + k12 k21 km12 s + 2 k11 k22 km12 s + k12 k22 km12 s +
k11 km11 km12 s + k12 km11 km12 s + k11 km12^2 s + k12 k21 km21 s + 2 k12 k22 km21 s +
k21 k22 km21 s + k22^2 km21 s + 2 k12 km11 km21 s + k21 km11 km21 s + 2 k22 km11 km21 s +
km11^2 km21 s + k12 km12 km21 s + k21 km12 km21 s + 2 k22 km12 km21 s +
2 km11 km12 km21 s + km12^2 km21 s + 2 k11 k21 km22 s + k21^2 km22 s + k11 k22 km22 s +
k21 k22 km22 s + k11 km11 km22 s + 2 k21 km11 km22 s + k22 km11 km22 s + km11^2 km22 s +
2 k11 km12 km22 s + 2 k21 km12 km22 s + k22 km12 km22 s + 2 km11 km12 km22 s +
km12^2 km22 s + k21 km21 km22 s + k22 km21 km22 s + 2 km11 km21 km22 s +
2 km12 km21 km22 s + k11 k12 s^2 + 2 k11 k21 s^2 + 2 k12 k21 s^2 + k21^2 s^2 + 2 k11 k22 s^2 +
2 k12 k22 s^2 + 2 k21 k22 s^2 + k22^2 s^2 + k11 km11 s^2 + 2 k12 km11 s^2 + 2 k21 km11 s^2 +
2 k22 km11 s^2 + km11^2 s^2 + 2 k11 km12 s^2 + k12 km12 s^2 + 2 k21 km12 s^2 + 2 k22 km12 s^2 +
2 km11 km12 s^2 + km12^2 s^2 + k12 km21 s^2 + k21 km21 s^2 + 2 k22 km21 s^2 + 2 km11 km21 s^2 +
2 km12 km21 s^2 + k11 km22 s^2 + 2 k21 km22 s^2 + k22 km22 s^2 + 2 km11 km22 s^2 +
2 km12 km22 s^2 + km21 km22 s^2 + k11 s^3 + k12 s^3 + 2 k21 s^3 + 2 k22 s^3 + 2 km11 s^3 +
2 km12 s^3 + km21 s^3 + km22 s^3 + s^4 + gammam1 (k21 + k22 + km11 + km12 + s)
  (km12 km21 + k21 s + k22 s + km12 s + km21 s + s^2 + k11 (k21 + k22 + s) + km11 (km21 + s)) +
gamma1 (k21 + k22 + km11 + km12 + s) (km12 km22 + k21 s + k22 s +
    km12 s + km22 s + s^2 + k12 (k21 + k22 + s) + km11 (km22 + s)))},
{(k22 (k11 k12 k21 + k11 k12 k22 + k11 k12 km11 + k11 k12 km12 + k12 k22 km21 +
     k11 k21 km22 + k11 km11 km22 + k11 km12 km22 + k11 k12 s +
     k11 k21 s + k11 k22 s + k11 km11 s + k11 km12 s + k11 km22 s + k11 s^2 +
     gammam1 k11 (k21 + k22 + km11 + km12 + s) + gamma1 k12 (k21 + k22 + km11 + km12 + s))) /
 (k11 k12 k21^2 + 2 k11 k12 k21 k22 + k11 k12 k22^2 + k11 k12 k21 km11 + k11 k12 k22 km11 +
  k11 k12 k21 km12 + k11 k12 k22 km12 + k12 k21 k22 km21 + k12 k22^2 km21 +
  k12 k21 km11 km21 + k12 k22 km11 km21 + k12 km11^2 km21 + k12 k21 km12 km21 +
  k12 k22 km12 km21 + k12 km11 km12 km21 + k11 k21^2 km22 + k11 k21 k22 km22 +
  k11 k21 km11 km22 + k11 k22 km11 km22 + k11 k21 km12 km22 + k11 k22 km12 km22 +
  k11 km11 km12 km22 + k11 km12^2 km22 + k21 km11 km21 km22 + k22 km11 km21 km22 +
  km11^2 km21 km22 + k21 km12 km21 km22 + k22 km12 km21 km22 + 2 km11 km12 km21 km22 +
  km12^2 km21 km22 + 2 k11 k12 k21 s + k11 k21^2 s + k12 k21^2 s + 2 k11 k12 k22 s +
  2 k11 k21 k22 s + 2 k12 k21 k22 s + k11 k22^2 s + k12 k22^2 s + k11 k12 km11 s +
  k11 k21 km11 s + 2 k12 k21 km11 s + k11 k22 km11 s + 2 k12 k22 km11 s + k12 km11^2 s +
  k11 k12 km12 s + 2 k11 k21 km12 s + k12 k21 km12 s + 2 k11 k22 km12 s + k12 k22 km12 s +
  k11 km11 km12 s + k12 km11 km12 s + k11 km12^2 s + k12 k21 km21 s + 2 k12 k22 km21 s +
  k21 k22 km21 s + k22^2 km21 s + 2 k12 km11 km21 s + k21 km11 km21 s + 2 k22 km11 km21 s +
  km11^2 km21 s + k12 km12 km21 s + k21 km12 km21 s + 2 k22 km12 km21 s +
```

$$2\ km11\ km12\ km21\ s + km12^2\ km21\ s + 2\ k11\ k21\ km22\ s + k21^2\ km22\ s + k11\ k22\ km22\ s +$$
$$k21\ k22\ km22\ s + k11\ km11\ km22\ s + 2\ k21\ km11\ km22\ s + k22\ km11\ km22\ s + km11^2\ km22\ s +$$
$$2\ k11\ km12\ km22\ s + 2\ k21\ km12\ km22\ s + k22\ km12\ km22\ s + 2\ km11\ km12\ km22\ s +$$
$$km12^2\ km22\ s + k21\ km21\ km22\ s + k22\ km21\ km22\ s + 2\ km11\ km21\ km22\ s +$$
$$2\ km12\ km21\ km22\ s + k11\ k12\ s^2 + 2\ k11\ k21\ s^2 + 2\ k12\ k21\ s^2 + k21^2\ s^2 + 2\ k11\ k22\ s^2 +$$
$$2\ k12\ k22\ s^2 + 2\ k21\ k22\ s^2 + k22^2\ s^2 + k11\ km11\ s^2 + 2\ k12\ km11\ s^2 + 2\ k21\ km11\ s^2 +$$
$$2\ k22\ km11\ s^2 + km11^2\ s^2 + 2\ k11\ km12\ s^2 + k12\ km12\ s^2 + 2\ k21\ km12\ s^2 + 2\ k22\ km12\ s^2 +$$
$$2\ km11\ km12\ s^2 + km12^2\ s^2 + k12\ km21\ s^2 + k21\ km21\ s^2 + 2\ k22\ km21\ s^2 + 2\ km11\ km21\ s^2 +$$
$$2\ km12\ km21\ s^2 + k11\ km22\ s^2 + 2\ k21\ km22\ s^2 + k22\ km22\ s^2 + 2\ km11\ km22\ s^2 +$$
$$2\ km12\ km22\ s^2 + km21\ km22\ s^2 + k11\ s^3 + k12\ s^3 + 2\ k21\ s^3 + 2\ k22\ s^3 + 2\ km11\ s^3 +$$
$$2\ km12\ s^3 + km21\ s^3 + km22\ s^3 + s^4 + gammam1\ (k21 + k22 + km11 + km12 + s)$$
$$(km12\ km21 + k21\ s + k22\ s + km12\ s + km21\ s + s^2 + k11\ (k21 + k22 + s) + km11\ (km21 + s)) +$$
$$gamma1\ (k21 + k22 + km11 + km12 + s)\ (km12\ km22 + k21\ s + k22\ s +$$
$$km12\ s + km22\ s + s^2 + k12\ (k21 + k22 + s) + km11\ (km22 + s))),$$
$$(k22\ (k11\ k12\ k21 + k11\ k12\ k22 + k11\ k12\ km11 + k11\ k12\ km12 + k12\ k22\ km21 +$$
$$k12\ km11\ km21 + k12\ km12\ km21 + k11\ k21\ km22 + k11\ k12\ s +$$
$$k12\ k21\ s + k12\ k22\ s + k12\ km11\ s + k12\ km12\ s + k12\ km21\ s + k12\ s^2 +$$
$$gammam1\ k11\ (k21 + k22 + km11 + km12 + s) + gamma1\ k12\ (k21 + k22 + km11 + km12 + s)))\ /$$
$$(k11\ k12\ k21^2 + 2\ k11\ k12\ k21\ k22 + k11\ k12\ k22^2 + k11\ k12\ k21\ km11 +$$
$$k11\ k12\ k22\ km11 + k11\ k12\ k21\ km12 + k11\ k12\ k22\ km12 + k12\ k21\ k22\ km21 +$$
$$k12\ k22^2\ km21 + k12\ k21\ km11\ km21 + k12\ k22\ km11\ km21 + k12\ km11^2\ km21 +$$
$$k12\ k21\ km12\ km21 + k12\ k22\ km12\ km21 + k12\ km11\ km12\ km21 + k11\ k21^2\ km22 +$$
$$k11\ k21\ k22\ km22 + k11\ k21\ km11\ km22 + k11\ k22\ km11\ km22 + k11\ k21\ km12\ km22 +$$
$$k11\ k22\ km12\ km22 + k11\ km11\ km12\ km22 + k11\ km12^2\ km22 + k21\ km11\ km21\ km22 +$$
$$k22\ km11\ km21\ km22 + km11^2\ km21\ km22 + k21\ km12\ km21\ km22 + k22\ km12\ km21\ km22 +$$
$$2\ km11\ km12\ km21\ km22 + km12^2\ km21\ km22 + 2\ k11\ k12\ k21\ s + k11\ k21^2\ s +$$
$$k12\ k21^2\ s + 2\ k11\ k12\ k22\ s + 2\ k11\ k21\ k22\ s + 2\ k12\ k21\ k22\ s + k11\ k22^2\ s +$$
$$k12\ k22^2\ s + k11\ k12\ km11\ s + k11\ k21\ km11\ s + 2\ k12\ k21\ km11\ s + k11\ k22\ km11\ s +$$
$$2\ k12\ k22\ km11\ s + k12\ km11^2\ s + k11\ k12\ km12\ s + 2\ k11\ k21\ km12\ s + k12\ k21\ km12\ s +$$
$$2\ k11\ k22\ km12\ s + k12\ k22\ km12\ s + k11\ km11\ km12\ s + k12\ km11\ km12\ s +$$
$$k11\ km12^2\ s + k12\ k21\ km21\ s + 2\ k12\ k22\ km21\ s + k21\ k22\ km21\ s + k22^2\ km21\ s +$$
$$2\ k12\ km11\ km21\ s + k21\ km11\ km21\ s + 2\ k22\ km11\ km21\ s + km11^2\ km21\ s +$$
$$k12\ km12\ km21\ s + k21\ km12\ km21\ s + 2\ k22\ km12\ km21\ s + 2\ km11\ km12\ km21\ s +$$
$$km12^2\ km21\ s + 2\ k11\ k21\ km22\ s + k21^2\ km22\ s + k11\ k22\ km22\ s + k21\ k22\ km22\ s +$$
$$k11\ km11\ km22\ s + 2\ k21\ km11\ km22\ s + k22\ km11\ km22\ s + km11^2\ km22\ s +$$
$$2\ k11\ km12\ km22\ s + 2\ k21\ km12\ km22\ s + k22\ km12\ km22\ s + 2\ km11\ km12\ km22\ s +$$
$$km12^2\ km22\ s + k21\ km21\ km22\ s + k22\ km21\ km22\ s + 2\ km11\ km21\ km22\ s +$$
$$2\ km12\ km21\ km22\ s + k11\ k12\ s^2 + 2\ k11\ k21\ s^2 + 2\ k12\ k21\ s^2 + k21^2\ s^2 + 2\ k11\ k22\ s^2 +$$
$$2\ k12\ k22\ s^2 + 2\ k21\ k22\ s^2 + k22^2\ s^2 + k11\ km11\ s^2 + 2\ k12\ km11\ s^2 + 2\ k21\ km11\ s^2 +$$
$$2\ k22\ km11\ s^2 + km11^2\ s^2 + 2\ k11\ km12\ s^2 + k12\ km12\ s^2 + 2\ k21\ km12\ s^2 + 2\ k22\ km12\ s^2 +$$
$$2\ km11\ km12\ s^2 + km12^2\ s^2 + k12\ km21\ s^2 + k21\ km21\ s^2 + 2\ k22\ km21\ s^2 + 2\ km11\ km21\ s^2 +$$
$$2\ km12\ km21\ s^2 + k11\ km22\ s^2 + 2\ k21\ km22\ s^2 + k22\ km22\ s^2 + 2\ km11\ km22\ s^2 +$$
$$2\ km12\ km22\ s^2 + km21\ km22\ s^2 + k11\ s^3 + k12\ s^3 + 2\ k21\ s^3 + 2\ k22\ s^3 + 2\ km11\ s^3 +$$

```
      2 km12 s^3 + km21 s^3 + km22 s^3 + s^4 + gammam1 (k21 + k22 + km11 + km12 + s)
        (km12 km21 + k21 s + k22 s + km12 s + km21 s + s^2 + k11 (k21 + k22 + s) + km11 (km21 + s)) +
      gamma1 (k21 + k22 + km11 + km12 + s) (km12 km22 + k21 s + k22 s +
          km12 s + km22 s + s^2 + k12 (k21 + k22 + s) + km11 (km22 + s)))}}]
```

```
In[30]:= Simplify[Together[Omegaminusfunc[s]]]
Out[30]=
{{(km11 (gamma1 k21 km22 + gamma1 k22 km22 + gamma1 km11 km22 + gamma1 km12 km22 +
        k11 km12 km22 + k21 km21 km22 + k22 km21 km22 + km11 km21 km22 + km12 km21 km22 +
        k21 km21 s + k22 km21 s + km11 km21 s + km12 km21 s + gamma1 km22 s + km21 km22 s +
        km21 s^2 + k12 km21 (k21 + k22 + km11 + s) + gammam1 km21 (k21 + k22 + km11 + km12 + s))) /
   (k11 k12 k21^2 + 2 k11 k12 k21 k22 + k11 k12 k22^2 + k11 k12 k21 km11 + k11 k12 k22 km11 +
     k11 k12 k21 km12 + k11 k12 k22 km12 + k12 k21 k22 km21 + k12 k22^2 km21 +
     k12 k21 km11 km21 + k12 k22 km11 km21 + k12 km11^2 km21 + k12 k21 km12 km21 +
     k12 k22 km12 km21 + k12 km11 km12 km21 + k11 k21^2 km22 + k11 k21 k22 km22 +
     k11 k21 km11 km22 + k11 k22 km11 km22 + k11 k21 km12 km22 + k11 k22 km12 km22 +
     k11 km11 km12 km22 + k11 km12^2 km22 + k21 km11 km21 km22 + k22 km11 km21 km22 +
     km11^2 km21 km22 + k21 km12 km21 km22 + k22 km12 km21 km22 + 2 km11 km12 km21 km22 +
     km12^2 km21 km22 + 2 k11 k12 k21 s + k11 k21^2 s + k12 k21^2 s + 2 k11 k12 k22 s +
     2 k11 k21 k22 s + 2 k12 k21 k22 s + k11 k22^2 s + k12 k22^2 s + k11 k12 km11 s +
     k11 k21 km11 s + 2 k12 k21 km11 s + k11 k22 km11 s + 2 k12 k22 km11 s + k12 km11^2 s +
     k11 k12 km12 s + 2 k11 k21 km12 s + k12 k21 km12 s + 2 k11 k22 km12 s + k12 k22 km12 s +
     k11 km11 km12 s + k12 km11 km12 s + k11 km12^2 s + k12 k21 km21 s + 2 k12 k22 km21 s +
     k21 k22 km21 s + k22^2 km21 s + 2 k12 km11 km21 s + k21 km11 km21 s + 2 k22 km11 km21 s +
     km11^2 km21 s + k12 km12 km21 s + k21 km12 km21 s + 2 k22 km12 km21 s +
     2 km11 km12 km21 s + km12^2 km21 s + 2 k11 k21 km22 s + k21^2 km22 s + k11 k22 km22 s +
     k21 k22 km22 s + k11 km11 km22 s + 2 k21 km11 km22 s + k22 km11 km22 s + km11^2 km22 s +
     2 k11 km12 km22 s + 2 k21 km12 km22 s + k22 km12 km22 s + 2 km11 km12 km22 s +
     km12^2 km22 s + k21 km21 km22 s + k22 km21 km22 s + 2 km11 km21 km22 s +
     2 km12 km21 km22 s + k11 k12 s^2 + 2 k11 k21 s^2 + 2 k12 k21 s^2 + k21^2 s^2 + 2 k11 k22 s^2 +
     2 k12 k22 s^2 + 2 k21 k22 s^2 + k22^2 s^2 + k11 km11 s^2 + 2 k12 km11 s^2 + 2 k21 km11 s^2 +
     2 k22 km11 s^2 + km11^2 s^2 + 2 k11 km12 s^2 + k12 km12 s^2 + 2 k21 km12 s^2 + 2 k22 km12 s^2 +
     2 km11 km12 s^2 + km12^2 s^2 + k12 km21 s^2 + k21 km21 s^2 + 2 k22 km21 s^2 + 2 km11 km21 s^2 +
     2 km12 km21 s^2 + k11 km22 s^2 + 2 k21 km22 s^2 + k22 km22 s^2 + 2 km11 km22 s^2 +
     2 km12 km22 s^2 + km21 km22 s^2 + k11 s^3 + k12 s^3 + 2 k21 s^3 + 2 k22 s^3 + 2 km11 s^3 +
     2 km12 s^3 + km21 s^3 + km22 s^3 + s^4 + gammam1 (k21 + k22 + km11 + km12 + s)
       (km12 km21 + k21 s + k22 s + km12 s + km21 s + s^2 + k11 (k21 + k22 + s) + km11 (km21 + s)) +
     gamma1 (k21 + k22 + km11 + km12 + s)
       (km12 km22 + k21 s + k22 s + km12 s + km22 s + s^2 + k12 (k21 + k22 + s) + km11 (km22 + s))),
  (km11 (k12 km11 km21 + gammam1 km21 (k21 + k22 + km11 + km12 + s) +
        km22 (k11 (k21 + k22 + km12 + s) + gamma1 (k21 + k22 + km11 + km12 + s) +
            (k21 + k22 + km11 + km12 + s) (km21 + s)))) /
   (k11 k12 k21^2 + 2 k11 k12 k21 k22 + k11 k12 k22^2 + k11 k12 k21 km11 + k11 k12 k22 km11 +
```

```
k11 k12 k21 km12 + k11 k12 k22 km12 + k12 k21 k22 km21 + k12 k22^2 km21 +
k12 k21 km11 km21 + k12 k22 km11 km21 + k12 km11^2 km21 + k12 k21 km12 km21 +
k12 k22 km12 km21 + k12 km11 km12 km21 + k11 k21^2 km22 + k11 k21 k22 km22 +
k11 k21 km11 km22 + k11 k22 km11 km22 + k11 k21 km12 km22 + k11 k22 km12 km22 +
k11 km11 km12 km22 + k11 km12^2 km22 + k21 km11 km21 km22 + k22 km11 km21 km22 +
km11^2 km21 km22 + k21 km12 km21 km22 + k22 km12 km21 km22 + 2 km11 km12 km21 km22 +
km12^2 km21 km22 + 2 k11 k12 k21 s + k11 k21^2 s + k12 k21^2 s + 2 k11 k12 k22 s +
2 k11 k21 k22 s + 2 k12 k21 k22 s + k11 k22^2 s + k12 k22^2 s + k11 k12 km11 s +
k11 k21 km11 s + 2 k12 k21 km11 s + k11 k22 km11 s + 2 k12 k22 km11 s + k12 km11^2 s +
k11 k12 km12 s + 2 k11 k21 km12 s + k12 k21 km12 s + 2 k11 k22 km12 s + k12 k22 km12 s +
k11 km11 km12 s + k12 km11 km12 s + k11 km12^2 s + k12 k21 km21 s + 2 k12 k22 km21 s +
k21 k22 km21 s + k22^2 km21 s + 2 k12 km11 km21 s + k21 km11 km21 s + 2 k22 km11 km21 s +
km11^2 km21 s + k12 km12 km21 s + k21 km12 km21 s + 2 k22 km12 km21 s +
2 km11 km12 km21 s + km12^2 km21 s + 2 k11 k21 km22 s + k21^2 km22 s + k11 k22 km22 s +
k21 k22 km22 s + k11 km11 km22 s + 2 k21 km11 km22 s + k22 km11 km22 s + km11^2 km22 s +
2 k11 km12 km22 s + 2 k21 km12 km22 s + k22 km12 km22 s + 2 km11 km12 km22 s +
km12^2 km22 s + k21 km21 km22 s + k22 km21 km22 s + 2 km11 km21 km22 s +
2 km12 km21 km22 s + k11 k12 s^2 + 2 k11 k21 s^2 + 2 k12 k21 s^2 + k21^2 s^2 + 2 k11 k22 s^2 +
2 k12 k22 s^2 + 2 k21 k22 s^2 + k22^2 s^2 + k11 km11 s^2 + 2 k12 km11 s^2 + 2 k21 km11 s^2 +
2 k22 km11 s^2 + km11^2 s^2 + 2 k11 km12 s^2 + k12 km12 s^2 + 2 k21 km12 s^2 + 2 k22 km12 s^2 +
2 km11 km12 s^2 + km12^2 s^2 + k12 km21 s^2 + k21 km21 s^2 + 2 k22 km21 s^2 + 2 km11 km21 s^2 +
2 km12 km21 s^2 + k11 km22 s^2 + 2 k21 km22 s^2 + k22 km22 s^2 + 2 km11 km22 s^2 +
2 km12 km22 s^2 + km21 km22 s^2 + k11 s^3 + k12 s^3 + 2 k21 s^3 + 2 k22 s^3 + 2 km11 s^3 +
2 km12 s^3 + km21 s^3 + km22 s^3 + s^4 + gammam1 (k21 + k22 + km11 + km12 + s)
  (km12 km21 + k21 s + k22 s + km12 s + km21 s + s^2 + k11 (k21 + k22 + s) + km11 (km21 + s)) +
gamma1 (k21 + k22 + km11 + km12 + s) (km12 km22 + k21 s + k22 s +
    km12 s + km22 s + s^2 + k12 (k21 + k22 + s) + km11 (km22 + s)))},
{(km12 (gamma1 k21 km22 + gamma1 k22 km22 + gamma1 km11 km22 + gamma1 km12 km22 +
    k11 km12 km22 + k21 km21 km22 + k22 km21 km22 + km11 km21 km22 + km12 km21 km22 +
    k21 km21 s + k22 km21 s + km11 km21 s + km12 km21 s + gamma1 km22 s + km21 km22 s +
    km21 s^2 + k12 km21 (k21 + k22 + km11 + s) + gammam1 km21 (k21 + k22 + km11 + km12 + s))) /
  (k11 k12 k21^2 + 2 k11 k12 k21 k22 + k11 k12 k22^2 + k11 k12 k21 km11 + k11 k12 k22 km11 +
k11 k12 k21 km12 + k11 k12 k22 km12 + k12 k21 k22 km21 + k12 k22^2 km21 +
k12 k21 km11 km21 + k12 k22 km11 km21 + k12 km11^2 km21 + k12 k21 km12 km21 +
k12 k22 km12 km21 + k12 km11 km12 km21 + k11 k21^2 km22 + k11 k21 k22 km22 +
k11 k21 km11 km22 + k11 k22 km11 km22 + k11 k21 km12 km22 + k11 k22 km12 km22 +
k11 km11 km12 km22 + k11 km12^2 km22 + k21 km11 km21 km22 + k22 km11 km21 km22 +
km11^2 km21 km22 + k21 km12 km21 km22 + k22 km12 km21 km22 + 2 km11 km12 km21 km22 +
km12^2 km21 km22 + 2 k11 k12 k21 s + k11 k21^2 s + k12 k21^2 s + 2 k11 k12 k22 s +
2 k11 k21 k22 s + 2 k12 k21 k22 s + k11 k22^2 s + k12 k22^2 s + k11 k12 km11 s +
k11 k21 km11 s + 2 k12 k21 km11 s + k11 k22 km11 s + 2 k12 k22 km11 s + k12 km11^2 s +
k11 k12 km12 s + 2 k11 k21 km12 s + k12 k21 km12 s + 2 k11 k22 km12 s + k12 k22 km12 s +
k11 km11 km12 s + k12 km11 km12 s + k11 km12^2 s + k12 k21 km21 s + 2 k12 k22 km21 s +
```

```
    k21 k22 km21 s + k22^2 km21 s + 2 k12 km11 km21 s + k21 km11 km21 s + 2 k22 km11 km21 s +
    km11^2 km21 s + k12 km12 km21 s + k21 km12 km21 s + 2 k22 km12 km21 s +
    2 km11 km12 km21 s + km12^2 km21 s + 2 k11 k21 km22 s + k21^2 km22 s + k11 k22 km22 s +
    k21 k22 km22 s + k11 km11 km22 s + 2 k21 km11 km22 s + k22 km11 km22 s + km11^2 km22 s +
    2 k11 km12 km22 s + 2 k21 km12 km22 s + k22 km12 km22 s + 2 km11 km12 km22 s +
    km12^2 km22 s + k21 km21 km22 s + k22 km21 km22 s + 2 km11 km21 km22 s +
    2 km12 km21 km22 s + k11 k12 s^2 + 2 k11 k21 s^2 + 2 k12 k21 s^2 + k21^2 s^2 + 2 k11 k22 s^2 +
    2 k12 k22 s^2 + 2 k21 k22 s^2 + k22^2 s^2 + k11 km11 s^2 + 2 k12 km11 s^2 + 2 k21 km11 s^2 +
    2 k22 km11 s^2 + km11^2 s^2 + 2 k11 km12 s^2 + k12 km12 s^2 + 2 k21 km12 s^2 + 2 k22 km12 s^2 +
    2 km11 km12 s^2 + km12^2 s^2 + k12 km21 s^2 + k21 km21 s^2 + 2 k22 km21 s^2 + 2 km11 km21 s^2 +
    2 km12 km21 s^2 + k11 km22 s^2 + 2 k21 km22 s^2 + k22 km22 s^2 + 2 km11 km22 s^2 +
    2 km12 km22 s^2 + km21 km22 s^2 + k11 s^3 + k12 s^3 + 2 k21 s^3 + 2 k22 s^3 + 2 km11 s^3 +
    2 km12 s^3 + km21 s^3 + km22 s^3 + s^4 + gammam1 (k21 + k22 + km11 + km12 + s)
      (km12 km21 + k21 s + k22 s + km12 s + km21 s + s^2 + k11 (k21 + k22 + s) + km11 (km21 + s)) +
    gamma1 (k21 + k22 + km11 + km12 + s)
      (km12 km22 + k21 s + k22 s + km12 s + km22 s + s^2 + k12 (k21 + k22 + s) + km11 (km22 + s))),
(km12 (k12 km11 km21 + gammam1 km21 (k21 + k22 + km11 + km12 + s) +
     km22 (k11 (k21 + k22 + km12 + s) + gamma1 (k21 + k22 + km11 + km12 + s) +
         (k21 + k22 + km11 + km12 + s) (km21 + s)))) /
 (k11 k12 k21^2 + 2 k11 k12 k21 k22 + k11 k12 k22^2 + k11 k12 k21 km11 + k11 k12 k22 km11 +
    k11 k12 k21 km12 + k11 k12 k22 km12 + k12 k21 k22 km21 + k12 k22^2 km21 +
    k12 k21 km11 km21 + k12 k22 km11 km21 + k12 km11^2 km21 + k12 k21 km12 km21 +
    k12 k22 km12 km21 + k12 km11 km12 km21 + k11 k21^2 km22 + k11 k21 k22 km22 +
    k11 k21 km11 km22 + k11 k22 km11 km22 + k11 k21 km12 km22 + k11 k22 km12 km22 +
    k11 km11 km12 km22 + k11 km12^2 km22 + k21 km11 km21 km22 + k22 km11 km21 km22 +
    km11^2 km21 km22 + k21 km12 km21 km22 + k22 km12 km21 km22 + 2 km11 km12 km21 km22 +
    km12^2 km21 km22 + 2 k11 k12 k21 s + k11 k21^2 s + k12 k21^2 s + 2 k11 k12 k22 s +
    2 k11 k21 k22 s + 2 k12 k21 k22 s + k11 k22^2 s + k12 k22^2 s + k11 k12 km11 s +
    k11 k21 km11 s + 2 k12 k21 km11 s + k11 k22 km11 s + 2 k12 k22 km11 s + k12 km11^2 s +
    k11 k12 km12 s + 2 k11 k21 km12 s + k12 k21 km12 s + 2 k11 k22 km12 s + k12 k22 km12 s +
    k11 km11 km12 s + k12 km11 km12 s + k11 km12^2 s + k12 k21 km21 s + 2 k12 k22 km21 s +
    k21 k22 km21 s + k22^2 km21 s + 2 k12 km11 km21 s + k21 km11 km21 s + 2 k22 km11 km21 s +
    km11^2 km21 s + k12 km12 km21 s + k21 km12 km21 s + 2 k22 km12 km21 s +
    2 km11 km12 km21 s + km12^2 km21 s + 2 k11 k21 km22 s + k21^2 km22 s + k11 k22 km22 s +
    k21 k22 km22 s + k11 km11 km22 s + 2 k21 km11 km22 s + k22 km11 km22 s + km11^2 km22 s +
    2 k11 km12 km22 s + 2 k21 km12 km22 s + k22 km12 km22 s + 2 km11 km12 km22 s +
    km12^2 km22 s + k21 km21 km22 s + k22 km21 km22 s + 2 km11 km21 km22 s +
    2 km12 km21 km22 s + k11 k12 s^2 + 2 k11 k21 s^2 + 2 k12 k21 s^2 + k21^2 s^2 + 2 k11 k22 s^2 +
    2 k12 k22 s^2 + 2 k21 k22 s^2 + k22^2 s^2 + k11 km11 s^2 + 2 k12 km11 s^2 + 2 k21 km11 s^2 +
    2 k22 km11 s^2 + km11^2 s^2 + 2 k11 km12 s^2 + k12 km12 s^2 + 2 k21 km12 s^2 + 2 k22 km12 s^2 +
    2 km11 km12 s^2 + km12^2 s^2 + k12 km21 s^2 + k21 km21 s^2 + 2 k22 km21 s^2 + 2 km11 km21 s^2 +
    2 km12 km21 s^2 + k11 km22 s^2 + 2 k21 km22 s^2 + k22 km22 s^2 + 2 km11 km22 s^2 +
    2 km12 km22 s^2 + km21 km22 s^2 + k11 s^3 + k12 s^3 + 2 k21 s^3 + 2 k22 s^3 + 2 km11 s^3 +
```

```
2 km12 s^3 + km21 s^3 + km22 s^3 + s^4 + gammam1 (k21 + k22 + km11 + km12 + s)
  (km12 km21 + k21 s + k22 s + km12 s + km21 s + s^2 + k11 (k21 + k22 + s) + km11 (km21 + s)) +
gamma1 (k21 + k22 + km11 + km12 + s) (km12 km22 + k21 s + k22 s +
    km12 s + km22 s + s^2 + k12 (k21 + k22 + s) + km11 (km22 + s)))}}
```

```
In[31]:= Omegaminus = Function[s,
  {{(km11 (gamma1 k21 km22 + gamma1 k22 km22 + gamma1 km11 km22 + gamma1 km12 km22 +
        k11 km12 km22 + k21 km21 km22 + k22 km21 km22 + km11 km21 km22 +
        km12 km21 km22 + k21 km21 s + k22 km21 s + km11 km21 s + km12 km21 s +
        gamma1 km22 s + km21 km22 s + km21 s^2 + k12 km21 (k21 + k22 + km11 + s) +
        gammam1 km21 (k21 + k22 + km11 + km12 + s))) /
     (k11 k12 k21^2 + 2 k11 k12 k21 k22 + k11 k12 k22^2 + k11 k12 k21 km11 +
       k11 k12 k22 km11 + k11 k12 k21 km12 + k11 k12 k22 km12 + k12 k21 k22 km21 +
       k12 k22^2 km21 + k12 k21 km11 km21 + k12 k22 km11 km21 + k12 km11^2 km21 +
       k12 k21 km12 km21 + k12 k22 km12 km21 + k12 km11 km12 km21 + k11 k21^2 km22 +
       k11 k21 k22 km22 + k11 k21 km11 km22 + k11 k22 km11 km22 + k11 k21 km12 km22 +
       k11 k22 km12 km22 + k11 km11 km12 km22 + k11 km12^2 km22 + k21 km11 km21 km22 +
       k22 km11 km21 km22 + km11^2 km21 km22 + k21 km12 km21 km22 + k22 km12 km21 km22 +
       2 km11 km12 km21 km22 + km12^2 km21 km22 + 2 k11 k12 k21 s + k11 k21^2 s +
       k12 k21^2 s + 2 k11 k12 k22 s + 2 k11 k21 k22 s + 2 k12 k21 k22 s + k11 k22^2 s +
       k12 k22^2 s + k11 k12 km11 s + k11 k21 km11 s + 2 k12 k21 km11 s + k11 k22 km11 s +
       2 k12 k22 km11 s + k12 km11^2 s + k11 k12 km12 s + 2 k11 k21 km12 s + k12 k21 km12 s +
       2 k11 k22 km12 s + k12 k22 km12 s + k11 km11 km12 s + k12 km11 km12 s + k11 km12^2 s +
       k12 k21 km21 s + 2 k12 k22 km21 s + k21 k22 km21 s + k22^2 km21 s + 2 k12 km11 km21 s +
       k21 km11 km21 s + 2 k22 km11 km21 s + km11^2 km21 s + k12 km12 km21 s +
       k21 km12 km21 s + 2 k22 km12 km21 s + 2 km11 km12 km21 s + km12^2 km21 s +
       2 k11 k21 km22 s + k21^2 km22 s + k11 k22 km22 s + k21 k22 km22 s + k11 km11 km22 s +
       2 k21 km11 km22 s + k22 km11 km22 s + km11^2 km22 s + 2 k11 km12 km22 s +
       2 k21 km12 km22 s + k22 km12 km22 s + 2 km11 km12 km22 s + km12^2 km22 s +
       k21 km21 km22 s + k22 km21 km22 s + 2 km11 km21 km22 s + 2 km12 km21 km22 s +
       k11 k12 s^2 + 2 k11 k21 s^2 + 2 k12 k21 s^2 + k21^2 s^2 + 2 k11 k22 s^2 + 2 k12 k22 s^2 +
       2 k21 k22 s^2 + k22^2 s^2 + k11 km11 s^2 + 2 k12 km11 s^2 + 2 k21 km11 s^2 + 2 k22 km11 s^2 +
       km11^2 s^2 + 2 k11 km12 s^2 + k12 km12 s^2 + 2 k21 km12 s^2 + 2 k22 km12 s^2 + 2 km11 km12 s^2 +
       km12^2 s^2 + k12 km21 s^2 + k21 km21 s^2 + 2 k22 km21 s^2 + 2 km11 km21 s^2 + 2 km12 km21 s^2 +
       k11 km22 s^2 + 2 k21 km22 s^2 + k22 km22 s^2 + 2 km11 km22 s^2 + 2 km12 km22 s^2 +
       km21 km22 s^2 + k11 s^3 + k12 s^3 + 2 k21 s^3 + 2 k22 s^3 + 2 km11 s^3 + 2 km12 s^3 +
       km21 s^3 + km22 s^3 + s^4 + gammam1 (k21 + k22 + km11 + km12 + s) (km12 km21 + k21 s +
          k22 s + km12 s + km21 s + s^2 + k11 (k21 + k22 + s) + km11 (km21 + s)) +
       gamma1 (k21 + k22 + km11 + km12 + s) (km12 km22 + k21 s + k22 s + km12 s +
          km22 s + s^2 + k12 (k21 + k22 + s) + km11 (km22 + s))),
    (km11 (k12 km11 km21 + gammam1 km21 (k21 + k22 + km11 + km12 + s) +
        km22 (k11 (k21 + k22 + km12 + s) + gamma1 (k21 + k22 + km11 + km12 + s) +
           (k21 + k22 + km11 + km12 + s) (km21 + s)))) /
```

```
(k11 k12 k21^2 + 2 k11 k12 k21 k22 + k11 k12 k22^2 + k11 k12 k21 km11 +
  k11 k12 k22 km11 + k11 k12 k21 km12 + k11 k12 k22 km12 + k12 k21 k22 km21 +
  k12 k22^2 km21 + k12 k21 km11 km21 + k12 k22 km11 km21 + k12 km11^2 km21 +
  k12 k21 km12 km21 + k12 k22 km12 km21 + k12 km11 km12 km21 + k11 k21^2 km22 +
  k11 k21 k22 km22 + k11 k21 km11 km22 + k11 k22 km11 km22 + k11 k21 km12 km22 +
  k11 k22 km12 km22 + k11 km11 km12 km22 + k11 km12^2 km22 + k21 km11 km21 km22 +
  k22 km11 km21 km22 + km11^2 km21 km22 + k21 km12 km21 km22 + k22 km12 km21 km22 +
  2 km11 km12 km21 km22 + km12^2 km21 km22 + 2 k11 k12 k21 s + k11 k21^2 s +
  k12 k21^2 s + 2 k11 k12 k22 s + 2 k11 k21 k22 s + 2 k12 k21 k22 s + k11 k22^2 s +
  k12 k22^2 s + k11 k12 km11 s + k11 k21 km11 s + 2 k12 k21 km11 s + k11 k22 km11 s +
  2 k12 k22 km11 s + k12 km11^2 s + k11 k12 km12 s + 2 k11 k21 km12 s + k12 k21 km12 s +
  2 k11 k22 km12 s + k12 k22 km12 s + k11 km11 km12 s + k12 km11 km12 s +
  k11 km12^2 s + k12 k21 km21 s + 2 k12 k22 km21 s + k21 k22 km21 s + k22^2 km21 s +
  2 k12 km11 km21 s + k21 km11 km21 s + 2 k22 km11 km21 s + km11^2 km21 s +
  k12 km12 km21 s + k21 km12 km21 s + 2 k22 km12 km21 s + 2 km11 km12 km21 s +
  km12^2 km21 s + 2 k11 k21 km22 s + k21^2 km22 s + k11 k22 km22 s + k21 k22 km22 s +
  k11 km11 km22 s + 2 k21 km11 km22 s + k22 km11 km22 s + km11^2 km22 s +
  2 k11 km12 km22 s + 2 k21 km12 km22 s + k22 km12 km22 s + 2 km11 km12 km22 s +
  km12^2 km22 s + k21 km21 km22 s + k22 km21 km22 s + 2 km11 km21 km22 s +
  2 km12 km21 km22 s + k11 k12 s^2 + 2 k11 k21 s^2 + 2 k12 k21 s^2 + k21^2 s^2 + 2 k11 k22 s^2 +
  2 k12 k22 s^2 + 2 k21 k22 s^2 + k22^2 s^2 + k11 km11 s^2 + 2 k12 km11 s^2 + 2 k21 km11 s^2 +
  2 k22 km11 s^2 + km11^2 s^2 + 2 k11 km12 s^2 + k12 km12 s^2 + 2 k21 km12 s^2 + 2 k22 km12 s^2 +
  2 km11 km12 s^2 + km12^2 s^2 + k12 km21 s^2 + k21 km21 s^2 + 2 k22 km21 s^2 + 2 km11 km21 s^2 +
  2 km12 km21 s^2 + k11 km22 s^2 + 2 k21 km22 s^2 + k22 km22 s^2 + 2 km11 km22 s^2 +
  2 km12 km22 s^2 + km21 km22 s^2 + k11 s^3 + k12 s^3 + 2 k21 s^3 + 2 k22 s^3 + 2 km11 s^3 +
  2 km12 s^3 + km21 s^3 + km22 s^3 + s^4 + gammam1 (k21 + k22 + km11 + km12 + s) (km12 km21 +
     k21 s + k22 s + km12 s + km21 s + s^2 + k11 (k21 + k22 + s) + km11 (km21 + s)) +
  gamma1 (k21 + k22 + km11 + km12 + s) (km12 km22 + k21 s + k22 s + km12 s +
     km22 s + s^2 + k12 (k21 + k22 + s) + km11 (km22 + s)))},
{(km12 (gamma1 k21 km22 + gamma1 k22 km22 + gamma1 km11 km22 + gamma1 km12 km22 +
    k11 km12 km22 + k21 km21 km22 + k22 km21 km22 + km11 km21 km22 +
    km12 km21 km22 + k21 km21 s + k22 km21 s + km11 km21 s + km12 km21 s +
    gamma1 km22 s + km21 km22 s + km21 s^2 + k12 km21 (k21 + k22 + km11 + s) +
    gammam1 km21 (k21 + k22 + km11 + km12 + s))) /
 (k11 k12 k21^2 + 2 k11 k12 k21 k22 + k11 k12 k22^2 + k11 k12 k21 km11 +
  k11 k12 k22 km11 + k11 k12 k21 km12 + k11 k12 k22 km12 + k12 k21 k22 km21 +
  k12 k22^2 km21 + k12 k21 km11 km21 + k12 k22 km11 km21 + k12 km11^2 km21 +
  k12 k21 km12 km21 + k12 k22 km12 km21 + k12 km11 km12 km21 + k11 k21^2 km22 +
  k11 k21 k22 km22 + k11 k21 km11 km22 + k11 k22 km11 km22 + k11 k21 km12 km22 +
  k11 k22 km12 km22 + k11 km11 km12 km22 + k11 km12^2 km22 + k21 km11 km21 km22 +
  k22 km11 km21 km22 + km11^2 km21 km22 + k21 km12 km21 km22 + k22 km12 km21 km22 +
  2 km11 km12 km21 km22 + km12^2 km21 km22 + 2 k11 k12 k21 s + k11 k21^2 s +
  k12 k21^2 s + 2 k11 k12 k22 s + 2 k11 k21 k22 s + 2 k12 k21 k22 s + k11 k22^2 s +
```

k12 k22$^2$ s + k11 k12 km11 s + k11 k21 km11 s + 2 k12 k21 km11 s + k11 k22 km11 s +
2 k12 k22 km11 s + k12 km11$^2$ s + k11 k12 km12 s + 2 k11 k21 km12 s + k12 k21 km12 s +
2 k11 k22 km12 s + k12 k22 km12 s + k11 km11 km12 s + k12 km11 km12 s +
k11 km12$^2$ s + k12 k21 km21 s + 2 k12 k22 km21 s + k21 k22 km21 s + k22$^2$ km21 s +
2 k12 km11 km21 s + k21 km11 km21 s + 2 k22 km11 km21 s + km11$^2$ km21 s +
k12 km12 km21 s + k21 km12 km21 s + 2 k22 km12 km21 s + 2 km11 km12 km21 s +
km12$^2$ km21 s + 2 k11 k21 km22 s + k21$^2$ km22 s + k11 k22 km22 s + k21 k22 km22 s +
k11 km11 km22 s + 2 k21 km11 km22 s + k22 km11 km22 s + km11$^2$ km22 s +
2 k11 km12 km22 s + 2 k21 km12 km22 s + k22 km12 km22 s + 2 km11 km12 km22 s +
km12$^2$ km22 s + k21 km21 km22 s + k22 km21 km22 s + 2 km11 km21 km22 s +
2 km12 km21 km22 s + k11 k12 s$^2$ + 2 k11 k21 s$^2$ + 2 k12 k21 s$^2$ + k21$^2$ s$^2$ + 2 k11 k22 s$^2$ +
2 k12 k22 s$^2$ + 2 k21 k22 s$^2$ + k22$^2$ s$^2$ + k11 km11 s$^2$ + 2 k12 km11 s$^2$ + 2 k21 km11 s$^2$ +
2 k22 km11 s$^2$ + km11$^2$ s$^2$ + 2 k11 km12 s$^2$ + k12 km12 s$^2$ + 2 k21 km12 s$^2$ + 2 k22 km12 s$^2$ +
2 km11 km12 s$^2$ + km12$^2$ s$^2$ + k12 km21 s$^2$ + k21 km21 s$^2$ + 2 k22 km21 s$^2$ + 2 km11 km21 s$^2$ +
2 km12 km21 s$^2$ + k11 km22 s$^2$ + 2 k21 km22 s$^2$ + k22 km22 s$^2$ + 2 km11 km22 s$^2$ +
2 km12 km22 s$^2$ + km21 km22 s$^2$ + k11 s$^3$ + k12 s$^3$ + 2 k21 s$^3$ + 2 k22 s$^3$ + 2 km11 s$^3$ +
2 km12 s$^3$ + km21 s$^3$ + km22 s$^3$ + s$^4$ + gammam1 (k21 + k22 + km11 + km12 + s) (km12 km21 +
k21 s + k22 s + km12 s + km21 s + s$^2$ + k11 (k21 + k22 + s) + km11 (km21 + s)) +
gamma1 (k21 + k22 + km11 + km12 + s) (km12 km22 + k21 s + k22 s + km12 s +
km22 s + s$^2$ + k12 (k21 + k22 + s) + km11 (km22 + s))),
(km12 (k12 km11 km21 + gammam1 km21 (k21 + k22 + km11 + km12 + s) +
km22 (k11 (k21 + k22 + km12 + s) + gamma1 (k21 + k22 + km11 + km12 + s) +
(k21 + k22 + km11 + km12 + s) (km21 + s)))) /
(k11 k12 k21$^2$ + 2 k11 k12 k21 k22 + k11 k12 k22$^2$ + k11 k12 k21 km11 +
k11 k12 k22 km11 + k11 k12 k21 km12 + k11 k12 k22 km12 + k12 k21 k22 km21 +
k12 k22$^2$ km21 + k12 k21 km11 km21 + k12 k22 km11 km21 + k12 km11$^2$ km21 +
k12 k21 km12 km21 + k12 k22 km12 km21 + k12 km11 km12 km21 + k11 k21$^2$ km22 +
k11 k21 k22 km22 + k11 k21 km11 km22 + k11 k22 km11 km22 + k11 k21 km12 km22 +
k11 k22 km12 km22 + k11 km11 km12 km22 + k11 km12$^2$ km22 + k21 km11 km21 km22 +
k22 km11 km21 km22 + km11$^2$ km21 km22 + k21 km12 km21 km22 + k22 km12 km21 km22 +
2 km11 km12 km21 km22 + km12$^2$ km21 km22 + 2 k11 k12 k21 s + k11 k21$^2$ s +
k12 k21$^2$ s + 2 k11 k12 k22 s + 2 k11 k21 k22 s + 2 k12 k21 k22 s + k11 k22$^2$ s +
k12 k22$^2$ s + k11 k12 km11 s + k11 k21 km11 s + 2 k12 k21 km11 s + k11 k22 km11 s +
2 k12 k22 km11 s + k12 km11$^2$ s + k11 k12 km12 s + 2 k11 k21 km12 s + k12 k21 km12 s +
2 k11 k22 km12 s + k12 k22 km12 s + k11 km11 km12 s + k12 km11 km12 s +
k11 km12$^2$ s + k12 k21 km21 s + 2 k12 k22 km21 s + k21 k22 km21 s + k22$^2$ km21 s +
2 k12 km11 km21 s + k21 km11 km21 s + 2 k22 km11 km21 s + km11$^2$ km21 s +
k12 km12 km21 s + k21 km12 km21 s + 2 k22 km12 km21 s + 2 km11 km12 km21 s +
km12$^2$ km21 s + 2 k11 k21 km22 s + k21$^2$ km22 s + k11 k22 km22 s + k21 k22 km22 s +
k11 km11 km22 s + 2 k21 km11 km22 s + k22 km11 km22 s + km11$^2$ km22 s +
2 k11 km12 km22 s + 2 k21 km12 km22 s + k22 km12 km22 s + 2 km11 km12 km22 s +
km12$^2$ km22 s + k21 km21 km22 s + k22 km21 km22 s + 2 km11 km21 km22 s +
2 km12 km21 km22 s + k11 k12 s$^2$ + 2 k11 k21 s$^2$ + 2 k12 k21 s$^2$ + k21$^2$ s$^2$ + 2 k11 k22 s$^2$ +

```
2 k12 k22 s^2 + 2 k21 k22 s^2 + k22^2 s^2 + k11 km11 s^2 + 2 k12 km11 s^2 + 2 k21 km11 s^2 +
2 k22 km11 s^2 + km11^2 s^2 + 2 k11 km12 s^2 + k12 km12 s^2 + 2 k21 km12 s^2 + 2 k22 km12 s^2 +
2 km11 km12 s^2 + km12^2 s^2 + k12 km21 s^2 + k21 km21 s^2 + 2 k22 km21 s^2 + 2 km11 km21 s^2 +
2 km12 km21 s^2 + k11 km22 s^2 + 2 k21 km22 s^2 + k22 km22 s^2 + 2 km11 km22 s^2 +
2 km12 km22 s^2 + km21 km22 s^2 + k11 s^3 + k12 s^3 + 2 k21 s^3 + 2 k22 s^3 + 2 km11 s^3 +
2 km12 s^3 + km21 s^3 + km22 s^3 + s^4 + gammam1 (k21 + k22 + km11 + km12 + s) (km12 km21 +
   k21 s + k22 s + km12 s + km21 s + s^2 + k11 (k21 + k22 + s) + km11 (km21 + s)) +
gamma1 (k21 + k22 + km11 + km12 + s) (km12 km22 + k21 s + k22 s + km12 s +
   km22 s + s^2 + k12 (k21 + k22 + s) + km11 (km22 + s)))}}]
```

Out[31]=

```
Function[s,
 {{(km11 (gamma1 k21 km22 + gamma1 k22 km22 + gamma1 km11 km22 + gamma1 km12 km22 + k11 km12
        km22 + k21 km21 km22 + k22 km21 km22 + km11 km21 km22 + km12 km21 km22 + k21 km21 s +
      k22 km21 s + km11 km21 s + km12 km21 s + gamma1 km22 s + km21 km22 s + km21 s^2 +
      k12 km21 (k21 + k22 + km11 + s) + gammam1 km21 (k21 + k22 + km11 + km12 + s))) /
   (k11 k12 k21^2 + 2 k11 k12 k21 k22 + k11 k12 k22^2 + k11 k12 k21 km11 + k11 k12 k22 km11 +
    k11 k12 k21 km12 + k11 k12 k22 km12 + k12 k21 k22 km21 + k12 k22^2 km21 +
    k12 k21 km11 km21 + k12 k22 km11 km21 + k12 km11^2 km21 + k12 k21 km12 km21 +
    k12 k22 km12 km21 + k12 km11 km12 km21 + k11 k21^2 km22 + k11 k21 k22 km22 +
    k11 k21 km11 km22 + k11 k22 km11 km22 + k11 k21 km12 km22 + k11 k22 km12 km22 +
    k11 km11 km12 km22 + k11 km12^2 km22 + k21 km11 km21 km22 + k22 km11 km21 km22 +
    km11^2 km21 km22 + k21 km12 km21 km22 + k22 km12 km21 km22 + 2 km11 km12 km21 km22 +
    km12^2 km21 km22 + 2 k11 k12 k21 s + k11 k21^2 s + k12 k21^2 s + 2 k11 k12 k22 s +
    2 k11 k21 k22 s + 2 k12 k21 k22 s + k11 k22^2 s + k12 k22^2 s + k11 k12 km11 s +
    k11 k21 km11 s + 2 k12 k21 km11 s + k11 k22 km11 s + 2 k12 k22 km11 s + k12 km11^2 s +
    k11 k12 km12 s + 2 k11 k21 km12 s + k12 k21 km12 s + 2 k11 k22 km12 s + k12 k22 km12 s +
    k11 km11 km12 s + k12 km11 km12 s + k11 km12^2 s + k12 k21 km21 s + 2 k12 k22 km21 s +
    k21 k22 km21 s + k22^2 km21 s + 2 k12 km11 km21 s + k21 km11 km21 s + 2 k22 km11 km21 s +
    km11^2 km21 s + k12 km12 km21 s + k21 km12 km21 s + 2 k22 km12 km21 s +
    2 km11 km12 km21 s + km12^2 km21 s + 2 k11 k21 km22 s + k21^2 km22 s + k11 k22 km22 s +
    k21 k22 km22 s + k11 km11 km22 s + 2 k21 km11 km22 s + k22 km11 km22 s + km11^2 km22 s +
    2 k11 km12 km22 s + 2 k21 km12 km22 s + k22 km12 km22 s + 2 km11 km12 km22 s +
    km12^2 km22 s + k21 km21 km22 s + k22 km21 km22 s + 2 km11 km21 km22 s +
    2 km12 km21 km22 s + k11 k12 s^2 + 2 k11 k21 s^2 + 2 k12 k21 s^2 + k21^2 s^2 + 2 k11 k22 s^2 +
    2 k12 k22 s^2 + 2 k21 k22 s^2 + k22^2 s^2 + k11 km11 s^2 + 2 k12 km11 s^2 + 2 k21 km11 s^2 +
    2 k22 km11 s^2 + km11^2 s^2 + 2 k11 km12 s^2 + k12 km12 s^2 + 2 k21 km12 s^2 + 2 k22 km12 s^2 +
    2 km11 km12 s^2 + km12^2 s^2 + k12 km21 s^2 + k21 km21 s^2 + 2 k22 km21 s^2 + 2 km11 km21 s^2 +
    2 km12 km21 s^2 + k11 km22 s^2 + 2 k21 km22 s^2 + k22 km22 s^2 + 2 km11 km22 s^2 +
    2 km12 km22 s^2 + km21 km22 s^2 + k11 s^3 + k12 s^3 + 2 k21 s^3 + 2 k22 s^3 + 2 km11 s^3 +
    2 km12 s^3 + km21 s^3 + km22 s^3 + s^4 + gammam1 (k21 + k22 + km11 + km12 + s)
      (km12 km21 + k21 s + k22 s + km12 s + km21 s + s^2 + k11 (k21 + k22 + s) + km11 (km21 + s)) +
    gamma1 (k21 + k22 + km11 + km12 + s) (km12 km22 + k21 s + k22 s +
        km12 s + km22 s + s^2 + k12 (k21 + k22 + s) + km11 (km22 + s))),
```

```
(km11 (k12 km11 km21 + gammam1 km21 (k21 + k22 + km11 + km12 + s) +
      km22 (k11 (k21 + k22 + km12 + s) + gamma1 (k21 + k22 + km11 + km12 + s) +
            (k21 + k22 + km11 + km12 + s) (km21 + s)))) /
 (k11 k12 k21^2 + 2 k11 k12 k21 k22 + k11 k12 k22^2 + k11 k12 k21 km11 + k11 k12 k22 km11 +
   k11 k12 k21 km12 + k11 k12 k22 km12 + k12 k21 k22 km21 + k12 k22^2 km21 +
   k12 k21 km11 km21 + k12 k22 km11 km21 + k12 km11^2 km21 + k12 k21 km12 km21 +
   k12 k22 km12 km21 + k12 km11 km12 km21 + k11 k21^2 km22 + k11 k21 k22 km22 +
   k11 k21 km11 km22 + k11 k22 km11 km22 + k11 k21 km12 km22 + k11 k22 km12 km22 +
   k11 km11 km12 km22 + k11 km12^2 km22 + k21 km11 km21 km22 + k22 km11 km21 km22 +
   km11^2 km21 km22 + k21 km12 km21 km22 + k22 km12 km21 km22 + 2 km11 km12 km21 km22 +
   km12^2 km21 km22 + 2 k11 k12 k21 s + k11 k21^2 s + k12 k21^2 s + 2 k11 k12 k22 s +
   2 k11 k21 k22 s + 2 k12 k21 k22 s + k11 k22^2 s + k12 k22^2 s + k11 k12 km11 s +
   k11 k21 km11 s + 2 k12 k21 km11 s + k11 k22 km11 s + 2 k12 k22 km11 s + k12 km11^2 s +
   k11 k12 km12 s + 2 k11 k21 km12 s + k12 k21 km12 s + 2 k11 k22 km12 s + k12 k22 km12 s +
   k11 km11 km12 s + k12 km11 km12 s + k11 km12^2 s + k12 k21 km21 s + 2 k12 k22 km21 s +
   k21 k22 km21 s + k22^2 km21 s + 2 k12 km11 km21 s + k21 km11 km21 s + 2 k22 km11 km21 s +
   km11^2 km21 s + k12 km12 km21 s + k21 km12 km21 s + 2 k22 km12 km21 s +
   2 km11 km12 km21 s + km12^2 km21 s + 2 k11 k21 km22 s + k21^2 km22 s + k11 k22 km22 s +
   k21 k22 km22 s + k11 km11 km22 s + 2 k21 km11 km22 s + k22 km11 km22 s + km11^2 km22 s +
   2 k11 km12 km22 s + 2 k21 km12 km22 s + k22 km12 km22 s + 2 km11 km12 km22 s +
   km12^2 km22 s + k21 km21 km22 s + k22 km21 km22 s + 2 km11 km21 km22 s +
   2 km12 km21 km22 s + k11 k12 s^2 + 2 k11 k21 s^2 + 2 k12 k21 s^2 + k21^2 s^2 + 2 k11 k22 s^2 +
   2 k12 k22 s^2 + 2 k21 k22 s^2 + k22^2 s^2 + k11 km11 s^2 + 2 k12 km11 s^2 + 2 k21 km11 s^2 +
   2 k22 km11 s^2 + km11^2 s^2 + 2 k11 km12 s^2 + k12 km12 s^2 + 2 k21 km12 s^2 + 2 k22 km12 s^2 +
   2 km11 km12 s^2 + km12^2 s^2 + k12 km21 s^2 + k21 km21 s^2 + 2 k22 km21 s^2 + 2 km11 km21 s^2 +
   2 km12 km21 s^2 + k11 km22 s^2 + 2 k21 km22 s^2 + k22 km22 s^2 + 2 km11 km22 s^2 +
   2 km12 km22 s^2 + km21 km22 s^2 + k11 s^3 + k12 s^3 + 2 k21 s^3 + 2 k22 s^3 + 2 km11 s^3 +
   2 km12 s^3 + km21 s^3 + km22 s^3 + s^4 + gammam1 (k21 + k22 + km11 + km12 + s)
    (km12 km21 + k21 s + k22 s + km12 s + km21 s + s^2 + k11 (k21 + k22 + s) + km11 (km21 + s)) +
   gamma1 (k21 + k22 + km11 + km12 + s) (km12 km22 + k21 s + k22 s +
      km12 s + km22 s + s^2 + k12 (k21 + k22 + s) + km11 (km22 + s)))},
{(km12 (gamma1 k21 km22 + gamma1 k22 km22 + gamma1 km11 km22 + gamma1 km12 km22 + k11 km12
        km22 + k21 km21 km22 + k22 km21 km22 + km11 km21 km22 + km12 km21 km22 + k21 km21 s +
      k22 km21 s + km11 km21 s + km12 km21 s + gamma1 km22 s + km21 km22 s + km21 s^2 +
      k12 km21 (k21 + k22 + km11 + s) + gammam1 km21 (k21 + k22 + km11 + km12 + s))) /
 (k11 k12 k21^2 + 2 k11 k12 k21 k22 + k11 k12 k22^2 + k11 k12 k21 km11 + k11 k12 k22 km11 +
   k11 k12 k21 km12 + k11 k12 k22 km12 + k12 k21 k22 km21 + k12 k22^2 km21 +
   k12 k21 km11 km21 + k12 k22 km11 km21 + k12 km11^2 km21 + k12 k21 km12 km21 +
   k12 k22 km12 km21 + k12 km11 km12 km21 + k11 k21^2 km22 + k11 k21 k22 km22 +
   k11 k21 km11 km22 + k11 k22 km11 km22 + k11 k21 km12 km22 + k11 k22 km12 km22 +
   k11 km11 km12 km22 + k11 km12^2 km22 + k21 km11 km21 km22 + k22 km11 km21 km22 +
   km11^2 km21 km22 + k21 km12 km21 km22 + k22 km12 km21 km22 + 2 km11 km12 km21 km22 +
   km12^2 km21 km22 + 2 k11 k12 k21 s + k11 k21^2 s + k12 k21^2 s + 2 k11 k12 k22 s +
```

$2\ k11\ k21\ k22\ s + 2\ k12\ k21\ k22\ s + k11\ k22^2\ s + k12\ k22^2\ s + k11\ k12\ km11\ s +$
$k11\ k21\ km11\ s + 2\ k12\ k21\ km11\ s + k11\ k22\ km11\ s + 2\ k12\ k22\ km11\ s + k12\ km11^2\ s +$
$k11\ k12\ km12\ s + 2\ k11\ k21\ km12\ s + k12\ k21\ km12\ s + 2\ k11\ k22\ km12\ s + k12\ k22\ km12\ s +$
$k11\ km11\ km12\ s + k12\ km11\ km12\ s + k11\ km12^2\ s + k12\ k21\ km21\ s + 2\ k12\ k22\ km21\ s +$
$k21\ k22\ km21\ s + k22^2\ km21\ s + 2\ k12\ km11\ km21\ s + k21\ km11\ km21\ s + 2\ k22\ km11\ km21\ s +$
$km11^2\ km21\ s + k12\ km12\ km21\ s + k21\ km12\ km21\ s + 2\ k22\ km12\ km21\ s +$
$2\ km11\ km12\ km21\ s + km12^2\ km21\ s + 2\ k11\ k21\ km22\ s + k21^2\ km22\ s + k11\ k22\ km22\ s +$
$k21\ k22\ km22\ s + k11\ km11\ km22\ s + 2\ k21\ km11\ km22\ s + k22\ km11\ km22\ s + km11^2\ km22\ s +$
$2\ k11\ km12\ km22\ s + 2\ k21\ km12\ km22\ s + k22\ km12\ km22\ s + 2\ km11\ km12\ km22\ s +$
$km12^2\ km22\ s + k21\ km21\ km22\ s + k22\ km21\ km22\ s + 2\ km11\ km21\ km22\ s +$
$2\ km12\ km21\ km22\ s + k11\ k12\ s^2 + 2\ k11\ k21\ s^2 + 2\ k12\ k21\ s^2 + k21^2\ s^2 + 2\ k11\ k22\ s^2 +$
$2\ k12\ k22\ s^2 + 2\ k21\ k22\ s^2 + k22^2\ s^2 + k11\ km11\ s^2 + 2\ k12\ km11\ s^2 + 2\ k21\ km11\ s^2 +$
$2\ k22\ km11\ s^2 + km11^2\ s^2 + 2\ k11\ km12\ s^2 + k12\ km12\ s^2 + 2\ k21\ km12\ s^2 + 2\ k22\ km12\ s^2 +$
$2\ km11\ km12\ s^2 + km12^2\ s^2 + k12\ km21\ s^2 + k21\ km21\ s^2 + 2\ k22\ km21\ s^2 + 2\ km11\ km21\ s^2 +$
$2\ km12\ km21\ s^2 + k11\ km22\ s^2 + 2\ k21\ km22\ s^2 + k22\ km22\ s^2 + 2\ km11\ km22\ s^2 +$
$2\ km12\ km22\ s^2 + km21\ km22\ s^2 + k11\ s^3 + k12\ s^3 + 2\ k21\ s^3 + 2\ k22\ s^3 + 2\ km11\ s^3 +$
$2\ km12\ s^3 + km21\ s^3 + km22\ s^3 + s^4 + gammam1\ (k21 + k22 + km11 + km12 + s)$
$\left(km12\ km21 + k21\ s + k22\ s + km12\ s + km21\ s + s^2 + k11\ (k21 + k22 + s) + km11\ (km21 + s)\right) +$
$gamma1\ (k21 + k22 + km11 + km12 + s)\ \left(km12\ km22 + k21\ s + k22\ s +\right.$
$\left.km12\ s + km22\ s + s^2 + k12\ (k21 + k22 + s) + km11\ (km22 + s)\right)\Big),$
$(km12\ (k12\ km11\ km21 + gammam1\ km21\ (k21 + k22 + km11 + km12 + s) +$
$km22\ (k11\ (k21 + k22 + km12 + s) + gamma1\ (k21 + k22 + km11 + km12 + s) +$
$(k21 + k22 + km11 + km12 + s)\ (km21 + s)))) \big/$
$\Big(k11\ k12\ k21^2 + 2\ k11\ k12\ k21\ k22 + k11\ k12\ k22^2 + k11\ k12\ k21\ km11 +$
$k11\ k12\ k22\ km11 + k11\ k12\ k21\ km12 + k11\ k12\ k22\ km12 + k12\ k21\ k22\ km21 +$
$k12\ k22^2\ km21 + k12\ k21\ km11\ km21 + k12\ k22\ km11\ km21 + k12\ km11^2\ km21 +$
$k12\ k21\ km12\ km21 + k12\ k22\ km12\ km21 + k12\ km11\ km12\ km21 + k11\ k21^2\ km22 +$
$k11\ k21\ k22\ km22 + k11\ k21\ km11\ km22 + k11\ k22\ km11\ km22 + k11\ k21\ km12\ km22 +$
$k11\ k22\ km12\ km22 + k11\ km11\ km12\ km22 + k11\ km12^2\ km22 + k21\ km11\ km21\ km22 +$
$k22\ km11\ km21\ km22 + km11^2\ km21\ km22 + k21\ km12\ km21\ km22 + k22\ km12\ km21\ km22 +$
$2\ km11\ km12\ km21\ km22 + km12^2\ km21\ km22 + 2\ k11\ k12\ k21\ s + k11\ k21^2\ s +$
$k12\ k21^2\ s + 2\ k11\ k12\ k22\ s + 2\ k11\ k21\ k22\ s + 2\ k12\ k21\ k22\ s + k11\ k22^2\ s +$
$k12\ k22^2\ s + k11\ k12\ km11\ s + k11\ k21\ km11\ s + 2\ k12\ k21\ km11\ s + k11\ k22\ km11\ s +$
$2\ k12\ k22\ km11\ s + k12\ km11^2\ s + k11\ k12\ km12\ s + 2\ k11\ k21\ km12\ s + k12\ k21\ km12\ s +$
$2\ k11\ k22\ km12\ s + k12\ k22\ km12\ s + k11\ km11\ km12\ s + k12\ km11\ km12\ s +$
$k11\ km12^2\ s + k12\ k21\ km21\ s + 2\ k12\ k22\ km21\ s + k21\ k22\ km21\ s + k22^2\ km21\ s +$
$2\ k12\ km11\ km21\ s + k21\ km11\ km21\ s + 2\ k22\ km11\ km21\ s + km11^2\ km21\ s +$
$k12\ km12\ km21\ s + k21\ km12\ km21\ s + 2\ k22\ km12\ km21\ s + 2\ km11\ km12\ km21\ s +$
$km12^2\ km21\ s + 2\ k11\ k21\ km22\ s + k21^2\ km22\ s + k11\ k22\ km22\ s + k21\ k22\ km22\ s +$
$k11\ km11\ km22\ s + 2\ k21\ km11\ km22\ s + k22\ km11\ km22\ s + km11^2\ km22\ s +$
$2\ k11\ km12\ km22\ s + 2\ k21\ km12\ km22\ s + k22\ km12\ km22\ s + 2\ km11\ km12\ km22\ s +$
$km12^2\ km22\ s + k21\ km21\ km22\ s + k22\ km21\ km22\ s + 2\ km11\ km21\ km22\ s +$
$2\ km12\ km21\ km22\ s + k11\ k12\ s^2 + 2\ k11\ k21\ s^2 + 2\ k12\ k21\ s^2 + k21^2\ s^2 + 2\ k11\ k22\ s^2 +$

```
2 k12 k22 s^2 + 2 k21 k22 s^2 + k22^2 s^2 + k11 km11 s^2 + 2 k12 km11 s^2 + 2 k21 km11 s^2 +
2 k22 km11 s^2 + km11^2 s^2 + 2 k11 km12 s^2 + k12 km12 s^2 + 2 k21 km12 s^2 + 2 k22 km12 s^2 +
2 km11 km12 s^2 + km12^2 s^2 + k12 km21 s^2 + k21 km21 s^2 + 2 k22 km21 s^2 + 2 km11 km21 s^2 +
2 km12 km21 s^2 + k11 km22 s^2 + 2 k21 km22 s^2 + k22 km22 s^2 + 2 km11 km22 s^2 +
2 km12 km22 s^2 + km21 km22 s^2 + k11 s^3 + k12 s^3 + 2 k21 s^3 + 2 k22 s^3 + 2 km11 s^3 +
2 km12 s^3 + km21 s^3 + km22 s^3 + s^4 + gammam1 (k21 + k22 + km11 + km12 + s)
  (km12 km21 + k21 s + k22 s + km12 s + km21 s + s^2 + k11 (k21 + k22 + s) + km11 (km21 + s)) +
gamma1 (k21 + k22 + km11 + km12 + s) (km12 km22 + k21 s + k22 s +
    km12 s + km22 s + s^2 + k12 (k21 + k22 + s) + km11 (km22 + s)))}}]
```

```
In[32]:= Omega = Function[s, Omegaplus[s] + Omegaminus[s]]
Out[32]=
Function[s, Omegaplus[s] + Omegaminus[s]]
```

```
In[33]:= Pbarev0 = {{Pbarev01}, {1 - Pbarev01}}
Out[33]=
{{Pbarev01}, {1 - Pbarev01}}
```

```
In[34]:= Factor[Simplify[Together[Solve[Omega[0].Pbarev0 == Pbarev0, Pbarev01]]]]
Out[34]=
{{Pbarev01 →
   (gammam1 k11 k21^2 + gamma1 k12 k21^2 + k11 k12 k21^2 + gammam1 k11 k21 k22 + gamma1 k12 k21
      k22 + k11 k12 k21 k22 + gammam1 k11 k21 km11 + gamma1 k12 k21 km11 + k11 k12 k21 km11 +
    gammam1 k11 k21 km12 + gamma1 k12 k21 km12 + k11 k12 k21 km12 + k12 k21 k22 km21 +
    gammam1 k21 km11 km21 + k12 k21 km11 km21 + gammam1 k22 km11 km21 +
    gammam1 km11^2 km21 + k12 km11^2 km21 + k12 k21 km12 km21 + gammam1 km11 km12 km21 +
    k11 k21^2 km22 + gamma1 k21 km11 km22 + k11 k21 km11 km22 + gamma1 k22 km11 km22 +
    k11 k22 km11 km22 + gamma1 km11^2 km22 + gamma1 km11 km12 km22 + k11 km11 km12 km22 +
    k21 km11 km21 km22 + k22 km11 km21 km22 + km11^2 km21 km22 + km11 km12 km21 km22) /
  (gammam1 k11 k21^2 + gamma1 k12 k21^2 + k11 k12 k21^2 + 2 gammam1 k11 k21 k22 +
    2 gamma1 k12 k21 k22 + 2 k11 k12 k21 k22 + gammam1 k11 k22^2 + gamma1 k12 k22^2 +
    k11 k12 k22^2 + gammam1 k11 k21 km11 + gamma1 k12 k21 km11 + k11 k12 k21 km11 +
    gammam1 k11 k22 km11 + gamma1 k12 k22 km11 + k11 k12 k22 km11 + gammam1 k11 k21 km12 +
    gamma1 k12 k21 km12 + k11 k12 k21 km12 + gammam1 k11 k22 km12 + gamma1 k12 k22 km12 +
    k11 k12 k22 km12 + k12 k21 k22 km21 + k12 k22^2 km21 + gammam1 k21 km11 km21 +
    k12 k21 km11 km21 + gammam1 k22 km11 km21 + gammam1 km11^2 km21 + k12 km11^2 km21 +
    gammam1 k21 km12 km21 + 2 k12 k21 km12 km21 + gammam1 k22 km12 km21 +
    k12 k22 km12 km21 + 2 gammam1 km11 km12 km21 + k12 km11 km12 km21 +
    gammam1 km12^2 km21 + k11 k21^2 km22 + k11 k21 k22 km22 + gamma1 k21 km11 km22 +
    k11 k21 km11 km22 + gamma1 k22 km11 km22 + 2 k11 k22 km11 km22 + gamma1 km11^2 km22 +
    gamma1 k21 km12 km22 + gamma1 k22 km12 km22 + k11 k22 km12 km22 +
    2 gamma1 km11 km12 km22 + k11 km11 km12 km22 + gamma1 km12^2 km22 +
    k11 km12^2 km22 + k21 km11 km21 km22 + k22 km11 km21 km22 + km11^2 km21 km22 +
    k21 km12 km21 km22 + k22 km12 km21 km22 + 2 km11 km12 km21 km22 + km12^2 km21 km22)}}
```

```
In[35]:= Pbarev01 = (gammam1 k11 k21^2 + gamma1 k12 k21^2 + k11 k12 k21^2 + gammam1 k11 k21 k22 +
      gamma1 k12 k21 k22 + k11 k12 k21 k22 + gammam1 k11 k21 km11 + gamma1 k12 k21 km11 +
      k11 k12 k21 km11 + gammam1 k11 k21 km12 + gamma1 k12 k21 km12 + k11 k12 k21 km12 +
      k12 k21 k22 km21 + gammam1 k21 km11 km21 + k12 k21 km11 km21 + gammam1 k22 km11 km21 +
      gammam1 km11^2 km21 + k12 km11^2 km21 + k12 k21 km12 km21 + gammam1 km11 km12 km21 +
      k11 k21^2 km22 + gamma1 k21 km11 km22 + k11 k21 km11 km22 + gamma1 k22 km11 km22 +
      k11 k22 km11 km22 + gamma1 km11^2 km22 + gamma1 km11 km12 km22 + k11 km11 km12 km22 +
      k21 km11 km21 km22 + k22 km11 km21 km22 + km11^2 km21 km22 + km11 km12 km21 km22) /
    (gammam1 k11 k21^2 + gamma1 k12 k21^2 + k11 k12 k21^2 + 2 gammam1 k11 k21 k22 +
      2 gamma1 k12 k21 k22 + 2 k11 k12 k21 k22 + gammam1 k11 k22^2 + gamma1 k12 k22^2 +
      k11 k12 k22^2 + gammam1 k11 k21 km11 + gamma1 k12 k21 km11 + k11 k12 k21 km11 +
      gammam1 k11 k22 km11 + gamma1 k12 k22 km11 + k11 k12 k22 km11 + gammam1 k11 k21 km12 +
      gamma1 k12 k21 km12 + k11 k12 k21 km12 + gammam1 k11 k22 km12 + gamma1 k12 k22 km12 +
      k11 k12 k22 km12 + k12 k21 k22 km21 + k12 k22^2 km21 + gammam1 k21 km11 km21 +
      k12 k21 km11 km21 + gammam1 k22 km11 km21 + gammam1 km11^2 km21 + k12 km11^2 km21 +
      gammam1 k21 km12 km21 + 2 k12 k21 km12 km21 + gammam1 k22 km12 km21 + k12 k22 km12 km21 +
      2 gammam1 km11 km12 km21 + k12 km11 km12 km21 + gammam1 km12^2 km21 + k11 k21^2 km22 +
      k11 k21 k22 km22 + gamma1 k21 km11 km22 + k11 k21 km11 km22 + gamma1 k22 km11 km22 +
      2 k11 k22 km11 km22 + gamma1 km11^2 km22 + gamma1 k21 km12 km22 + gamma1 k22 km12 km22 +
      k11 k22 km12 km22 + 2 gamma1 km11 km12 km22 + k11 km11 km12 km22 + gamma1 km12^2 km22 +
      k11 km12^2 km22 + k21 km11 km21 km22 + k22 km11 km21 km22 + km11^2 km21 km22 +
      k21 km12 km21 km22 + k22 km12 km21 km22 + 2 km11 km12 km21 km22 + km12^2 km21 km22)
```

Out[35]=

```
(gammam1 k11 k21^2 + gamma1 k12 k21^2 + k11 k12 k21^2 + gammam1 k11 k21 k22 +
    gamma1 k12 k21 k22 + k11 k12 k21 k22 + gammam1 k11 k21 km11 + gamma1 k12 k21 km11 +
    k11 k12 k21 km11 + gammam1 k11 k21 km12 + gamma1 k12 k21 km12 + k11 k12 k21 km12 +
    k12 k21 k22 km21 + gammam1 k21 km11 km21 + k12 k21 km11 km21 + gammam1 k22 km11 km21 +
    gammam1 km11^2 km21 + k12 km11^2 km21 + k12 k21 km12 km21 + gammam1 km11 km12 km21 +
    k11 k21^2 km22 + gamma1 k21 km11 km22 + k11 k21 km11 km22 + gamma1 k22 km11 km22 +
    k11 k22 km11 km22 + gamma1 km11^2 km22 + gamma1 km11 km12 km22 + k11 km11 km12 km22 +
    k21 km11 km21 km22 + k22 km11 km21 km22 + km11^2 km21 km22 + km11 km12 km21 km22) /
  (gammam1 k11 k21^2 + gamma1 k12 k21^2 + k11 k12 k21^2 + 2 gammam1 k11 k21 k22 +
    2 gamma1 k12 k21 k22 + 2 k11 k12 k21 k22 + gammam1 k11 k22^2 + gamma1 k12 k22^2 +
    k11 k12 k22^2 + gammam1 k11 k21 km11 + gamma1 k12 k21 km11 + k11 k12 k21 km11 +
    gammam1 k11 k22 km11 + gamma1 k12 k22 km11 + k11 k12 k22 km11 + gammam1 k11 k21 km12 +
    gamma1 k12 k21 km12 + k11 k12 k21 km12 + gammam1 k11 k22 km12 + gamma1 k12 k22 km12 +
    k11 k12 k22 km12 + k12 k21 k22 km21 + k12 k22^2 km21 + gammam1 k21 km11 km21 +
    k12 k21 km11 km21 + gammam1 k22 km11 km21 + gammam1 km11^2 km21 + k12 km11^2 km21 +
    gammam1 k21 km12 km21 + 2 k12 k21 km12 km21 + gammam1 k22 km12 km21 + k12 k22 km12 km21 +
    2 gammam1 km11 km12 km21 + k12 km11 km12 km21 + gammam1 km12^2 km21 + k11 k21^2 km22 +
    k11 k21 k22 km22 + gamma1 k21 km11 km22 + k11 k21 km11 km22 + gamma1 k22 km11 km22 +
    2 k11 k22 km11 km22 + gamma1 km11^2 km22 + gamma1 k21 km12 km22 + gamma1 k22 km12 km22 +
    k11 k22 km12 km22 + 2 gamma1 km11 km12 km22 + k11 km11 km12 km22 + gamma1 km12^2 km22 +
    k11 km12^2 km22 + k21 km11 km21 km22 + k22 km11 km21 km22 + km11^2 km21 km22 +
    k21 km12 km21 km22 + k22 km12 km21 km22 + 2 km11 km12 km21 km22 + km12^2 km21 km22)
```

In[36]:=

```
Pplusfunc = Function[s, (Omegaplus[s].Pbarev0)⟦1, 1⟧ + (Omegaplus[s].Pbarev0)⟦2, 1⟧]
```

Out[36]=

```
Function[s, (Omegaplus[s].Pbarev0)⟦1, 1⟧ + (Omegaplus[s].Pbarev0)⟦2, 1⟧]
```

In[37]:=

```
Simplify[Together[Pplusfunc[s]]]
```

Out[37]=

```
((k21 + k22)
    (k11^2 k12^2 k21^3 + 3 k11^2 k12^2 k21^2 k22 + 3 k11^2 k12^2 k21 k22^2 + k11^2 k12^2 k22^3 + 2 k11^2 k12^2
        k21^2 km11 + 4 k11^2 k12^2 k21 k22 km11 + 2 k11^2 k12^2 k22^2 km11 + k11^2 k12^2 k21 km11^2 +
      k11^2 k12^2 k22 km11^2 + 2 k11^2 k12^2 k21^2 km12 + 4 k11^2 k12^2 k21 k22 km12 +
      2 k11^2 k12^2 k22^2 km12 + 2 k11^2 k12^2 k21 km11 km12 + 2 k11^2 k12^2 k22 km11 km12 +
      k11^2 k12^2 k21 km12^2 + k11^2 k12^2 k22 km12^2 + 2 k11 k12^2 k21^2 k22 km21 +
      4 k11 k12^2 k21 k22^2 km21 + 2 k11 k12^2 k22^3 km21 + k11 k12^2 k21^2 km11 km21 +
      4 k11 k12^2 k21 k22 km11 km21 + 3 k11 k12^2 k22^2 km11 km21 + 2 k11 k12^2 k21 km11^2 km21 +
      2 k11 k12^2 k22 km11^2 km21 + k11 k12^2 km11^3 km21 + 2 k11 k12^2 k21^2 km12 km21 +
      6 k11 k12^2 k21 k22 km12 km21 + 4 k11 k12^2 k22^2 km12 km21 + 4 k11 k12^2 k21 km11 km12 km21 +
      4 k11 k12^2 k22 km11 km12 km21 + 2 k11 k12^2 km11^2 km12 km21 + 2 k11 k12^2 k21 km12^2 km21 +
      2 k11 k12^2 k22 km12^2 km21 + k11 k12^2 km11 km12^2 km21 + k12^2 k21 k22^2 km21^2 +
      k12^2 k22^3 km21^2 + k12^2 k21 k22 km11 km21^2 + k12^2 k22^2 km11 km21^2 + k12^2 k22 km11^2 km21^2 +
      2 k12^2 k21 k22 km12 km21^2 + 2 k12^2 k22^2 km12 km21^2 + k12^2 k21 km11 km12 km21^2 +
      2 k12^2 k22 km11 km12 km21^2 + k12^2 km11^2 km12 km21^2 + k12^2 k21 km12^2 km21^2 +
```

$k12^2 k22 km12^2 km21^2 + k12^2 km11 km12^2 km21^2 + 2 k11^2 k12 k21^3 km22 +$
$4 k11^2 k12 k21^2 k22 km22 + 2 k11^2 k12 k21 k22^2 km22 + 4 k11^2 k12 k21^2 km11 km22 +$
$6 k11^2 k12 k21 k22 km11 km22 + 2 k11^2 k12 k22^2 km11 km22 + 2 k11^2 k12 k21 km11^2 km22 +$
$2 k11^2 k12 k22 km11^2 km22 + 3 k11^2 k12 k21^2 km12 km22 + 4 k11^2 k12 k21 k22 km12 km22 +$
$k11^2 k12 k22^2 km12 km22 + 4 k11^2 k12 k21 km11 km12 km22 + 4 k11^2 k12 k22 km11 km12 km22 +$
$k11^2 k12 km11^2 km12 km22 + 2 k11^2 k12 k21 km12^2 km22 + 2 k11^2 k12 k22 km12^2 km22 +$
$2 k11^2 k12 km11 km12^2 km22 + k11^2 k12 km12^3 km22 + 2 k11 k12 k21^2 k22 km21 km22 +$
$2 k11 k12 k21 k22^2 km21 km22 + 2 k11 k12 k21^2 km11 km21 km22 +$
$5 k11 k12 k21 k22 km11 km21 km22 + 3 k11 k12 k22^2 km11 km21 km22 +$
$4 k11 k12 k21 km11^2 km21 km22 + 3 k11 k12 k22 km11^2 km21 km22 +$
$2 k11 k12 km11^3 km21 km22 + 3 k11 k12 k21^2 km12 km21 km22 +$
$5 k11 k12 k21 k22 km12 km21 km22 + 2 k11 k12 k22^2 km12 km21 km22 +$
$7 k11 k12 k21 km11 km12 km21 km22 + 7 k11 k12 k22 km11 km12 km21 km22 +$
$4 k11 k12 km11^2 km12 km21 km22 + 3 k11 k12 k21 km12^2 km21 km22 +$
$4 k11 k12 k22 km12^2 km21 km22 + 4 k11 k12 km11 km12^2 km21 km22 +$
$2 k11 k12 km12^3 km21 km22 + k12 k21 k22 km11 km21^2 km22 + k12 k22^2 km11 km21^2 km22 +$
$k12 k22 km11^2 km21^2 km22 + k12 k21 k22 km12 km21^2 km22 + k12 k22^2 km12 km21^2 km22 +$
$k12 k21 km11 km12 km21^2 km22 + 3 k12 k22 km11 km12 km21^2 km22 +$
$k12 km11^2 km12 km21^2 km22 + k12 k21 km12^2 km21^2 km22 + 2 k12 k22 km12^2 km21^2 km22 +$
$2 k12 km11 km12^2 km21^2 km22 + k12 km12^3 km21^2 km22 + k11^2 k21^3 km22^2 +$
$k11^2 k21^2 k22 km22^2 + 2 k11^2 k21^2 km11 km22^2 + 2 k11^2 k21 k22 km11 km22^2 +$
$k11^2 k21 km11^2 km22^2 + k11^2 k22 km11^2 km22^2 + k11^2 k21^2 km12 km22^2 +$
$k11^2 k21 k22 km12 km22^2 + 2 k11^2 k21 km11 km12 km22^2 + k11^2 k22 km11 km12 km22^2 +$
$k11^2 km11^2 km12 km22^2 + k11^2 k21 km12^2 km22^2 + k11^2 km11 km12^2 km22^2 +$
$k11 k21^2 km11 km21 km22^2 + k11 k21 k22 km11 km21 km22^2 + 2 k11 k21 km11^2 km21 km22^2 +$
$k11 k22 km11^2 km21 km22^2 + k11 km11^3 km21 km22^2 + k11 k21^2 km12 km21 km22^2 +$
$k11 k21 k22 km12 km21 km22^2 + 3 k11 k21 km11 km12 km21 km22^2 +$
$k11 k22 km11 km12 km21 km22^2 + 2 k11 km11^2 km12 km21 km22^2 + k11 k21 km12^2 km21 km22^2 +$
$k11 km11 km12^2 km21 km22^2 + k11^2 k12^2 k21^2 s + k11^2 k12 k21^3 s + 2 k11^2 k12^2 k21 k22 s +$
$2 k11^2 k12 k21^2 k22 s + k11 k12^2 k21^2 k22 s + k11^2 k12^2 k22^2 s + k11^2 k12 k21 k22^2 s +$
$2 k11 k12^2 k21 k22^2 s + k11 k12^2 k22^3 s + k11^2 k12^2 k21 km11 s + 2 k11^2 k12 k21^2 km11 s +$
$k11^2 k12^2 k22 km11 s + 2 k11^2 k12 k21 k22 km11 s + 2 k11 k12^2 k21 k22 km11 s +$
$2 k11 k12^2 k22^2 km11 s + k11^2 k12 k21 km11^2 s + k11 k12^2 k22 km11^2 s +$
$k11^2 k12^2 k21 km12 s + 2 k11^2 k12 k21^2 km12 s + k11^2 k12^2 k22 km12 s +$
$2 k11^2 k12 k21 k22 km12 s + 2 k11 k12^2 k21 k22 km12 s + 2 k11 k12^2 k22^2 km12 s +$
$2 k11^2 k12 k21 km11 km12 s + 2 k11 k12^2 k22 km11 km12 s + k11^2 k12 k21 km12^2 s +$
$k11 k12^2 k22 km12^2 s + 2 k11 k12^2 k21 k22 km21 s + k11 k12 k21^2 k22 km21 s +$
$2 k11 k12^2 k22^2 km21 s + k11 k12 k21 k22^2 km21 s + k12^2 k21 k22^2 km21 s +$
$k12^2 k22^3 km21 s + k11 k12^2 k21 km11 km21 s + k11 k12 k21^2 km11 km21 s +$
$k11 k12^2 k22 km11 km21 s + 2 k11 k12 k21 k22 km11 km21 s + k12^2 k22^2 km11 km21 s +$
$k11 k12^2 km11^2 km21 s + 2 k11 k12 k21 km11^2 km21 s + k11 k12 k22 km11^2 km21 s +$
$k11 k12 km11^3 km21 s + 2 k11 k12^2 k21 km12 km21 s + k11 k12 k21^2 km12 km21 s +$
$k12^2 k21^2 km12 km21 s + 2 k11 k12^2 k22 km12 km21 s + 2 k11 k12 k21 k22 km12 km21 s +$
$2 k12^2 k21 k22 km12 km21 s + 2 k12^2 k22^2 km12 km21 s + k11 k12^2 km11 km12 km21 s +$

$$2\ k11\ k12\ k21\ km11\ km12\ km21\ s + 2\ k12^2\ k21\ km11\ km12\ km21\ s +$$
$$2\ k12^2\ k22\ km11\ km12\ km21\ s + k11\ k12\ km11^2\ km12\ km21\ s + k12^2\ km11^2\ km12\ km21\ s +$$
$$k11\ k12\ k21\ km12^2\ km21\ s + k12^2\ k21\ km12^2\ km21\ s + k12^2\ k22\ km12^2\ km21\ s +$$
$$k12^2\ km11\ km12^2\ km21\ s + k12^2\ k22^2\ km21^2\ s + k12^2\ k21\ km12\ km21^2\ s +$$
$$k12^2\ k22\ km12\ km21^2\ s + k12^2\ km11\ km12\ km21^2\ s + 2\ k11^2\ k12\ k21^2\ km22\ s + k11^2\ k21^3\ km22\ s +$$
$$2\ k11^2\ k12\ k21\ k22\ km22\ s + k11^2\ k21^2\ k22\ km22\ s + k11\ k12\ k21^2\ k22\ km22\ s +$$
$$k11\ k12\ k21\ k22^2\ km22\ s + 2\ k11^2\ k12\ k21\ km11\ km22\ s + 2\ k11^2\ k21^2\ km11\ km22\ s +$$
$$2\ k11^2\ k12\ k22\ km11\ km22\ s + 2\ k11^2\ k21\ k22\ km11\ km22\ s + 2\ k11\ k12\ k21\ k22\ km11\ km22\ s +$$
$$k11^2\ k22^2\ km11\ km22\ s + k11\ k12\ k22^2\ km11\ km22\ s + k11^2\ k21\ km11^2\ km22\ s +$$
$$k11^2\ k22\ km11^2\ km22\ s + k11\ k12\ k22\ km11^2\ km22\ s + k11^2\ k12\ k21\ km12\ km22\ s +$$
$$k11^2\ k21^2\ km12\ km22\ s + k11^2\ k12\ k22\ km12\ km22\ s + 2\ k11\ k12\ k21\ k22\ km12\ km22\ s +$$
$$k11\ k12\ k22^2\ km12\ km22\ s + k11^2\ k12\ km11\ km12\ km22\ s + 2\ k11^2\ k21\ km11\ km12\ km22\ s +$$
$$2\ k11^2\ k22\ km11\ km12\ km22\ s + 2\ k11\ k12\ k22\ km11\ km12\ km22\ s + k11^2\ km11^2\ km12\ km22\ s +$$
$$k11^2\ k12\ km12^2\ km22\ s + k11\ k12\ k21\ km12^2\ km22\ s + 2\ k11\ k12\ k22\ km12^2\ km22\ s +$$
$$k11^2\ km11\ km12^2\ km22\ s + k11\ k12\ km11\ km12^2\ km22\ s + k11\ k12\ km12^3\ km22\ s +$$
$$2\ k11\ k12\ k21\ k22\ km21\ km22\ s + 2\ k11\ k12\ k21\ km11\ km21\ km22\ s +$$
$$k11\ k21^2\ km11\ km21\ km22\ s + 2\ k11\ k12\ k22\ km11\ km21\ km22\ s +$$
$$2\ k11\ k21\ k22\ km11\ km21\ km22\ s + k11\ k22^2\ km11\ km21\ km22\ s +$$
$$2\ k11\ k12\ km11^2\ km21\ km22\ s + 2\ k11\ k21\ km11^2\ km21\ km22\ s + 2\ k11\ k22\ km11^2\ km21\ km22\ s +$$
$$k11\ km11^3\ km21\ km22\ s + 2\ k11\ k12\ k21\ km12\ km21\ km22\ s + k12\ k21^2\ km12\ km21\ km22\ s +$$
$$2\ k11\ k12\ k22\ km12\ km21\ km22\ s + 2\ k12\ k21\ k22\ km12\ km21\ km22\ s +$$
$$k12\ k22^2\ km12\ km21\ km22\ s + 2\ k11\ k12\ km11\ km12\ km21\ km22\ s +$$
$$2\ k11\ k21\ km11\ km12\ km21\ km22\ s + 2\ k12\ k21\ km11\ km12\ km21\ km22\ s +$$
$$2\ k11\ k22\ km11\ km12\ km21\ km22\ s + 2\ k12\ k22\ km11\ km12\ km21\ km22\ s +$$
$$2\ k11\ km11^2\ km12\ km21\ km22\ s + k12\ km11^2\ km12\ km21\ km22\ s + 2\ k11\ k12\ km12^2\ km21\ km22\ s +$$
$$2\ k12\ k21\ km12^2\ km21\ km22\ s + 2\ k12\ k22\ km12^2\ km21\ km22\ s + k11\ km11\ km12^2\ km21\ km22\ s +$$
$$2\ k12\ km11\ km12^2\ km21\ km22\ s + k12\ km12^3\ km21\ km22\ s + k12\ k21\ km12\ km21^2\ km22\ s +$$
$$k12\ k22\ km12\ km21^2\ km22\ s + k12\ km11\ km12\ km21^2\ km22\ s + k12\ km12^2\ km21^2\ km22\ s +$$
$$k11^2\ k21^2\ km22^2\ s + k11^2\ k21\ km11\ km22^2\ s + k11^2\ k22\ km11\ km22^2\ s +$$
$$k11^2\ km11\ km12\ km22^2\ s + k11\ k21\ km11\ km21\ km22^2\ s + k11\ k22\ km11\ km21\ km22^2\ s +$$
$$k11\ km11^2\ km21\ km22^2\ s + k11\ km11\ km12\ km21\ km22^2\ s + k11^2\ k12\ k21^2\ s^2 +$$
$$k11^2\ k12\ k21\ k22\ s^2 + k11\ k12^2\ k21\ k22\ s^2 + k11\ k12^2\ k22^2\ s^2 + k11^2\ k12\ k21\ km11\ s^2 +$$
$$k11\ k12^2\ k22\ km11\ s^2 + k11^2\ k12\ k21\ km12\ s^2 + k11\ k12^2\ k22\ km12\ s^2 +$$
$$k11\ k12\ k21\ k22\ km21\ s^2 + k12^2\ k22^2\ km21\ s^2 + k11\ k12\ k21\ km11\ km21\ s^2 +$$
$$k11\ k12\ km11^2\ km21\ s^2 + k11\ k12\ k21\ km12\ km21\ s^2 + k12^2\ k21\ km12\ km21\ s^2 +$$
$$k12^2\ k22\ km12\ km21\ s^2 + k12^2\ km11\ km12\ km21\ s^2 + k11^2\ k21^2\ km22\ s^2 +$$
$$k11\ k12\ k21\ k22\ km22\ s^2 + k11^2\ k21\ km11\ km22\ s^2 + k11^2\ k22\ km11\ km22\ s^2 +$$
$$k11\ k12\ k22\ km11\ km22\ s^2 + k11\ k12\ k22\ km12\ km22\ s^2 + k11^2\ km11\ km12\ km22\ s^2 +$$
$$k11\ k12\ km12^2\ km22\ s^2 + k11\ k21\ km11\ km21\ km22\ s^2 + k11\ k22\ km11\ km21\ km22\ s^2 +$$
$$k11\ km11^2\ km21\ km22\ s^2 + k12\ k21\ km12\ km21\ km22\ s^2 + k12\ k22\ km12\ km21\ km22\ s^2 +$$
$$k11\ km11\ km12\ km21\ km22\ s^2 + k12\ km11\ km12\ km21\ km22\ s^2 + k12\ km12^2\ km21\ km22\ s^2 +$$
$$gammam1^2\ k11\ (k21 + k22 + km11 + km12)\ (k11\ (k21 + k22) + (km11 + km12)\ km21)$$
$$(k21 + k22 + km11 + km12 + s) + gamma1^2\ k12\ (k21 + k22 + km11 + km12)$$
$$(k12\ (k21 + k22) + (km11 + km12)\ km22)\ (k21 + k22 + km11 + km12 + s) +$$

```
gamma1 (k12 (k12 (k21 + k22 + km11 + km12 + s) (km11 (km11 + km12) km21 +
        k21 (km11 + 2 km12) km21 + k22 km11 (km21 + s) + k21 k22 (2 km21 + s) +
        k22^2 (2 km21 + s) + k22 km12 (2 km21 + s)) + (k21 + k22 + km11 + km12)
      km22 (k21 km11 km21 + k21 km12 (km21 + s) + (km11 + km12 + s)
         (km11 km21 + km12 (2 km21 + s)) + k22 (2 km11 km21 + km12 (2 km21 + s)))) +
   k11 (2 k12^2 (k21 + k22) (k21 + k22 + km11 + km12) (k21 + k22 + km11 + km12 + s) +
      (k21 + k22 + km11 + km12) km22 (k21 (km12 km22 + km11 (km22 + s)) +
        km11 (km11 (km22 + s) + km12 (km22 + s) + s (k22 + km22 + s))) +
      k12 (k21 + k22 + km11 + km12 + s) ((3 k22 km11 + km11^2 + 2 k22 km12 +
           3 km11 km12 + 2 km12^2) km22 + k21^2 (2 km22 + s) +
        k21 (3 km11 km22 + 2 km12 km22 + km11 s + km12 s + k22 (2 km22 + s))))) +
gammam1 (gamma1 (k21 + k22 + km11 + km12) (2 k11 k12 (k21 + k22) +
      k12 (km11 + km12) km21 + k11 (km11 + km12) km22) (k21 + k22 + km11 + km12 + s) +
   k11^2 (k21 + k22 + km11 + km12 + s) (2 k12 (k21 + k22) (k21 + k22 + km11 + km12) +
      km12 (km11 + km12) km22 + k22 (2 km11 + km12) km22 + k21 km12 (km22 + s) +
      k21^2 (2 km22 + s) + k21 k22 (2 km22 + s) + k21 km11 (2 km22 + s)) +
   k12 (k21 + k22 + km11 + km12) km21 (k22 (km11 km21 + km12 (km21 + s)) +
      km12 (km11 (km21 + s) + km12 (km21 + s) + s (k21 + km21 + s))) +
   k11 (k12 (k21 + k22 + km11 + km12 + s) ((2 km11^2 + 3 km11 km12 + km12^2) km21 +
        k22^2 (2 km21 + s) + k21 (2 k22 km21 + 2 km11 km21 + 3 km12 km21 + k22 s) +
        k22 (2 km11 km21 + 3 km12 km21 + km11 s + km12 s)) + (k21 + k22 + km11 + km12)
      km21 (k22 (km12 km22 + km11 (km22 + s)) + (km11 + km12 + s) (km12 km22 +
           km11 (2 km22 + s)) + k21 (2 km12 km22 + km11 (2 km22 + s)))))) /
((k11 k12 k21^2 + 2 k11 k12 k21 k22 + k11 k12 k22^2 + k11 k12 k21 km11 + k11 k12 k22 km11 +
   k11 k12 k21 km12 + k11 k12 k22 km12 + k12 k21 k22 km21 +
   k12 k22^2 km21 + k12 k21 km11 km21 + k12 km11^2 km21 +
   2 k12 k21 km12 km21 + k12 k22 km12 km21 + k12 km11 km12 km21 +
   gammam1 (k21 + k22 + km11 + km12) (k11 (k21 + k22) + (km11 + km12) km21) +
   k11 k21^2 km22 + k11 k21 k22 km22 + k11 k21 km11 km22 + 2 k11 k22 km11 km22 +
   k11 k22 km12 km22 + k11 km11 km12 km22 + k11 km12^2 km22 + k21 km11 km21 km22 +
   k22 km11 km21 km22 + km11^2 km21 km22 + k21 km12 km21 km22 +
   k22 km12 km21 km22 + 2 km11 km12 km21 km22 + km12^2 km21 km22 +
   gamma1 (k21 + k22 + km11 + km12) (k12 (k21 + k22) + (km11 + km12) km22))
  (k11 k12 k21^2 + 2 k11 k12 k21 k22 + k11 k12 k22^2 + k11 k12 k21 km11 +
   k11 k12 k22 km11 + k11 k12 k21 km12 + k11 k12 k22 km12 + k12 k21 k22 km21 +
   k12 k22^2 km21 + k12 k21 km11 km21 + k12 k22 km11 km21 + k12 km11^2 km21 +
   k12 k21 km12 km21 + k12 k22 km12 km21 + k12 km11 km12 km21 +
   k11 k21^2 km22 + k11 k21 k22 km22 + k11 k21 km11 km22 + k11 k22 km11 km22 +
   k11 k21 km12 km22 + k11 k22 km12 km22 + k11 km11 km12 km22 +
   k11 km12^2 km22 + k21 km11 km21 km22 + k22 km11 km21 km22 + km11^2 km21 km22 +
   k21 km12 km21 km22 + k22 km12 km21 km22 + 2 km11 km12 km21 km22 +
   km12^2 km21 km22 + 2 k11 k12 k21 s + k11 k21^2 s + k12 k21^2 s +
```

```
2 k11 k12 k22 s + 2 k11 k21 k22 s + 2 k12 k21 k22 s + k11 k22^2 s +
k12 k22^2 s + k11 k12 km11 s + k11 k21 km11 s + 2 k12 k21 km11 s +
k11 k22 km11 s + 2 k12 k22 km11 s + k12 km11^2 s + k11 k12 km12 s +
2 k11 k21 km12 s + k12 k21 km12 s + 2 k11 k22 km12 s + k12 k22 km12 s +
k11 km11 km12 s + k12 km11 km12 s + k11 km12^2 s + k12 k21 km21 s +
2 k12 k22 km21 s + k21 k22 km21 s + k22^2 km21 s + 2 k12 km11 km21 s +
k21 km11 km21 s + 2 k22 km11 km21 s + km11^2 km21 s + k12 km12 km21 s +
k21 km12 km21 s + 2 k22 km12 km21 s + 2 km11 km12 km21 s + km12^2 km21 s +
2 k11 k21 km22 s + k21^2 km22 s + k11 k22 km22 s + k21 k22 km22 s +
k11 km11 km22 s + 2 k21 km11 km22 s + k22 km11 km22 s + km11^2 km22 s +
2 k11 km12 km22 s + 2 k21 km12 km22 s + k22 km12 km22 s + 2 km11 km12 km22 s +
km12^2 km22 s + k21 km21 km22 s + k22 km21 km22 s + 2 km11 km21 km22 s +
2 km12 km21 km22 s + k11 k12 s^2 + 2 k11 k21 s^2 + 2 k12 k21 s^2 + k21^2 s^2 +
2 k11 k22 s^2 + 2 k12 k22 s^2 + 2 k21 k22 s^2 + k22^2 s^2 + k11 km11 s^2 +
2 k12 km11 s^2 + 2 k21 km11 s^2 + 2 k22 km11 s^2 + km11^2 s^2 + 2 k11 km12 s^2 +
k12 km12 s^2 + 2 k21 km12 s^2 + 2 k22 km12 s^2 + 2 km11 km12 s^2 + km12^2 s^2 +
k12 km21 s^2 + k21 km21 s^2 + 2 k22 km21 s^2 + 2 km11 km21 s^2 + 2 km12 km21 s^2 +
k11 km22 s^2 + 2 k21 km22 s^2 + k22 km22 s^2 + 2 km11 km22 s^2 + 2 km12 km22 s^2 +
km21 km22 s^2 + k11 s^3 + k12 s^3 + 2 k21 s^3 + 2 k22 s^3 + 2 km11 s^3 +
2 km12 s^3 + km21 s^3 + km22 s^3 + s^4 + gammam1 (k21 + k22 + km11 + km12 + s)
  (km12 km21 + k21 s + k22 s + km12 s + km21 s + s^2 + k11 (k21 + k22 + s) + km11 (km21 + s)) +
gamma1 (k21 + k22 + km11 + km12 + s)
  (km12 km22 + k21 s + k22 s + km12 s + km22 s + s^2 + k12 (k21 + k22 + s) + km11 (km22 + s))))
```

In[38]:=
```
Pplus = Function[s,
  ((k21 + k22) (k11^2 k12^2 k21^3 + 3 k11^2 k12^2 k21^2 k22 + 3 k11^2 k12^2 k21 k22^2 + k11^2 k12^2 k22^3 +
      2 k11^2 k12^2 k21^2 km11 + 4 k11^2 k12^2 k21 k22 km11 + 2 k11^2 k12^2 k22^2 km11 +
      k11^2 k12^2 k21 km11^2 + k11^2 k12^2 k22 km11^2 + 2 k11^2 k12^2 k21^2 km12 +
      4 k11^2 k12^2 k21 k22 km12 + 2 k11^2 k12^2 k22^2 km12 + 2 k11^2 k12^2 k21 km11 km12 +
      2 k11^2 k12^2 k22 km11 km12 + k11^2 k12^2 k21 km12^2 + k11^2 k12^2 k22 km12^2 +
      2 k11 k12^2 k21^2 k22 km21 + 4 k11 k12^2 k21 k22^2 km21 + 2 k11 k12^2 k22^3 km21 +
      k11 k12^2 k21^2 km11 km21 + 4 k11 k12^2 k21 k22 km11 km21 + 3 k11 k12^2 k22^2 km11 km21 +
      2 k11 k12^2 k21 km11^2 km21 + 2 k11 k12^2 k22 km11^2 km21 + k11 k12^2 km11^3 km21 +
      2 k11 k12^2 k21^2 km12 km21 + 6 k11 k12^2 k21 k22 km12 km21 + 4 k11 k12^2 k22^2 km12 km21 +
      4 k11 k12^2 k21 km11 km12 km21 + 4 k11 k12^2 k22 km11 km12 km21 +
      2 k11 k12^2 km11^2 km12 km21 + 2 k11 k12^2 k21 km12^2 km21 +
      2 k11 k12^2 k22 km12^2 km21 + k11 k12^2 km11 km12^2 km21 + k12^2 k21 k22^2 km21^2 +
      k12^2 k22^3 km21^2 + k12^2 k21 k22 km11 km21^2 + k12^2 k22^2 km11 km21^2 +
      k12^2 k22 km11^2 km21^2 + 2 k12^2 k21 k22 km12 km21^2 + 2 k12^2 k22^2 km12 km21^2 +
      k12^2 k21 km11 km12 km21^2 + 2 k12^2 k22 km11 km12 km21^2 + k12^2 km11^2 km12 km21^2 +
      k12^2 k21 km12^2 km21^2 + k12^2 k22 km12^2 km21^2 + k12^2 km11 km12^2 km21^2 +
      2 k11^2 k12 k21^3 km22 + 4 k11^2 k12 k21^2 k22 km22 + 2 k11^2 k12 k21 k22^2 km22 +
      4 k11^2 k12 k21^2 km11 km22 + 6 k11^2 k12 k21 k22 km11 km22 +
```

$2 k11^2 k12 k22^2 km11 km22 + 2 k11^2 k12 k21 km11^2 km22 + 2 k11^2 k12 k22 km11^2 km22 +$
$3 k11^2 k12 k21^2 km12 km22 + 4 k11^2 k12 k21 k22 km12 km22 + k11^2 k12 k22^2 km12 km22 +$
$4 k11^2 k12 k21 km11 km12 km22 + 4 k11^2 k12 k22 km11 km12 km22 +$
$k11^2 k12 km11^2 km12 km22 + 2 k11^2 k12 k21 km12^2 km22 + 2 k11^2 k12 k22 km12^2 km22 +$
$2 k11^2 k12 km11 km12^2 km22 + k11^2 k12 km12^3 km22 + 2 k11 k12 k21^2 k22 km21 km22 +$
$2 k11 k12 k21 k22^2 km21 km22 + 2 k11 k12 k21^2 km11 km21 km22 +$
$5 k11 k12 k21 k22 km11 km21 km22 + 3 k11 k12 k22^2 km11 km21 km22 +$
$4 k11 k12 k21 km11^2 km21 km22 + 3 k11 k12 k22 km11^2 km21 km22 +$
$2 k11 k12 km11^3 km21 km22 + 3 k11 k12 k21^2 km12 km21 km22 +$
$5 k11 k12 k21 k22 km12 km21 km22 + 2 k11 k12 k22^2 km12 km21 km22 +$
$7 k11 k12 k21 km11 km12 km21 km22 + 7 k11 k12 k22 km11 km12 km21 km22 +$
$4 k11 k12 km11^2 km12 km21 km22 + 3 k11 k12 k21 km12^2 km21 km22 +$
$4 k11 k12 k22 km12^2 km21 km22 + 4 k11 k12 km11 km12^2 km21 km22 +$
$2 k11 k12 km12^3 km21 km22 + k12 k21 k22 km11 km21^2 km22 + k12 k22^2 km11 km21^2 km22 +$
$k12 k22 km11^2 km21^2 km22 + k12 k21 k22 km12 km21^2 km22 + k12 k22^2 km12 km21^2 km22 +$
$k12 k21 km11 km12 km21^2 km22 + 3 k12 k22 km11 km12 km21^2 km22 +$
$k12 km11^2 km12 km21^2 km22 + k12 k21 km12^2 km21^2 km22 + 2 k12 k22 km12^2 km21^2 km22 +$
$2 k12 km11 km12^2 km21^2 km22 + k12 km12^3 km21^2 km22 + k11^2 k21^3 km22^2 +$
$k11^2 k21^2 k22 km22^2 + 2 k11^2 k21^2 km11 km22^2 + 2 k11^2 k21 k22 km11 km22^2 +$
$k11^2 k21 km11^2 km22^2 + k11^2 k22 km11^2 km22^2 + k11^2 k21^2 km12 km22^2 +$
$k11^2 k21 k22 km12 km22^2 + 2 k11^2 k21 km11 km12 km22^2 + k11^2 k22 km11 km12 km22^2 +$
$k11^2 km11^2 km12 km22^2 + k11^2 k21 km12^2 km22^2 + k11^2 km11 km12^2 km22^2 +$
$k11 k21^2 km11 km21 km22^2 + k11 k21 k22 km11 km21 km22^2 + 2 k11 k21 km11^2 km21 km22^2 +$
$k11 k22 km11^2 km21 km22^2 + k11 km11^3 km21 km22^2 + k11 k21^2 km12 km21 km22^2 +$
$k11 k21 k22 km12 km21 km22^2 + 3 k11 k21 km11 km12 km21 km22^2 +$
$k11 k22 km11 km12 km21 km22^2 + 2 k11 km11^2 km12 km21 km22^2 +$
$k11 k21 km12^2 km21 km22^2 + k11 km11 km12^2 km21 km22^2 + k11^2 k12^2 k21^2 s +$
$k11^2 k12 k21^3 s + 2 k11^2 k12^2 k21 k22 s + 2 k11^2 k12 k21^2 k22 s + k11 k12^2 k21^2 k22 s +$
$k11^2 k12^2 k22^2 s + k11^2 k12 k21 k22^2 s + 2 k11 k12^2 k21 k22^2 s + k11 k12^2 k22^3 s +$
$k11^2 k12^2 k21 km11 s + 2 k11^2 k12 k21^2 km11 s + k11^2 k12^2 k22 km11 s +$
$2 k11^2 k12 k21 k22 km11 s + 2 k11 k12^2 k21 k22 km11 s + 2 k11 k12^2 k22^2 km11 s +$
$k11^2 k12 k21 km11^2 s + k11 k12^2 k22 km11^2 s + k11^2 k12^2 k21 km12 s +$
$2 k11^2 k12 k21^2 km12 s + k11^2 k12^2 k22 km12 s + 2 k11^2 k12 k21 k22 km12 s +$
$2 k11 k12^2 k21 k22 km12 s + 2 k11 k12^2 k22^2 km12 s + 2 k11^2 k12 k21 km11 km12 s +$
$2 k11 k12^2 k22 km11 km12 s + k11^2 k12 k21 km12^2 s + k11 k12^2 k22 km12^2 s +$
$2 k11 k12^2 k21 k22 km21 s + k11 k12 k21^2 k22 km21 s + 2 k11 k12^2 k22^2 km21 s +$
$k11 k12 k21 k22^2 km21 s + k12^2 k21 k22^2 km21 s + k12^2 k22^3 km21 s +$
$k11 k12^2 k21 km11 km21 s + k11 k12 k21^2 km11 km21 s + k11 k12^2 k22 km11 km21 s +$
$2 k11 k12 k21 k22 km11 km21 s + k12^2 k22^2 km11 km21 s + k11 k12^2 km11^2 km21 s +$
$2 k11 k12 k21 km11^2 km21 s + k11 k12 k22 km11^2 km21 s + k11 k12 km11^3 km21 s +$
$2 k11 k12^2 k21 km12 km21 s + k11 k12 k21^2 km12 km21 s + k12^2 k21^2 km12 km21 s +$
$2 k11 k12^2 k22 km12 km21 s + 2 k11 k12 k21 k22 km12 km21 s + 2 k12^2 k21 k22 km12 km21 s +$
$2 k12^2 k22^2 km12 km21 s + k11 k12^2 km11 km12 km21 s + 2 k11 k12 k21 km11 km12 km21 s +$
$2 k12^2 k21 km11 km12 km21 s + 2 k12^2 k22 km11 km12 km21 s + k11 k12 km11^2 km12 km21 s +$

```
k12^2 km11^2 km12 km21 s + k11 k12 k21 km12^2 km21 s + k12^2 k21 km12^2 km21 s +
k12^2 k22 km12^2 km21 s + k12^2 km11 km12^2 km21 s + k12^2 k22^2 km21^2 s +
k12^2 k21 km12 km21^2 s + k12^2 k22 km12 km21^2 s + k12^2 km11 km12 km21^2 s +
2 k11^2 k12 k21^2 km22 s + k11^2 k21^3 km22 s + 2 k11^2 k12 k21 k22 km22 s +
k11^2 k21^2 k22 km22 s + k11 k12 k21^2 k22 km22 s + k11 k12 k21 k22^2 km22 s +
2 k11^2 k12 k21 km11 km22 s + 2 k11^2 k21^2 km11 km22 s + 2 k11^2 k12 k22 km11 km22 s +
2 k11^2 k21 k22 km11 km22 s + 2 k11 k12 k21 k22 km11 km22 s + k11^2 k22^2 km11 km22 s +
k11 k12 k22^2 km11 km22 s + k11^2 k21 km11^2 km22 s + k11^2 k22 km11^2 km22 s +
k11 k12 k22 km11^2 km22 s + k11^2 k12 k21 km12 km22 s + k11^2 k21^2 km12 km22 s +
k11^2 k12 k22 km12 km22 s + 2 k11 k12 k21 k22 km12 km22 s + k11 k12 k22^2 km12 km22 s +
k11^2 k12 km11 km12 km22 s + 2 k11^2 k21 km11 km12 km22 s + 2 k11^2 k22 km11 km12 km22 s +
2 k11 k12 k22 km11 km12 km22 s + k11^2 km11^2 km12 km22 s + k11^2 k12 km12^2 km22 s +
k11 k12 k21 km12^2 km22 s + 2 k11 k12 k22 km12^2 km22 s + k11^2 km11 km12^2 km22 s +
k11 k12 km11 km12^2 km22 s + k11 k12 km12^3 km22 s + 2 k11 k12 k21 k22 km21 km22 s +
2 k11 k12 k21 km11 km21 km22 s + k11 k21^2 km11 km21 km22 s +
2 k11 k12 k22 km11 km21 km22 s + 2 k11 k21 k22 km11 km21 km22 s +
k11 k22^2 km11 km21 km22 s + 2 k11 k12 km11^2 km21 km22 s + 2 k11 k21 km11^2 km21 km22 s +
2 k11 k22 km11^2 km21 km22 s + k11 km11^3 km21 km22 s + 2 k11 k12 k21 km12 km21 km22 s +
k12 k21^2 km12 km21 km22 s + 2 k11 k12 k22 km12 km21 km22 s +
2 k12 k21 k22 km12 km21 km22 s + k12 k22^2 km12 km21 km22 s +
2 k11 k12 km11 km12 km21 km22 s + 2 k11 k21 km11 km12 km21 km22 s +
2 k12 k21 km11 km12 km21 km22 s + 2 k11 k22 km11 km12 km21 km22 s +
2 k12 k22 km11 km12 km21 km22 s + 2 k11 km11^2 km12 km21 km22 s +
k12 km11^2 km12 km21 km22 s + 2 k11 k12 km12^2 km21 km22 s +
2 k12 k21 km12^2 km21 km22 s + 2 k12 k22 km12^2 km21 km22 s + k11 km11 km12^2 km21 km22 s +
2 k12 km11 km12^2 km21 km22 s + k12 km12^3 km21 km22 s + k12 k21 km12 km21^2 km22 s +
k12 k22 km12 km21^2 km22 s + k12 km11 km12 km21^2 km22 s + k12 km12^2 km21^2 km22 s +
k11^2 k21^2 km22^2 s + k11^2 k21 km11 km22^2 s + k11^2 k22 km11 km22^2 s +
k11^2 km11 km12 km22^2 s + k11 k21 km11 km21 km22^2 s + k11 k22 km11 km21 km22^2 s +
k11 km11^2 km21 km22^2 s + k11 km11 km12 km21 km22^2 s + k11^2 k12 k21^2 s^2 +
k11^2 k12 k21 k22 s^2 + k11 k12^2 k21 k22 s^2 + k11 k12^2 k22^2 s^2 + k11^2 k12 k21 km11 s^2 +
k11 k12^2 k22 km11 s^2 + k11^2 k12 k21 km12 s^2 + k11 k12^2 k22 km12 s^2 +
k11 k12 k21 k22 km21 s^2 + k12^2 k22^2 km21 s^2 + k11 k12 k21 km11 km21 s^2 +
k11 k12 km11^2 km21 s^2 + k11 k12 k21 km12 km21 s^2 + k12^2 k21 km12 km21 s^2 +
k12^2 k22 km12 km21 s^2 + k12^2 km11 km12 km21 s^2 + k11^2 k21^2 km22 s^2 +
k11 k12 k21 k22 km22 s^2 + k11^2 k21 km11 km22 s^2 + k11^2 k22 km11 km22 s^2 +
k11 k12 k22 km11 km22 s^2 + k11 k12 k22 km12 km22 s^2 + k11^2 km11 km12 km22 s^2 +
k11 k12 km12^2 km22 s^2 + k11 k21 km11 km21 km22 s^2 + k11 k22 km11 km21 km22 s^2 +
k11 km11^2 km21 km22 s^2 + k12 k21 km12 km21 km22 s^2 + k12 k22 km12 km21 km22 s^2 +
k11 km11 km12 km21 km22 s^2 + k12 km11 km12 km21 km22 s^2 + k12 km12^2 km21 km22 s^2 +
gammam1^2 k11 (k21 + k22 + km11 + km12) (k11 (k21 + k22) + (km11 + km12) km21)
  (k21 + k22 + km11 + km12 + s) + gamma1^2 k12 (k21 + k22 + km11 + km12)
  (k12 (k21 + k22) + (km11 + km12) km22) (k21 + k22 + km11 + km12 + s) +
```

```
gamma1 (k12 (k12 (k21 + k22 + km11 + km12 + s) (km11 (km11 + km12) km21 +
          k21 (km11 + 2 km12) km21 + k22 km11 (km21 + s) + k21 k22 (2 km21 + s) +
          k22^2 (2 km21 + s) + k22 km12 (2 km21 + s)) + (k21 + k22 + km11 + km12)
        km22 (k21 km11 km21 + k21 km12 (km21 + s) + (km11 + km12 + s)
           (km11 km21 + km12 (2 km21 + s)) + k22 (2 km11 km21 + km12 (2 km21 + s)))) +
    k11 (2 k12^2 (k21 + k22) (k21 + k22 + km11 + km12) (k21 + k22 + km11 + km12 + s) +
       (k21 + k22 + km11 + km12) km22 (k21 (km12 km22 + km11 (km22 + s)) +
          km11 (km11 (km22 + s) + km12 (km22 + s) + s (k22 + km22 + s))) +
       k12 (k21 + k22 + km11 + km12 + s) ((3 k22 km11 + km11^2 + 2 k22 km12 +
              3 km11 km12 + 2 km12^2) km22 + k21^2 (2 km22 + s) +
          k21 (3 km11 km22 + 2 km12 km22 + km11 s + km12 s + k22 (2 km22 + s))))) +
 gammam1 (gamma1 (k21 + k22 + km11 + km12) (2 k11 k12 (k21 + k22) +
       k12 (km11 + km12) km21 + k11 (km11 + km12) km22) (k21 + k22 + km11 + km12 + s) +
    k11^2 (k21 + k22 + km11 + km12 + s) (2 k12 (k21 + k22) (k21 + k22 + km11 + km12) +
       km12 (km11 + km12) km22 + k22 (2 km11 + km12) km22 + k21 km12 (km22 + s) +
       k21^2 (2 km22 + s) + k21 k22 (2 km22 + s) + k21 km11 (2 km22 + s)) +
    k12 (k21 + k22 + km11 + km12) km21 (k22 (km11 km21 + km12 (km21 + s)) +
       km12 (km11 (km21 + s) + km12 (km21 + s) + s (k21 + km21 + s))) +
    k11 (k12 (k21 + k22 + km11 + km12 + s) ((2 km11^2 + 3 km11 km12 + km12^2) km21 +
          k22^2 (2 km21 + s) + k21 (2 k22 km21 + 2 km11 km21 + 3 km12 km21 + k22 s) + k22
           (2 km11 km21 + 3 km12 km21 + km11 s + km12 s)) + (k21 + k22 + km11 + km12)
        km21 (k22 (km12 km22 + km11 (km22 + s)) + (km11 + km12 + s) (km12 km22 +
             km11 (2 km22 + s)) + k21 (2 km12 km22 + km11 (2 km22 + s)))))) /
((k11 k12 k21^2 + 2 k11 k12 k21 k22 + k11 k12 k22^2 + k11 k12 k21 km11 +
    k11 k12 k22 km11 + k11 k12 k21 km12 + k11 k12 k22 km12 +
    k12 k21 k22 km21 + k12 k22^2 km21 + k12 k21 km11 km21 + k12 km11^2 km21 +
    2 k12 k21 km12 km21 + k12 k22 km12 km21 + k12 km11 km12 km21 +
    gammam1 (k21 + k22 + km11 + km12) (k11 (k21 + k22) + (km11 + km12) km21) +
    k11 k21^2 km22 + k11 k21 k22 km22 + k11 k21 km11 km22 + 2 k11 k22 km11 km22 +
    k11 k22 km12 km22 + k11 km11 km12 km22 + k11 km12^2 km22 + k21 km11 km21 km22 +
    k22 km11 km21 km22 + km11^2 km21 km22 + k21 km12 km21 km22 +
    k22 km12 km21 km22 + 2 km11 km12 km21 km22 + km12^2 km21 km22 +
    gamma1 (k21 + k22 + km11 + km12) (k12 (k21 + k22) + (km11 + km12) km22))
  (k11 k12 k21^2 + 2 k11 k12 k21 k22 + k11 k12 k22^2 + k11 k12 k21 km11 +
    k11 k12 k22 km11 + k11 k12 k21 km12 + k11 k12 k22 km12 + k12 k21 k22 km21 +
    k12 k22^2 km21 + k12 k21 km11 km21 + k12 k22 km11 km21 + k12 km11^2 km21 +
    k12 k21 km12 km21 + k12 k22 km12 km21 + k12 km11 km12 km21 +
    k11 k21^2 km22 + k11 k21 k22 km22 + k11 k21 km11 km22 + k11 k22 km11 km22 +
    k11 k21 km12 km22 + k11 k22 km12 km22 + k11 km11 km12 km22 +
    k11 km12^2 km22 + k21 km11 km21 km22 + k22 km11 km21 km22 + km11^2 km21 km22 +
    k21 km12 km21 km22 + k22 km12 km21 km22 + 2 km11 km12 km21 km22 +
    km12^2 km21 km22 + 2 k11 k12 k21 s + k11 k21^2 s + k12 k21^2 s + 2 k11 k12 k22 s +
```

```
2 k11 k21 k22 s + 2 k12 k21 k22 s + k11 k22^2 s + k12 k22^2 s + k11 k12 km11 s +
k11 k21 km11 s + 2 k12 k21 km11 s + k11 k22 km11 s + 2 k12 k22 km11 s +
k12 km11^2 s + k11 k12 km12 s + 2 k11 k21 km12 s + k12 k21 km12 s +
2 k11 k22 km12 s + k12 k22 km12 s + k11 km11 km12 s + k12 km11 km12 s +
k11 km12^2 s + k12 k21 km21 s + 2 k12 k22 km21 s + k21 k22 km21 s +
k22^2 km21 s + 2 k12 km11 km21 s + k21 km11 km21 s + 2 k22 km11 km21 s +
km11^2 km21 s + k12 km12 km21 s + k21 km12 km21 s + 2 k22 km12 km21 s +
2 km11 km12 km21 s + km12^2 km21 s + 2 k11 k21 km22 s + k21^2 km22 s +
k11 k22 km22 s + k21 k22 km22 s + k11 km11 km22 s + 2 k21 km11 km22 s +
k22 km11 km22 s + km11^2 km22 s + 2 k11 km12 km22 s + 2 k21 km12 km22 s +
k22 km12 km22 s + 2 km11 km12 km22 s + km12^2 km22 s + k21 km21 km22 s +
k22 km21 km22 s + 2 km11 km21 km22 s + 2 km12 km21 km22 s + k11 k12 s^2 +
2 k11 k21 s^2 + 2 k12 k21 s^2 + k21^2 s^2 + 2 k11 k22 s^2 + 2 k12 k22 s^2 +
2 k21 k22 s^2 + k22^2 s^2 + k11 km11 s^2 + 2 k12 km11 s^2 + 2 k21 km11 s^2 +
2 k22 km11 s^2 + km11^2 s^2 + 2 k11 km12 s^2 + k12 km12 s^2 + 2 k21 km12 s^2 +
2 k22 km12 s^2 + 2 km11 km12 s^2 + km12^2 s^2 + k12 km21 s^2 + k21 km21 s^2 +
2 k22 km21 s^2 + 2 km11 km21 s^2 + 2 km12 km21 s^2 + k11 km22 s^2 + 2 k21 km22 s^2 +
k22 km22 s^2 + 2 km11 km22 s^2 + 2 km12 km22 s^2 + km21 km22 s^2 + k11 s^3 +
k12 s^3 + 2 k21 s^3 + 2 k22 s^3 + 2 km11 s^3 + 2 km12 s^3 + km21 s^3 + km22 s^3 +
s^4 + gammam1 (k21 + k22 + km11 + km12 + s) (km12 km21 + k21 s + k22 s +
    km12 s + km21 s + s^2 + k11 (k21 + k22 + s) + km11 (km21 + s)) +
gamma1 (k21 + k22 + km11 + km12 + s) (km12 km22 + k21 s + k22 s + km12 s +
    km22 s + s^2 + k12 (k21 + k22 + s) + km11 (km22 + s))))]
```

Out[38]=

```
Function[s,
 ((k21 + k22) (k11^2 k12^2 k21^3 + 3 k11^2 k12^2 k21^2 k22 + 3 k11^2 k12^2 k21 k22^2 + k11^2 k12^2 k22^3 +
      2 k11^2 k12^2 k21^2 km11 + 4 k11^2 k12^2 k21 k22 km11 + 2 k11^2 k12^2 k22^2 km11 +
      k11^2 k12^2 k21 km11^2 + k11^2 k12^2 k22 km11^2 + 2 k11^2 k12^2 k21^2 km12 +
      4 k11^2 k12^2 k21 k22 km12 + 2 k11^2 k12^2 k22^2 km12 + 2 k11^2 k12^2 k21 km11 km12 +
      2 k11^2 k12^2 k22 km11 km12 + k11^2 k12^2 k21 km12^2 + k11^2 k12^2 k22 km12^2 +
      2 k11 k12^2 k21^2 k22 km21 + 4 k11 k12^2 k21 k22^2 km21 + 2 k11 k12^2 k22^3 km21 +
      k11 k12^2 k21^2 km11 km21 + 4 k11 k12^2 k21 k22 km11 km21 + 3 k11 k12^2 k22^2 km11 km21 +
      2 k11 k12^2 k21 km11^2 km21 + 2 k11 k12^2 k22 km11^2 km21 + k11 k12^2 km11^3 km21 +
      2 k11 k12^2 k21^2 km12 km21 + 6 k11 k12^2 k21 k22 km12 km21 + 4 k11 k12^2 k22^2 km12 km21 +
      4 k11 k12^2 k21 km11 km12 km21 + 4 k11 k12^2 k22 km11 km12 km21 +
      2 k11 k12^2 km11^2 km12 km21 + 2 k11 k12^2 k21 km12^2 km21 + 2 k11 k12^2 k22 km12^2 km21 +
      k11 k12^2 km11 km12^2 km21 + k12^2 k21 k22^2 km21^2 + k12^2 k22^3 km21^2 +
      k12^2 k21 k22 km11 km21^2 + k12^2 k22^2 km11 km21^2 + k12^2 k22 km11^2 km21^2 +
      2 k12^2 k21 k22 km12 km21^2 + 2 k12^2 k22^2 km12 km21^2 + k12^2 k21 km11 km12 km21^2 +
      2 k12^2 k22 km11 km12 km21^2 + k12^2 km11^2 km12 km21^2 + k12^2 k21 km12^2 km21^2 +
      k12^2 k22 km12^2 km21^2 + k12^2 km11 km12^2 km21^2 + 2 k11^2 k12 k21^3 km22 +
      4 k11^2 k12 k21^2 k22 km22 + 2 k11^2 k12 k21 k22^2 km22 + 4 k11^2 k12 k21^2 km11 km22 +
      6 k11^2 k12 k21 k22 km11 km22 + 2 k11^2 k12 k22^2 km11 km22 +
```

$2 k11^{2} k12 k21 km11^{2} km22 + 2 k11^{2} k12 k22 km11^{2} km22 + 3 k11^{2} k12 k21^{2} km12 km22 +$
$4 k11^{2} k12 k21 k22 km12 km22 + k11^{2} k12 k22^{2} km12 km22 + 4 k11^{2} k12 k21 km11 km12 km22 +$
$4 k11^{2} k12 k22 km11 km12 km22 + k11^{2} k12 km11^{2} km12 km22 + 2 k11^{2} k12 k21 km12^{2} km22 +$
$2 k11^{2} k12 k22 km12^{2} km22 + 2 k11^{2} k12 km11 km12^{2} km22 + k11^{2} k12 km12^{3} km22 +$
$2 k11 k12 k21^{2} k22 km21 km22 + 2 k11 k12 k21 k22^{2} km21 km22 +$
$2 k11 k12 k21^{2} km11 km21 km22 + 5 k11 k12 k21 k22 km11 km21 km22 +$
$3 k11 k12 k22^{2} km11 km21 km22 + 4 k11 k12 k21 km11^{2} km21 km22 +$
$3 k11 k12 k22 km11^{2} km21 km22 + 2 k11 k12 km11^{3} km21 km22 +$
$3 k11 k12 k21^{2} km12 km21 km22 + 5 k11 k12 k21 k22 km12 km21 km22 +$
$2 k11 k12 k22^{2} km12 km21 km22 + 7 k11 k12 k21 km11 km12 km21 km22 +$
$7 k11 k12 k22 km11 km12 km21 km22 + 4 k11 k12 km11^{2} km12 km21 km22 +$
$3 k11 k12 k21 km12^{2} km21 km22 + 4 k11 k12 k22 km12^{2} km21 km22 +$
$4 k11 k12 km11 km12^{2} km21 km22 + 2 k11 k12 km12^{3} km21 km22 +$
$k12 k21 k22 km11 km21^{2} km22 + k12 k22^{2} km11 km21^{2} km22 + k12 k22 km11^{2} km21^{2} km22 +$
$k12 k21 k22 km12 km21^{2} km22 + k12 k22^{2} km12 km21^{2} km22 + k12 k21 km11 km12 km21^{2} km22 +$
$3 k12 k22 km11 km12 km21^{2} km22 + k12 km11^{2} km12 km21^{2} km22 +$
$k12 k21 km12^{2} km21^{2} km22 + 2 k12 k22 km12^{2} km21^{2} km22 + 2 k12 km11 km12^{2} km21^{2} km22 +$
$k12 km12^{3} km21^{2} km22 + k11^{2} k21^{3} km22^{2} + k11^{2} k21^{2} k22 km22^{2} +$
$2 k11^{2} k21^{2} km11 km22^{2} + 2 k11^{2} k21 k22 km11 km22^{2} + k11^{2} k21 km11^{2} km22^{2} +$
$k11^{2} k22 km11^{2} km22^{2} + k11^{2} k21^{2} km12 km22^{2} + k11^{2} k21 k22 km12 km22^{2} +$
$2 k11^{2} k21 km11 km12 km22^{2} + k11^{2} k22 km11 km12 km22^{2} + k11^{2} km11^{2} km12 km22^{2} +$
$k11^{2} k21 km12^{2} km22^{2} + k11^{2} km11 km12^{2} km22^{2} + k11 k21^{2} km11 km21 km22^{2} +$
$k11 k21 k22 km11 km21 km22^{2} + 2 k11 k21 km11^{2} km21 km22^{2} + k11 k22 km11^{2} km21 km22^{2} +$
$k11 km11^{3} km21 km22^{2} + k11 k21^{2} km12 km21 km22^{2} + k11 k21 k22 km12 km21 km22^{2} +$
$3 k11 k21 km11 km12 km21 km22^{2} + k11 k22 km11 km12 km21 km22^{2} +$
$2 k11 km11^{2} km12 km21 km22^{2} + k11 k21 km12^{2} km21 km22^{2} + k11 km11 km12^{2} km21 km22^{2} +$
$k11^{2} k12^{2} k21^{2} s + k11^{2} k12 k21^{3} s + 2 k11^{2} k12^{2} k21 k22 s + 2 k11^{2} k12 k21^{2} k22 s +$
$k11 k12^{2} k21^{2} k22 s + k11^{2} k12^{2} k22^{2} s + k11^{2} k12 k21 k22^{2} s + 2 k11 k12^{2} k21 k22^{2} s +$
$k11 k12^{2} k22^{3} s + k11^{2} k12^{2} k21 km11 s + 2 k11^{2} k12 k21^{2} km11 s + k11^{2} k12^{2} k22 km11 s +$
$2 k11^{2} k12 k21 k22 km11 s + 2 k11 k12^{2} k21 k22 km11 s + 2 k11 k12^{2} k22^{2} km11 s +$
$k11^{2} k12 k21 km11^{2} s + k11 k12^{2} k22 km11^{2} s + k11^{2} k12^{2} k21 km12 s +$
$2 k11^{2} k12 k21^{2} km12 s + k11^{2} k12^{2} k22 km12 s + 2 k11^{2} k12 k21 k22 km12 s +$
$2 k11 k12^{2} k21 k22 km12 s + 2 k11 k12^{2} k22^{2} km12 s + 2 k11^{2} k12 k21 km11 km12 s +$
$2 k11 k12^{2} k22 km11 km12 s + k11^{2} k12 k21 km12^{2} s + k11 k12^{2} k22 km12^{2} s +$
$2 k11 k12^{2} k21 k22 km21 s + k11 k12 k21^{2} k22 km21 s + 2 k11 k12^{2} k22^{2} km21 s +$
$k11 k12 k21 k22^{2} km21 s + k12^{2} k21 k22^{2} km21 s + k12^{2} k22^{3} km21 s +$
$k11 k12^{2} k21 km11 km21 s + k11 k12 k21^{2} km11 km21 s + k11 k12^{2} k22 km11 km21 s +$
$2 k11 k12 k21 k22 km11 km21 s + k12^{2} k22^{2} km11 km21 s + k11 k12^{2} km11^{2} km21 s +$
$2 k11 k12 k21 km11^{2} km21 s + k11 k12 k22 km11^{2} km21 s + k11 k12 km11^{3} km21 s +$
$2 k11 k12^{2} k21 km12 km21 s + k11 k12 k21^{2} km12 km21 s + k12^{2} k21^{2} km12 km21 s +$
$2 k11 k12^{2} k22 km12 km21 s + 2 k11 k12 k21 k22 km12 km21 s + 2 k12^{2} k21 k22 km12 km21 s +$
$2 k12^{2} k22^{2} km12 km21 s + k11 k12^{2} km11 km12 km21 s + 2 k11 k12 k21 km11 km12 km21 s +$
$2 k12^{2} k21 km11 km12 km21 s + 2 k12^{2} k22 km11 km12 km21 s + k11 k12 km11^{2} km12 km21 s +$
$k12^{2} km11^{2} km12 km21 s + k11 k12 k21 km12^{2} km21 s + k12^{2} k21 km12^{2} km21 s +$

$$k12^2 k22 km12^2 km21 s + k12^2 km11 km12^2 km21 s + k12^2 k22^2 km21^2 s +$$
$$k12^2 k21 km12 km21^2 s + k12^2 k22 km12 km21^2 s + k12^2 km11 km12 km21^2 s +$$
$$2 k11^2 k12 k21^2 km22 s + k11^2 k21^3 km22 s + 2 k11^2 k12 k21 k22 km22 s +$$
$$k11^2 k21^2 k22 km22 s + k11 k12 k21^2 k22 km22 s + k11 k12 k21 k22^2 km22 s +$$
$$2 k11^2 k12 k21 km11 km22 s + 2 k11^2 k21^2 km11 km22 s + 2 k11^2 k12 k22 km11 km22 s +$$
$$2 k11^2 k21 k22 km11 km22 s + 2 k11 k12 k21 k22 km11 km22 s + k11^2 k22^2 km11 km22 s +$$
$$k11 k12 k22^2 km11 km22 s + k11^2 k21 km11^2 km22 s + k11^2 k22 km11^2 km22 s +$$
$$k11 k12 k22 km11^2 km22 s + k11^2 k12 k21 km12 km22 s + k11^2 k21^2 km12 km22 s +$$
$$k11^2 k12 k22 km12 km22 s + 2 k11 k12 k21 k22 km12 km22 s + k11 k12 k22^2 km12 km22 s +$$
$$k11^2 k12 km11 km12 km22 s + 2 k11^2 k21 km11 km12 km22 s + 2 k11^2 k22 km11 km12 km22 s +$$
$$2 k11 k12 k22 km11 km12 km22 s + k11^2 km11^2 km12 km22 s + k11^2 k12 km12^2 km22 s +$$
$$k11 k12 k21 km12^2 km22 s + 2 k11 k12 k22 km12^2 km22 s + k11^2 km11 km12^2 km22 s +$$
$$k11 k12 km11 km12^2 km22 s + k11 k12 km12^3 km22 s + 2 k11 k12 k21 k22 km21 km22 s +$$
$$2 k11 k12 k21 km11 km21 km22 s + k11 k21^2 km11 km21 km22 s +$$
$$2 k11 k12 k22 km11 km21 km22 s + 2 k11 k21 k22 km11 km21 km22 s +$$
$$k11 k22^2 km11 km21 km22 s + 2 k11 k12 km11^2 km21 km22 s + 2 k11 k21 km11^2 km21 km22 s +$$
$$2 k11 k22 km11^2 km21 km22 s + k11 km11^3 km21 km22 s + 2 k11 k12 k21 km12 km21 km22 s +$$
$$k12 k21^2 km12 km21 km22 s + 2 k11 k12 k22 km12 km21 km22 s +$$
$$2 k12 k21 k22 km12 km21 km22 s + k12 k22^2 km12 km21 km22 s +$$
$$2 k11 k12 km11 km12 km21 km22 s + 2 k11 k21 km11 km12 km21 km22 s +$$
$$2 k12 k21 km11 km12 km21 km22 s + 2 k11 k22 km11 km12 km21 km22 s +$$
$$2 k12 k22 km11 km12 km21 km22 s + 2 k11 km11^2 km12 km21 km22 s +$$
$$k12 km11^2 km12 km21 km22 s + 2 k11 k12 km12^2 km21 km22 s + 2 k12 k21 km12^2 km21 km22 s +$$
$$2 k12 k22 km12^2 km21 km22 s + k11 km11 km12^2 km21 km22 s + 2 k12 km11 km12^2 km21 km22 s +$$
$$k12 km12^3 km21 km22 s + k12 k21 km12 km21^2 km22 s + k12 k22 km12 km21^2 km22 s +$$
$$k12 km11 km12 km21^2 km22 s + k12 km12^2 km21^2 km22 s + k11^2 k21^2 km22^2 s +$$
$$k11^2 k21 km11 km22^2 s + k11^2 k22 km11 km22^2 s + k11^2 km11 km12 km22^2 s +$$
$$k11 k21 km11 km21 km22^2 s + k11 k22 km11 km21 km22^2 s + k11 km11^2 km21 km22^2 s +$$
$$k11 km11 km12 km21 km22^2 s + k11^2 k12 k21^2 s^2 + k11^2 k12 k21 k22 s^2 +$$
$$k11 k12^2 k21 k22 s^2 + k11 k12^2 k22^2 s^2 + k11^2 k12 k21 km11 s^2 +$$
$$k11 k12^2 k22 km11 s^2 + k11^2 k12 k21 km12 s^2 + k11 k12^2 k22 km12 s^2 +$$
$$k11 k12 k21 k22 km21 s^2 + k12^2 k22^2 km21 s^2 + k11 k12 k21 km11 km21 s^2 +$$
$$k11 k12 km11^2 km21 s^2 + k11 k12 k21 km12 km21 s^2 + k12^2 k21 km12 km21 s^2 +$$
$$k12^2 k22 km12 km21 s^2 + k12^2 km11 km12 km21 s^2 + k11^2 k21^2 km22 s^2 +$$
$$k11 k12 k21 k22 km22 s^2 + k11^2 k21 km11 km22 s^2 + k11^2 k22 km11 km22 s^2 +$$
$$k11 k12 k22 km11 km22 s^2 + k11 k12 k22 km12 km22 s^2 + k11^2 km11 km12 km22 s^2 +$$
$$k11 k12 km12^2 km22 s^2 + k11 k21 km11 km21 km22 s^2 + k11 k22 km11 km21 km22 s^2 +$$
$$k11 km11^2 km21 km22 s^2 + k12 k21 km12 km21 km22 s^2 + k12 k22 km12 km21 km22 s^2 +$$
$$k11 km11 km12 km21 km22 s^2 + k12 km11 km12 km21 km22 s^2 + k12 km12^2 km21 km22 s^2 +$$
$$gammam1^2 k11 (k21 + k22 + km11 + km12) (k11 (k21 + k22) + (km11 + km12) km21)$$
$$(k21 + k22 + km11 + km12 + s) + gamma1^2 k12 (k21 + k22 + km11 + km12)$$
$$(k12 (k21 + k22) + (km11 + km12) km22) (k21 + k22 + km11 + km12 + s) +$$
$$gamma1 (k12 (k12 (k21 + k22 + km11 + km12 + s) (km11 (km11 + km12) km21 + k21$$

Printed by Wolfram Mathematica Student Edition

```
(km11 + 2 km12) km21 + k22 km11 (km21 + s) + k21 k22 (2 km21 + s) + k22^2
(2 km21 + s) + k22 km12 (2 km21 + s)) + (k21 + k22 + km11 + km12)
km22 (k21 km11 km21 + k21 km12 (km21 + s) + (km11 + km12 + s)
(km11 km21 + km12 (2 km21 + s)) + k22 (2 km11 km21 + km12 (2 km21 + s)))) +
k11 (2 k12^2 (k21 + k22) (k21 + k22 + km11 + km12) (k21 + k22 + km11 + km12 + s) +
(k21 + k22 + km11 + km12) km22 (k21 (km12 km22 + km11 (km22 + s)) + km11
(km11 (km22 + s) + km12 (km22 + s) + s (k22 + km22 + s))) +
k12 (k21 + k22 + km11 + km12 + s) ((3 k22 km11 + km11^2 + 2 k22 km12 +
3 km11 km12 + 2 km12^2) km22 + k21^2 (2 km22 + s) + k21
(3 km11 km22 + 2 km12 km22 + km11 s + km12 s + k22 (2 km22 + s))))) +
gammam1 (gamma1 (k21 + k22 + km11 + km12) (2 k11 k12 (k21 + k22) +
k12 (km11 + km12) km21 + k11 (km11 + km12) km22) (k21 + k22 + km11 + km12 + s) +
k11^2 (k21 + k22 + km11 + km12 + s) (2 k12 (k21 + k22) (k21 + k22 + km11 + km12) +
km12 (km11 + km12) km22 + k22 (2 km11 + km12) km22 + k21 km12 (km22 + s) +
k21^2 (2 km22 + s) + k21 k22 (2 km22 + s) + k21 km11 (2 km22 + s)) +
k12 (k21 + k22 + km11 + km12) km21 (k22 (km11 km21 + km12 (km21 + s)) +
km12 (km11 (km21 + s) + km12 (km21 + s) + s (k21 + km21 + s))) +
k11 (k12 (k21 + k22 + km11 + km12 + s) ((2 km11^2 + 3 km11 km12 + km12^2) km21 +
k22^2 (2 km21 + s) + k21 (2 k22 km21 + 2 km11 km21 + 3 km12 km21 + k22 s) + k22
(2 km11 km21 + 3 km12 km21 + km11 s + km12 s)) + (k21 + k22 + km11 + km12)
km21 (k22 (km12 km22 + km11 (km22 + s)) + (km11 + km12 + s) (km12 km22 +
km11 (2 km22 + s)) + k21 (2 km12 km22 + km11 (2 km22 + s)))))) /
((k11 k12 k21^2 + 2 k11 k12 k21 k22 + k11 k12 k22^2 + k11 k12 k21 km11 +
k11 k12 k22 km11 + k11 k12 k21 km12 + k11 k12 k22 km12 +
k12 k21 k22 km21 + k12 k22^2 km21 + k12 k21 km11 km21 + k12 km11^2 km21 +
2 k12 k21 km12 km21 + k12 k22 km12 km21 + k12 km11 km12 km21 +
gammam1 (k21 + k22 + km11 + km12) (k11 (k21 + k22) + (km11 + km12) km21) +
k11 k21^2 km22 + k11 k21 k22 km22 + k11 k21 km11 km22 + 2 k11 k22 km11 km22 +
k11 k22 km12 km22 + k11 km11 km12 km22 + k11 km12^2 km22 + k21 km11 km21 km22 +
k22 km11 km21 km22 + km11^2 km21 km22 + k21 km12 km21 km22 +
k22 km12 km21 km22 + 2 km11 km12 km21 km22 + km12^2 km21 km22 +
gamma1 (k21 + k22 + km11 + km12) (k12 (k21 + k22) + (km11 + km12) km22))
(k11 k12 k21^2 + 2 k11 k12 k21 k22 + k11 k12 k22^2 + k11 k12 k21 km11 +
k11 k12 k22 km11 + k11 k12 k21 km12 + k11 k12 k22 km12 + k12 k21 k22 km21 +
k12 k22^2 km21 + k12 k21 km11 km21 + k12 k22 km11 km21 + k12 km11^2 km21 +
k12 k21 km12 km21 + k12 k22 km12 km21 + k12 km11 km12 km21 +
k11 k21^2 km22 + k11 k21 k22 km22 + k11 k21 km11 km22 + k11 k22 km11 km22 +
k11 k21 km12 km22 + k11 k22 km12 km22 + k11 km11 km12 km22 +
k11 km12^2 km22 + k21 km11 km21 km22 + k22 km11 km21 km22 + km11^2 km21 km22 +
k21 km12 km21 km22 + k22 km12 km21 km22 + 2 km11 km12 km21 km22 +
km12^2 km21 km22 + 2 k11 k12 k21 s + k11 k21^2 s + k12 k21^2 s + 2 k11 k12 k22 s +
2 k11 k21 k22 s + 2 k12 k21 k22 s + k11 k22^2 s + k12 k22^2 s + k11 k12 km11 s +
```

```
k11 k21 km11 s + 2 k12 k21 km11 s + k11 k22 km11 s + 2 k12 k22 km11 s +
k12 km11^2 s + k11 k12 km12 s + 2 k11 k21 km12 s + k12 k21 km12 s +
2 k11 k22 km12 s + k12 k22 km12 s + k11 km11 km12 s + k12 km11 km12 s +
k11 km12^2 s + k12 k21 km21 s + 2 k12 k22 km21 s + k21 k22 km21 s +
k22^2 km21 s + 2 k12 km11 km21 s + k21 km11 km21 s + 2 k22 km11 km21 s +
km11^2 km21 s + k12 km12 km21 s + k21 km12 km21 s + 2 k22 km12 km21 s +
2 km11 km12 km21 s + km12^2 km21 s + 2 k11 k21 km22 s + k21^2 km22 s +
k11 k22 km22 s + k21 k22 km22 s + k11 km11 km22 s + 2 k21 km11 km22 s +
k22 km11 km22 s + km11^2 km22 s + 2 k11 km12 km22 s + 2 k21 km12 km22 s +
k22 km12 km22 s + 2 km11 km12 km22 s + km12^2 km22 s + k21 km21 km22 s +
k22 km21 km22 s + 2 km11 km21 km22 s + 2 km12 km21 km22 s + k11 k12 s^2 +
2 k11 k21 s^2 + 2 k12 k21 s^2 + k21^2 s^2 + 2 k11 k22 s^2 + 2 k12 k22 s^2 +
2 k21 k22 s^2 + k22^2 s^2 + k11 km11 s^2 + 2 k12 km11 s^2 + 2 k21 km11 s^2 +
2 k22 km11 s^2 + km11^2 s^2 + 2 k11 km12 s^2 + k12 km12 s^2 + 2 k21 km12 s^2 +
2 k22 km12 s^2 + 2 km11 km12 s^2 + km12^2 s^2 + k12 km21 s^2 + k21 km21 s^2 +
2 k22 km21 s^2 + 2 km11 km21 s^2 + 2 km12 km21 s^2 + k11 km22 s^2 +
2 k21 km22 s^2 + k22 km22 s^2 + 2 km11 km22 s^2 + 2 km12 km22 s^2 +
km21 km22 s^2 + k11 s^3 + k12 s^3 + 2 k21 s^3 + 2 k22 s^3 + 2 km11 s^3 +
2 km12 s^3 + km21 s^3 + km22 s^3 + s^4 + gammam1 (k21 + k22 + km11 + km12 + s)
  (km12 km21 + k21 s + k22 s + km12 s + km21 s + s^2 + k11 (k21 + k22 + s) + km11 (km21 + s)) +
gamma1 (k21 + k22 + km11 + km12 + s) (km12 km22 + k21 s + k22 s +
    km12 s + km22 s + s^2 + k12 (k21 + k22 + s) + km11 (km22 + s)))))]
```

In[39]:=

```
Pminusfunc =
  Function[s, (Omegaminus[s].Pbarev0)[[1, 1]] + (Omegaminus[s].Pbarev0)[[2, 1]]]
```

Out[39]=

```
Function[s, (Omegaminus[s].Pbarev0)[[1, 1]] + (Omegaminus[s].Pbarev0)[[2, 1]]]
```

In[40]:=

```
Simplify[Together[Pminusfunc[s]]]
```

Out[40]=

```
((km11 + km12) (k11 k12^2 k21^3 km21 + 2 k11 k12^2 k21^2 k22 km21 +
    k11 k12^2 k21 k22^2 km21 + 2 k11 k12^2 k21^2 km11 km21 + 3 k11 k12^2 k21 k22 km11 km21 +
    k11 k12^2 k22^2 km11 km21 + k11 k12^2 k21 km11^2 km21 + k11 k12^2 k22 km11^2 km21 +
    k11 k12^2 k21^2 km12 km21 + k11 k12^2 k21 k22 km12 km21 + k11 k12^2 k21 km11 km12 km21 +
    k11 k12^2 k22 km11 km12 km21 + k12^2 k21^2 k22 km21^2 + k12^2 k21 k22^2 km21^2 +
    k12^2 k21^2 km11 km21^2 + 2 k12^2 k21 k22 km11 km21^2 + k12^2 k22^2 km11 km21^2 +
    2 k12^2 k21 km11^2 km21^2 + k12^2 k22 km11^2 km21^2 + k12^2 km11^3 km21^2 + k12^2 k21^2 km12 km21^2 +
    k12^2 k21 k22 km12 km21^2 + 2 k12^2 k21 km11 km12 km21^2 + k12^2 k22 km11 km12 km21^2 +
    k12^2 km11^2 km12 km21^2 + k11^2 k12 k21^2 k22 km22 + 2 k11^2 k12 k21 k22^2 km22 +
    k11^2 k12 k22^3 km22 + k11^2 k12 k21 k22 km11 km22 + k11^2 k12 k22^2 km11 km22 +
    k11^2 k12 k21^2 km12 km22 + 3 k11^2 k12 k21 k22 km12 km22 + 2 k11^2 k12 k22^2 km12 km22 +
    k11^2 k12 k21 km11 km12 km22 + k11^2 k12 k22 km11 km12 km22 + k11^2 k12 k21 km12^2 km22 +
    k11^2 k12 k22 km12^2 km22 + 2 k11 k12 k21^3 km21 km22 + 4 k11 k12 k21^2 k22 km21 km22 +
    4 k11 k12 k21 k22^2 km21 km22 + 2 k11 k12 k22^3 km21 km22 + 4 k11 k12 k21^2 km11 km21 km22 +
```

7 k11 k12 k21 k22 km11 km21 km22 + 3 k11 k12 $k22^2$ km11 km21 km22 +
2 k11 k12 k21 $km11^2$ km21 km22 + 3 k11 k12 k22 $km11^2$ km21 km22 +
3 k11 k12 $k21^2$ km12 km21 km22 + 7 k11 k12 k21 k22 km12 km21 km22 +
4 k11 k12 $k22^2$ km12 km21 km22 + 5 k11 k12 k21 km11 km12 km21 km22 +
5 k11 k12 k22 km11 km12 km21 km22 + 2 k11 k12 $km11^2$ km12 km21 km22 +
3 k11 k12 k21 $km12^2$ km21 km22 + 2 k11 k12 k22 $km12^2$ km21 km22 +
2 k11 k12 km11 $km12^2$ km21 km22 + k12 $k21^2$ k22 $km21^2$ km22 + 2 k12 k21 $k22^2$ $km21^2$ km22 +
k12 $k22^3$ $km21^2$ km22 + 2 k12 $k21^2$ km11 $km21^2$ km22 + 4 k12 k21 k22 km11 $km21^2$ km22 +
2 k12 $k22^2$ km11 $km21^2$ km22 + 4 k12 k21 $km11^2$ $km21^2$ km22 + 3 k12 k22 $km11^2$ $km21^2$ km22 +
2 k12 $km11^3$ $km21^2$ km22 + 2 k12 $k21^2$ km12 $km21^2$ km22 + 4 k12 k21 k22 km12 $km21^2$ km22 +
2 k12 $k22^2$ km12 $km21^2$ km22 + 6 k12 k21 km11 km12 $km21^2$ km22 +
4 k12 k22 km11 km12 $km21^2$ km22 + 4 k12 $km11^2$ km12 $km21^2$ km22 +
2 k12 k21 $km12^2$ $km21^2$ km22 + k12 k22 $km12^2$ $km21^2$ km22 + 2 k12 km11 $km12^2$ $km21^2$ km22 +
$k11^2$ $k21^2$ k22 $km22^2$ + $k11^2$ k21 $k22^2$ $km22^2$ + $k11^2$ k21 k22 km11 $km22^2$ +
$k11^2$ $k22^2$ km11 $km22^2$ + $k11^2$ $k21^2$ km12 $km22^2$ + 2 $k11^2$ k21 k22 km12 $km22^2$ +
$k11^2$ $k22^2$ km12 $km22^2$ + $k11^2$ k21 km11 km12 $km22^2$ + 2 $k11^2$ k22 km11 km12 $km22^2$ +
$k11^2$ k21 $km12^2$ $km22^2$ + 2 $k11^2$ k22 $km12^2$ $km22^2$ + $k11^2$ km11 $km12^2$ $km22^2$ +
$k11^2$ $km12^3$ $km22^2$ + k11 $k21^3$ km21 $km22^2$ + 2 k11 $k21^2$ k22 km21 $km22^2$ +
k11 k21 $k22^2$ km21 $km22^2$ + 2 k11 $k21^2$ km11 km21 $km22^2$ + 4 k11 k21 k22 km11 km21 $km22^2$ +
2 k11 $k22^2$ km11 km21 $km22^2$ + k11 k21 $km11^2$ km21 $km22^2$ + 2 k11 k22 $km11^2$ km21 $km22^2$ +
2 k11 $k21^2$ km12 km21 $km22^2$ + 4 k11 k21 k22 km12 km21 $km22^2$ + 2 k11 $k22^2$ km12 km21 $km22^2$ +
4 k11 k21 km11 km12 km21 $km22^2$ + 6 k11 k22 km11 km12 km21 $km22^2$ +
2 k11 $km11^2$ km12 km21 $km22^2$ + 3 k11 k21 $km12^2$ km21 $km22^2$ + 4 k11 k22 $km12^2$ km21 $km22^2$ +
4 k11 km11 $km12^2$ km21 $km22^2$ + 2 k11 $km12^3$ km21 $km22^2$ + $k21^2$ km11 $km21^2$ $km22^2$ +
2 k21 k22 km11 $km21^2$ $km22^2$ + $k22^2$ km11 $km21^2$ $km22^2$ + 2 k21 $km11^2$ $km21^2$ $km22^2$ +
2 k22 $km11^2$ $km21^2$ $km22^2$ + $km11^3$ $km21^2$ $km22^2$ + $k21^2$ km12 $km21^2$ $km22^2$ +
2 k21 k22 km12 $km21^2$ $km22^2$ + $k22^2$ km12 $km21^2$ $km22^2$ + 4 k21 km11 km12 $km21^2$ $km22^2$ +
4 k22 km11 km12 $km21^2$ $km22^2$ + 3 $km11^2$ km12 $km21^2$ $km22^2$ + 2 k21 $km12^2$ $km21^2$ $km22^2$ +
2 k22 $km12^2$ $km21^2$ $km22^2$ + 3 km11 $km12^2$ $km21^2$ $km22^2$ + $km12^3$ $km21^2$ $km22^2$ +
k11 $k12^2$ $k21^2$ km21 s + k11 k12 $k21^3$ km21 s + k11 $k12^2$ k21 k22 km21 s +
2 k11 k12 $k21^2$ k22 km21 s + k11 k12 k21 $k22^2$ km21 s + k11 $k12^2$ k21 km11 km21 s +
2 k11 k12 $k21^2$ km11 km21 s + 2 k11 k12 k21 k22 km11 km21 s + k11 k12 k21 $km11^2$ km21 s +
k11 $k12^2$ k21 km12 km21 s + 2 k11 k12 $k21^2$ km12 km21 s + 2 k11 k12 k21 k22 km12 km21 s +
2 k11 k12 k21 km11 km12 km21 s + k11 k12 k21 $km12^2$ km21 s + $k12^2$ k21 k22 $km21^2$ s +
k12 $k21^2$ k22 $km21^2$ s + k12 k21 $k22^2$ $km21^2$ s + $k12^2$ k21 km11 $km21^2$ s +
k12 $k21^2$ km11 $km21^2$ s + 2 k12 k21 k22 km11 $km21^2$ s + $k12^2$ $km11^2$ $km21^2$ s +
2 k12 k21 $km11^2$ $km21^2$ s + k12 k22 $km11^2$ $km21^2$ s + k12 $km11^3$ $km21^2$ s +
$k12^2$ k21 km12 $km21^2$ s + k12 $k21^2$ km12 $km21^2$ s + 2 k12 k21 k22 km12 $km21^2$ s +
2 k12 k21 km11 km12 $km21^2$ s + k12 $km11^2$ km12 $km21^2$ s + k12 k21 $km12^2$ $km21^2$ s +
$k11^2$ k12 k21 k22 km22 s + k11 k12 $k21^2$ k22 km22 s + $k11^2$ k12 $k22^2$ km22 s +
2 k11 k12 k21 $k22^2$ km22 s + k11 k12 $k22^3$ km22 s + $k11^2$ k12 k22 km11 km22 s +
2 k11 k12 k21 k22 km11 km22 s + 2 k11 k12 $k22^2$ km11 km22 s + k11 k12 k22 $km11^2$ km22 s +
$k11^2$ k12 k22 km12 km22 s + 2 k11 k12 k21 k22 km12 km22 s + 2 k11 k12 $k22^2$ km12 km22 s +
2 k11 k12 k22 km11 km12 km22 s + k11 k12 k22 $km12^2$ km22 s + 2 k11 k12 $k21^2$ km21 km22 s +

$k11\ k21^3\ km21\ km22\ s + 2\ k11\ k12\ k21\ k22\ km21\ km22\ s + k11\ k21^2\ k22\ km21\ km22\ s +$
$2\ k11\ k12\ k22^2\ km21\ km22\ s + k12\ k21\ k22^2\ km21\ km22\ s + k12\ k22^3\ km21\ km22\ s +$
$2\ k11\ k12\ k21\ km11\ km21\ km22\ s + 2\ k11\ k21^2\ km11\ km21\ km22\ s +$
$2\ k11\ k12\ k22\ km11\ km21\ km22\ s + 2\ k11\ k21\ k22\ km11\ km21\ km22\ s +$
$k11\ k22^2\ km11\ km21\ km22\ s + k12\ k22^2\ km11\ km21\ km22\ s + k11\ k21\ km11^2\ km21\ km22\ s +$
$k11\ k22\ km11^2\ km21\ km22\ s + 2\ k11\ k12\ k21\ km12\ km21\ km22\ s +$
$k11\ k21^2\ km12\ km21\ km22\ s + k12\ k21^2\ km12\ km21\ km22\ s + 2\ k11\ k12\ k22\ km12\ km21\ km22\ s +$
$2\ k12\ k21\ k22\ km12\ km21\ km22\ s + 2\ k12\ k22^2\ km12\ km21\ km22\ s +$
$2\ k11\ k12\ km11\ km12\ km21\ km22\ s + 2\ k11\ k21\ km11\ km12\ km21\ km22\ s +$
$2\ k12\ k21\ km11\ km12\ km21\ km22\ s + 2\ k11\ k22\ km11\ km12\ km21\ km22\ s +$
$2\ k12\ k22\ km11\ km12\ km21\ km22\ s + k11\ km11^2\ km12\ km21\ km22\ s +$
$k12\ km11^2\ km12\ km21\ km22\ s + k12\ k21\ km12^2\ km21\ km22\ s + k12\ k22\ km12^2\ km21\ km22\ s +$
$k11\ km11\ km12^2\ km21\ km22\ s + k12\ km11\ km12^2\ km21\ km22\ s + k12\ k21\ k22\ km21^2\ km22\ s +$
$k12\ k22^2\ km21^2\ km22\ s + 2\ k12\ k21\ km11\ km21^2\ km22\ s + k21^2\ km11\ km21^2\ km22\ s +$
$k12\ k22\ km11\ km21^2\ km22\ s + 2\ k21\ k22\ km11\ km21^2\ km22\ s + k22^2\ km11\ km21^2\ km22\ s +$
$2\ k12\ km11^2\ km21^2\ km22\ s + 2\ k21\ km11^2\ km21^2\ km22\ s + 2\ k22\ km11^2\ km21^2\ km22\ s +$
$km11^3\ km21^2\ km22\ s + 2\ k12\ k21\ km12\ km21^2\ km22\ s + k12\ k22\ km12\ km21^2\ km22\ s +$
$2\ k12\ km11\ km12\ km21^2\ km22\ s + 2\ k21\ km11\ km12\ km21^2\ km22\ s +$
$2\ k22\ km11\ km12\ km21^2\ km22\ s + 2\ km11^2\ km12\ km21^2\ km22\ s + km11\ km12^2\ km21^2\ km22\ s +$
$k11^2\ k21\ k22\ km22^2\ s + k11\ k21^2\ k22\ km22^2\ s + k11\ k21\ k22^2\ km22^2\ s +$
$k11^2\ k22\ km11\ km22^2\ s + 2\ k11\ k21\ k22\ km11\ km22^2\ s + k11\ k22^2\ km11\ km22^2\ s +$
$k11\ k22\ km11^2\ km22^2\ s + k11^2\ k22\ km12\ km22^2\ s + 2\ k11\ k21\ k22\ km12\ km22^2\ s +$
$k11\ k22^2\ km12\ km22^2\ s + 2\ k11\ k22\ km11\ km12\ km22^2\ s + k11^2\ km12^2\ km22^2\ s +$
$k11\ k21\ km12^2\ km22^2\ s + 2\ k11\ k22\ km12^2\ km22^2\ s + k11\ km11\ km12^2\ km22^2\ s +$
$k11\ km12^3\ km22^2\ s + k11\ k21^2\ km21\ km22^2\ s + k11\ k21\ k22\ km21\ km22^2\ s +$
$k11\ k21\ km11\ km21\ km22^2\ s + 2\ k11\ k22\ km11\ km21\ km22^2\ s + k11\ k21\ km12\ km21\ km22^2\ s +$
$k21^2\ km12\ km21\ km22^2\ s + 2\ k11\ k22\ km12\ km21\ km22^2\ s + 2\ k21\ k22\ km12\ km21\ km22^2\ s +$
$k22^2\ km12\ km21\ km22^2\ s + 2\ k11\ km11\ km12\ km21\ km22^2\ s + 2\ k21\ km11\ km12\ km21\ km22^2\ s +$
$2\ k22\ km11\ km12\ km21\ km22^2\ s + km11^2\ km12\ km21\ km22^2\ s + 2\ k11\ km12^2\ km21\ km22^2\ s +$
$2\ k21\ km12^2\ km21\ km22^2\ s + 2\ k22\ km12^2\ km21\ km22^2\ s + 2\ km11\ km12^2\ km21\ km22^2\ s +$
$km12^3\ km21\ km22^2\ s + k21\ km11\ km21^2\ km22^2\ s + k22\ km11\ km21^2\ km22^2\ s +$
$km11^2\ km21^2\ km22^2\ s + k21\ km12\ km21^2\ km22^2\ s + k22\ km12\ km21^2\ km22^2\ s +$
$2\ km11\ km12\ km21^2\ km22^2\ s + km12^2\ km21^2\ km22^2\ s + k11\ k12\ k21^2\ km21\ s^2 +$
$k11\ k12\ k21\ k22\ km21\ s^2 + k11\ k12\ k21\ km11\ km21\ s^2 + k11\ k12\ k21\ km12\ km21\ s^2 +$
$k12\ k21\ k22\ km21^2\ s^2 + k12\ k21\ km11\ km21^2\ s^2 + k12\ km11^2\ km21^2\ s^2 + k12\ k21\ km12\ km21^2\ s^2 +$
$k11\ k12\ k21\ k22\ km22\ s^2 + k11\ k12\ k22^2\ km22\ s^2 + k11\ k12\ k22\ km11\ km22\ s^2 +$
$k11\ k12\ k22\ km12\ km22\ s^2 + k11\ k21^2\ km21\ km22\ s^2 + k12\ k22^2\ km21\ km22\ s^2 +$
$k11\ k21\ km11\ km21\ km22\ s^2 + k11\ k22\ km11\ km21\ km22\ s^2 + k12\ k21\ km12\ km21\ km22\ s^2 +$
$k12\ k22\ km12\ km21\ km22\ s^2 + k11\ km11\ km12\ km21\ km22\ s^2 + k12\ km11\ km12\ km21\ km22\ s^2 +$
$k21\ km11\ km21^2\ km22\ s^2 + k22\ km11\ km21^2\ km22\ s^2 + km11^2\ km21^2\ km22\ s^2 +$
$km11\ km12\ km21^2\ km22\ s^2 + k11\ k21\ k22\ km22^2\ s^2 + k11\ k22\ km11\ km22^2\ s^2 +$
$k11\ k22\ km12\ km22^2\ s^2 + k11\ km12^2\ km22^2\ s^2 + k21\ km12\ km21\ km22^2\ s^2 +$
$k22\ km12\ km21\ km22^2\ s^2 + km11\ km12\ km21\ km22^2\ s^2 + km12^2\ km21\ km22^2\ s^2 +$
$gammam1^2\ (k21 + k22 + km11 + km12)\ km21\ (k11\ (k21 + k22) + (km11 + km12)\ km21)$

$(k21 + k22 + km11 + km12 + s) + gamma1^{2} (k21 + k22 + km11 + km12) km22$
$(k12 (k21 + k22) + (km11 + km12) km22) (k21 + k22 + km11 + km12 + s) +$
$gammam1 (gamma1 (k21 + k22 + km11 + km12) (k12 (k21 + k22) km21 +$
$k11 (k21 + k22) km22 + 2 (km11 + km12) km21 km22) (k21 + k22 + km11 + km12 + s) +$
$k11^{2} (k21 + k22 + km11 + km12) km22 (k21 (k22 + km12) + k22 (k22 + km12 + s)) + km21$
$(k21 + k22 + km11 + km12 + s) (k12 (k22^{2} + k22 (km11 + km12) + 2 km11 (km11 + km12) +$
$k21 (k22 + 2 (km11 + km12))) km21 + (k21 + k22 + km11 + km12) (km12 km22$
$(2 km21 + s) + km11 km21 (2 km22 + s))) + k11 (k12 (k21 + k22 + km11 + km12)$
$km21 (2 k21^{2} + k22 (k22 + 2 km11 + km12 + s) + k21 (3 k22 + 2 km11 + km12 + 2 s)) +$
$(k21 + k22 + km11 + km12 + s) (2 km12 (km11 + km12) km21 km22 + k22^{2} km22$
$(km21 + s) + k22 (km11 + km12) km22 (3 km21 + s) + k21^{2} km21 (2 km22 + s) +$
$k21 (km11 + km12) km21 (2 km22 + s) + k21 k22 (km22 s + km21 (3 km22 + s))))) +$
$gamma1 (k12^{2} (k21 + k22 + km11 + km12) km21 (k21^{2} + k22 km11 + k21 (k22 + km11 + s)) +$
$km22 (k21 + k22 + km11 + km12 + s)$
$(k11 (k21^{2} + 2 (k22 + km12) (km11 + km12) + k21 (k22 + km11 + km12)) km22 +$
$(k21 + k22 + km11 + km12) (km12 km22 (2 km21 + s) + km11 km21 (2 km22 + s))) +$
$k12 (k11 (k21 + k22 + km11 + km12) km22 (k21^{2} + k21 (3 k22 + km11 + 2 km12 + s) +$
$k22 (2 k22 + km11 + 2 (km12 + s))) + (k21 + k22 + km11 + km12 + s)$
$(2 km11 (km11 + km12) km21 km22 + k22^{2} km22 (2 km21 + s) +$
$k22 (km11 + km12) km22 (2 km21 + s) + k21^{2} km21 (km22 + s) + k21 (km11 + km12)$
$km21 (3 km22 + s) + k21 k22 (km22 s + km21 (3 km22 + s)))))) /$
$((k11 k12 k21^{2} + 2 k11 k12 k21 k22 + k11 k12 k22^{2} + k11 k12 k21 km11 + k11 k12 k22 km11 +$
$k11 k12 k21 km12 + k11 k12 k22 km12 + k12 k21 k22 km21 +$
$k12 k22^{2} km21 + k12 k21 km11 km21 + k12 km11^{2} km21 +$
$2 k12 k21 km12 km21 + k12 k22 km12 km21 + k12 km11 km12 km21 +$
$gammam1 (k21 + k22 + km11 + km12) (k11 (k21 + k22) + (km11 + km12) km21) +$
$k11 k21^{2} km22 + k11 k21 k22 km22 + k11 k21 km11 km22 + 2 k11 k22 km11 km22 +$
$k11 k22 km12 km22 + k11 km11 km12 km22 + k11 km12^{2} km22 + k21 km11 km21 km22 +$
$k22 km11 km21 km22 + km11^{2} km21 km22 + k21 km12 km21 km22 +$
$k22 km12 km21 km22 + 2 km11 km12 km21 km22 + km12^{2} km21 km22 +$
$gamma1 (k21 + k22 + km11 + km12) (k12 (k21 + k22) + (km11 + km12) km22))$
$(k11 k12 k21^{2} + 2 k11 k12 k21 k22 + k11 k12 k22^{2} + k11 k12 k21 km11 +$
$k11 k12 k22 km11 + k11 k12 k21 km12 + k11 k12 k22 km12 + k12 k21 k22 km21 +$
$k12 k22^{2} km21 + k12 k21 km11 km21 + k12 k22 km11 km21 + k12 km11^{2} km21 +$
$k12 k21 km12 km21 + k12 k22 km12 km21 + k12 km11 km12 km21 +$
$k11 k21^{2} km22 + k11 k21 k22 km22 + k11 k21 km11 km22 + k11 k22 km11 km22 +$
$k11 k21 km12 km22 + k11 k22 km12 km22 + k11 km11 km12 km22 +$
$k11 km12^{2} km22 + k21 km11 km21 km22 + k22 km11 km21 km22 + km11^{2} km21 km22 +$
$k21 km12 km21 km22 + k22 km12 km21 km22 + 2 km11 km12 km21 km22 +$
$km12^{2} km21 km22 + 2 k11 k12 k21 s + k11 k21^{2} s + k12 k21^{2} s + 2 k11 k12 k22 s +$
$2 k11 k21 k22 s + 2 k12 k21 k22 s + k11 k22^{2} s + k12 k22^{2} s + k11 k12 km11 s +$
$k11 k21 km11 s + 2 k12 k21 km11 s + k11 k22 km11 s + 2 k12 k22 km11 s +$

```
k12 km11^2 s + k11 k12 km12 s + 2 k11 k21 km12 s + k12 k21 km12 s +
2 k11 k22 km12 s + k12 k22 km12 s + k11 km11 km12 s + k12 km11 km12 s +
k11 km12^2 s + k12 k21 km21 s + 2 k12 k22 km21 s + k21 k22 km21 s + k22^2 km21 s +
2 k12 km11 km21 s + k21 km11 km21 s + 2 k22 km11 km21 s + km11^2 km21 s +
k12 km12 km21 s + k21 km12 km21 s + 2 k22 km12 km21 s + 2 km11 km12 km21 s +
km12^2 km21 s + 2 k11 k21 km22 s + k21^2 km22 s + k11 k22 km22 s +
k21 k22 km22 s + k11 km11 km22 s + 2 k21 km11 km22 s + k22 km11 km22 s +
km11^2 km22 s + 2 k11 km12 km22 s + 2 k21 km12 km22 s + k22 km12 km22 s +
2 km11 km12 km22 s + km12^2 km22 s + k21 km21 km22 s + k22 km21 km22 s +
2 km11 km21 km22 s + 2 km12 km21 km22 s + k11 k12 s^2 + 2 k11 k21 s^2 +
2 k12 k21 s^2 + k21^2 s^2 + 2 k11 k22 s^2 + 2 k12 k22 s^2 + 2 k21 k22 s^2 + k22^2 s^2 +
k11 km11 s^2 + 2 k12 km11 s^2 + 2 k21 km11 s^2 + 2 k22 km11 s^2 + km11^2 s^2 +
2 k11 km12 s^2 + k12 km12 s^2 + 2 k21 km12 s^2 + 2 k22 km12 s^2 + 2 km11 km12 s^2 +
km12^2 s^2 + k12 km21 s^2 + k21 km21 s^2 + 2 k22 km21 s^2 + 2 km11 km21 s^2 +
2 km12 km21 s^2 + k11 km22 s^2 + 2 k21 km22 s^2 + k22 km22 s^2 + 2 km11 km22 s^2 +
2 km12 km22 s^2 + km21 km22 s^2 + k11 s^3 + k12 s^3 + 2 k21 s^3 + 2 k22 s^3 + 2 km11 s^3 +
2 km12 s^3 + km21 s^3 + km22 s^3 + s^4 + gammam1 (k21 + k22 + km11 + km12 + s)
  (km12 km21 + k21 s + k22 s + km12 s + km21 s + s^2 + k11 (k21 + k22 + s) + km11 (km21 + s)) +
gamma1 (k21 + k22 + km11 + km12 + s)
  (km12 km22 + k21 s + k22 s + km12 s + km22 s + s^2 + k12 (k21 + k22 + s) + km11 (km22 + s))))
```

```
In[41]:= Pminus = Function[s,
  ((km11 + km12) (k11 k12^2 k21^3 km21 + 2 k11 k12^2 k21^2 k22 km21 + k11 k12^2 k21 k22^2 km21 +
      2 k11 k12^2 k21^2 km11 km21 + 3 k11 k12^2 k21 k22 km11 km21 + k11 k12^2 k22^2 km11 km21 +
      k11 k12^2 k21 km11^2 km21 + k11 k12^2 k22 km11^2 km21 + k11 k12^2 k21^2 km12 km21 +
      k11 k12^2 k21 k22 km12 km21 + k11 k12^2 k21 km11 km12 km21 +
      k11 k12^2 k22 km11 km12 km21 + k12^2 k21^2 k22 km21^2 + k12^2 k21 k22^2 km21^2 +
      k12^2 k21^2 km11 km21^2 + 2 k12^2 k21 k22 km11 km21^2 + k12^2 k22^2 km11 km21^2 +
      2 k12^2 k21 km11^2 km21^2 + k12^2 k22 km11^2 km21^2 + k12^2 km11^3 km21^2 +
      k12^2 k21^2 km12 km21^2 + k12^2 k21 k22 km12 km21^2 + 2 k12^2 k21 km11 km12 km21^2 +
      k12^2 k22 km11 km12 km21^2 + k12^2 km11^2 km12 km21^2 + k11^2 k12 k21^2 k22 km22 +
      2 k11^2 k12 k21 k22^2 km22 + k11^2 k12 k22^3 km22 + k11^2 k12 k21 k22 km11 km22 +
      k11^2 k12 k22^2 km11 km22 + k11^2 k12 k21^2 km12 km22 + 3 k11^2 k12 k21 k22 km12 km22 +
      2 k11^2 k12 k22^2 km12 km22 + k11^2 k12 k21 km11 km12 km22 + k11^2 k12 k22 km11 km12 km22 +
      k11^2 k12 k21 km12^2 km22 + k11^2 k12 k22 km12^2 km22 + 2 k11 k12 k21^3 km21 km22 +
      4 k11 k12 k21^2 k22 km21 km22 + 4 k11 k12 k21 k22^2 km21 km22 + 2 k11 k12 k22^3 km21 km22 +
      4 k11 k12 k21^2 km11 km21 km22 + 7 k11 k12 k21 k22 km11 km21 km22 +
      3 k11 k12 k22^2 km11 km21 km22 + 2 k11 k12 k21 km11^2 km21 km22 +
      3 k11 k12 k22 km11^2 km21 km22 + 3 k11 k12 k21^2 km12 km21 km22 +
      7 k11 k12 k21 k22 km12 km21 km22 + 4 k11 k12 k22^2 km12 km21 km22 +
      5 k11 k12 k21 km11 km12 km21 km22 + 5 k11 k12 k22 km11 km12 km21 km22 +
      2 k11 k12 km11^2 km12 km21 km22 + 3 k11 k12 k21 km12^2 km21 km22 +
      2 k11 k12 k22 km12^2 km21 km22 + 2 k11 k12 km11 km12^2 km21 km22 +
```

$k12\ k21^2\ k22\ km21^2\ km22 + 2\ k12\ k21\ k22^2\ km21^2\ km22 + k12\ k22^3\ km21^2\ km22 +$
$2\ k12\ k21^2\ km11\ km21^2\ km22 + 4\ k12\ k21\ k22\ km11\ km21^2\ km22 +$
$2\ k12\ k22^2\ km11\ km21^2\ km22 + 4\ k12\ k21\ km11^2\ km21^2\ km22 +$
$3\ k12\ k22\ km11^2\ km21^2\ km22 + 2\ k12\ km11^3\ km21^2\ km22 + 2\ k12\ k21^2\ km12\ km21^2\ km22 +$
$4\ k12\ k21\ k22\ km12\ km21^2\ km22 + 2\ k12\ k22^2\ km12\ km21^2\ km22 +$
$6\ k12\ k21\ km11\ km12\ km21^2\ km22 + 4\ k12\ k22\ km11\ km12\ km21^2\ km22 +$
$4\ k12\ km11^2\ km12\ km21^2\ km22 + 2\ k12\ k21\ km12^2\ km21^2\ km22 + k12\ k22\ km12^2\ km21^2\ km22 +$
$2\ k12\ km11\ km12^2\ km21^2\ km22 + k11^2\ k21^2\ k22\ km22^2 + k11^2\ k21\ k22^2\ km22^2 +$
$k11^2\ k21\ k22\ km11\ km22^2 + k11^2\ k22^2\ km11\ km22^2 + k11^2\ k21^2\ km12\ km22^2 +$
$2\ k11^2\ k21\ k22\ km12\ km22^2 + k11^2\ k22^2\ km12\ km22^2 + k11^2\ k21\ km11\ km12\ km22^2 +$
$2\ k11^2\ k22\ km11\ km12\ km22^2 + k11^2\ k21\ km12^2\ km22^2 + 2\ k11^2\ k22\ km12^2\ km22^2 +$
$k11^2\ km11\ km12^2\ km22^2 + k11^2\ km12^3\ km22^2 + k11\ k21^3\ km21\ km22^2 +$
$2\ k11\ k21^2\ k22\ km21\ km22^2 + k11\ k21\ k22^2\ km21\ km22^2 + 2\ k11\ k21^2\ km11\ km21\ km22^2 +$
$4\ k11\ k21\ k22\ km11\ km21\ km22^2 + 2\ k11\ k22^2\ km11\ km21\ km22^2 +$
$k11\ k21\ km11^2\ km21\ km22^2 + 2\ k11\ k22\ km11^2\ km21\ km22^2 + 2\ k11\ k21^2\ km12\ km21\ km22^2 +$
$4\ k11\ k21\ k22\ km12\ km21\ km22^2 + 2\ k11\ k22^2\ km12\ km21\ km22^2 +$
$4\ k11\ k21\ km11\ km12\ km21\ km22^2 + 6\ k11\ k22\ km11\ km12\ km21\ km22^2 +$
$2\ k11\ km11^2\ km12\ km21\ km22^2 + 3\ k11\ k21\ km12^2\ km21\ km22^2 + 4\ k11\ k22\ km12^2\ km21\ km22^2 +$
$4\ k11\ km11\ km12^2\ km21\ km22^2 + 2\ k11\ km12^3\ km21\ km22^2 + k21^2\ km11\ km21^2\ km22^2 +$
$2\ k21\ k22\ km11\ km21^2\ km22^2 + k22^2\ km11\ km21^2\ km22^2 + 2\ k21\ km11^2\ km21^2\ km22^2 +$
$2\ k22\ km11^2\ km21^2\ km22^2 + km11^3\ km21^2\ km22^2 + k21^2\ km12\ km21^2\ km22^2 +$
$2\ k21\ k22\ km12\ km21^2\ km22^2 + k22^2\ km12\ km21^2\ km22^2 + 4\ k21\ km11\ km12\ km21^2\ km22^2 +$
$4\ k22\ km11\ km12\ km21^2\ km22^2 + 3\ km11^2\ km12\ km21^2\ km22^2 + 2\ k21\ km12^2\ km21^2\ km22^2 +$
$2\ k22\ km12^2\ km21^2\ km22^2 + 3\ km11\ km12^2\ km21^2\ km22^2 + km12^3\ km21^2\ km22^2 +$
$k11\ k12^2\ k21^2\ km21\ s + k11\ k12\ k21^3\ km21\ s + k11\ k12^2\ k21\ k22\ km21\ s +$
$2\ k11\ k12\ k21^2\ k22\ km21\ s + k11\ k12\ k21\ k22^2\ km21\ s + k11\ k12^2\ k21\ km11\ km21\ s +$
$2\ k11\ k12\ k21^2\ km11\ km21\ s + 2\ k11\ k12\ k21\ k22\ km11\ km21\ s + k11\ k12\ k21\ km11^2\ km21\ s +$
$k11\ k12^2\ k21\ km12\ km21\ s + 2\ k11\ k12\ k21^2\ km12\ km21\ s + 2\ k11\ k12\ k21\ k22\ km12\ km21\ s +$
$2\ k11\ k12\ k21\ km11\ km12\ km21\ s + k11\ k12\ k21\ km12^2\ km21\ s + k12^2\ k21\ k22\ km21^2\ s +$
$k12\ k21^2\ k22\ km21^2\ s + k12\ k21\ k22^2\ km21^2\ s + k12^2\ k21\ km11\ km21^2\ s +$
$k12\ k21^2\ km11\ km21^2\ s + 2\ k12\ k21\ k22\ km11\ km21^2\ s + k12^2\ km11^2\ km21^2\ s +$
$2\ k12\ k21\ km11^2\ km21^2\ s + k12\ k22\ km11^2\ km21^2\ s + k12\ km11^3\ km21^2\ s +$
$k12^2\ k21\ km12\ km21^2\ s + k12\ k21^2\ km12\ km21^2\ s + 2\ k12\ k21\ k22\ km12\ km21^2\ s +$
$2\ k12\ k21\ km11\ km12\ km21^2\ s + k12\ km11^2\ km12\ km21^2\ s + k12\ k21\ km12^2\ km21^2\ s +$
$k11^2\ k12\ k21\ k22\ km22\ s + k11\ k12\ k21^2\ k22\ km22\ s + k11^2\ k12\ k22^2\ km22\ s +$
$2\ k11\ k12\ k21\ k22^2\ km22\ s + k11\ k12\ k22^3\ km22\ s + k11^2\ k12\ k22\ km11\ km22\ s +$
$2\ k11\ k12\ k21\ k22\ km11\ km22\ s + 2\ k11\ k12\ k22^2\ km11\ km22\ s +$
$k11\ k12\ k22\ km11^2\ km22\ s + k11^2\ k12\ k22\ km12\ km22\ s + 2\ k11\ k12\ k21\ k22\ km12\ km22\ s +$
$2\ k11\ k12\ k22^2\ km12\ km22\ s + 2\ k11\ k12\ k22\ km11\ km12\ km22\ s +$
$k11\ k12\ k22\ km12^2\ km22\ s + 2\ k11\ k12\ k21^2\ km21\ km22\ s + k11\ k21^3\ km21\ km22\ s +$
$2\ k11\ k12\ k21\ k22\ km21\ km22\ s + k11\ k21^2\ k22\ km21\ km22\ s + 2\ k11\ k12\ k22^2\ km21\ km22\ s +$
$k12\ k21\ k22^2\ km21\ km22\ s + k12\ k22^3\ km21\ km22\ s + 2\ k11\ k12\ k21\ km11\ km21\ km22\ s +$
$2\ k11\ k21^2\ km11\ km21\ km22\ s + 2\ k11\ k12\ k22\ km11\ km21\ km22\ s +$
$2\ k11\ k21\ k22\ km11\ km21\ km22\ s + k11\ k22^2\ km11\ km21\ km22\ s +$

$$k12\ k22^2\ km11\ km21\ km22\ s + k11\ k21\ km11^2\ km21\ km22\ s + k11\ k22\ km11^2\ km21\ km22\ s +$$
$$2\ k11\ k12\ k21\ km12\ km21\ km22\ s + k11\ k21^2\ km12\ km21\ km22\ s +$$
$$k12\ k21^2\ km12\ km21\ km22\ s + 2\ k11\ k12\ k22\ km12\ km21\ km22\ s +$$
$$2\ k12\ k21\ k22\ km12\ km21\ km22\ s + 2\ k12\ k22^2\ km12\ km21\ km22\ s +$$
$$2\ k11\ k12\ km11\ km12\ km21\ km22\ s + 2\ k11\ k21\ km11\ km12\ km21\ km22\ s +$$
$$2\ k12\ k21\ km11\ km12\ km21\ km22\ s + 2\ k11\ k22\ km11\ km12\ km21\ km22\ s +$$
$$2\ k12\ k22\ km11\ km12\ km21\ km22\ s + k11\ km11^2\ km12\ km21\ km22\ s +$$
$$k12\ km11^2\ km12\ km21\ km22\ s + k12\ k21\ km12^2\ km21\ km22\ s + k12\ k22\ km12^2\ km21\ km22\ s +$$
$$k11\ km11\ km12^2\ km21\ km22\ s + k12\ km11\ km12^2\ km21\ km22\ s + k12\ k21\ k22\ km21^2\ km22\ s +$$
$$k12\ k22^2\ km21^2\ km22\ s + 2\ k12\ k21\ km11\ km21^2\ km22\ s + k21^2\ km11\ km21^2\ km22\ s +$$
$$k12\ k22\ km11\ km21^2\ km22\ s + 2\ k21\ k22\ km11\ km21^2\ km22\ s + k22^2\ km11\ km21^2\ km22\ s +$$
$$2\ k12\ km11^2\ km21^2\ km22\ s + 2\ k21\ km11^2\ km21^2\ km22\ s + 2\ k22\ km11^2\ km21^2\ km22\ s +$$
$$km11^3\ km21^2\ km22\ s + 2\ k12\ k21\ km12\ km21^2\ km22\ s + k12\ k22\ km12\ km21^2\ km22\ s +$$
$$2\ k12\ km11\ km12\ km21^2\ km22\ s + 2\ k21\ km11\ km12\ km21^2\ km22\ s +$$
$$2\ k22\ km11\ km12\ km21^2\ km22\ s + 2\ km11^2\ km12\ km21^2\ km22\ s + km11\ km12^2\ km21^2\ km22\ s +$$
$$k11^2\ k21\ k22\ km22^2\ s + k11\ k21^2\ k22\ km22^2\ s + k11\ k21\ k22^2\ km22^2\ s +$$
$$k11^2\ k22\ km11\ km22^2\ s + 2\ k11\ k21\ k22\ km11\ km22^2\ s + k11\ k22^2\ km11\ km22^2\ s +$$
$$k11\ k22\ km11^2\ km22^2\ s + k11^2\ k22\ km12\ km22^2\ s + 2\ k11\ k21\ k22\ km12\ km22^2\ s +$$
$$k11\ k22^2\ km12\ km22^2\ s + 2\ k11\ k22\ km11\ km12\ km22^2\ s + k11^2\ km12^2\ km22^2\ s +$$
$$k11\ k21\ km12^2\ km22^2\ s + 2\ k11\ k22\ km12^2\ km22^2\ s + k11\ km11\ km12^2\ km22^2\ s +$$
$$k11\ km12^3\ km22^2\ s + k11\ k21^2\ km21\ km22^2\ s + k11\ k21\ k22\ km21\ km22^2\ s +$$
$$k11\ k21\ km11\ km21\ km22^2\ s + 2\ k11\ k22\ km11\ km21\ km22^2\ s +$$
$$k11\ k21\ km12\ km21\ km22^2\ s + k21^2\ km12\ km21\ km22^2\ s + 2\ k11\ k22\ km12\ km21\ km22^2\ s +$$
$$2\ k21\ k22\ km12\ km21\ km22^2\ s + k22^2\ km12\ km21\ km22^2\ s + 2\ k11\ km11\ km12\ km21\ km22^2\ s +$$
$$2\ k21\ km11\ km12\ km21\ km22^2\ s + 2\ k22\ km11\ km12\ km21\ km22^2\ s +$$
$$km11^2\ km12\ km21\ km22^2\ s + 2\ k11\ km12^2\ km21\ km22^2\ s + 2\ k21\ km12^2\ km21\ km22^2\ s +$$
$$2\ k22\ km12^2\ km21\ km22^2\ s + 2\ km11\ km12^2\ km21\ km22^2\ s + km12^3\ km21\ km22^2\ s +$$
$$k21\ km11\ km21^2\ km22^2\ s + k22\ km11\ km21^2\ km22^2\ s + km11^2\ km21^2\ km22^2\ s +$$
$$k21\ km12\ km21^2\ km22^2\ s + k22\ km12\ km21^2\ km22^2\ s + 2\ km11\ km12\ km21^2\ km22^2\ s +$$
$$km12^2\ km21^2\ km22^2\ s + k11\ k12\ k21^2\ km21\ s^2 + k11\ k12\ k21\ k22\ km21\ s^2 +$$
$$k11\ k12\ k21\ km11\ km21\ s^2 + k11\ k12\ k21\ km12\ km21\ s^2 + k12\ k21\ k22\ km21^2\ s^2 +$$
$$k12\ k21\ km11\ km21^2\ s^2 + k12\ km11^2\ km21^2\ s^2 + k12\ k21\ km12\ km21^2\ s^2 +$$
$$k11\ k12\ k21\ k22\ km22\ s^2 + k11\ k12\ k22^2\ km22\ s^2 + k11\ k12\ k22\ km11\ km22\ s^2 +$$
$$k11\ k12\ k22\ km12\ km22\ s^2 + k11\ k21^2\ km21\ km22\ s^2 + k12\ k22^2\ km21\ km22\ s^2 +$$
$$k11\ k21\ km11\ km21\ km22\ s^2 + k11\ k22\ km11\ km21\ km22\ s^2 + k12\ k21\ km12\ km21\ km22\ s^2 +$$
$$k12\ k22\ km12\ km21\ km22\ s^2 + k11\ km11\ km12\ km21\ km22\ s^2 + k12\ km11\ km12\ km21\ km22\ s^2 +$$
$$k21\ km11\ km21^2\ km22\ s^2 + k22\ km11\ km21^2\ km22\ s^2 + km11^2\ km21^2\ km22\ s^2 +$$
$$km11\ km12\ km21^2\ km22\ s^2 + k11\ k21\ k22\ km22^2\ s^2 + k11\ k22\ km11\ km22^2\ s^2 +$$
$$k11\ k22\ km12\ km22^2\ s^2 + k11\ km12^2\ km22^2\ s^2 + k21\ km12\ km21\ km22^2\ s^2 +$$
$$k22\ km12\ km21\ km22^2\ s^2 + km11\ km12\ km21\ km22^2\ s^2 + km12^2\ km21\ km22^2\ s^2 +$$
$$gammam1^2\ (k21 + k22 + km11 + km12)\ km21\ (k11\ (k21 + k22) + (km11 + km12)\ km21)$$
$$(k21 + k22 + km11 + km12 + s) + gamma1^2\ (k21 + k22 + km11 + km12)\ km22$$
$$(k12\ (k21 + k22) + (km11 + km12)\ km22)\ (k21 + k22 + km11 + km12 + s) +$$

```
gammam1 (gamma1 (k21 + k22 + km11 + km12) (k12 (k21 + k22) km21 +
        k11 (k21 + k22) km22 + 2 (km11 + km12) km21 km22) (k21 + k22 + km11 + km12 + s) +
    k11^2 (k21 + k22 + km11 + km12) km22 (k21 (k22 + km12) + k22 (k22 + km12 + s)) +
    km21 (k21 + k22 + km11 + km12 + s) (k12 (k22^2 + k22 (km11 + km12) +
            2 km11 (km11 + km12) + k21 (k22 + 2 (km11 + km12))) km21 +
        (k21 + k22 + km11 + km12) (km12 km22 (2 km21 + s) + km11 km21 (2 km22 + s))) +
    k11 (k12 (k21 + k22 + km11 + km12) km21 (2 k21^2 + k22 (k22 + 2 km11 + km12 + s) +
            k21 (3 k22 + 2 km11 + km12 + 2 s)) + (k21 + k22 + km11 + km12 + s)
         (2 km12 (km11 + km12) km21 km22 + k22^2 km22 (km21 + s) +
            k22 (km11 + km12) km22 (3 km21 + s) + k21^2 km21 (2 km22 + s) + k21
              (km11 + km12) km21 (2 km22 + s) + k21 k22 (km22 s + km21 (3 km22 + s))))) +
gamma1 (k12^2 (k21 + k22 + km11 + km12) km21 (k21^2 + k22 km11 + k21 (k22 + km11 + s)) +
    km22 (k21 + k22 + km11 + km12 + s)
      (k11 (k21^2 + 2 (k22 + km12) (km11 + km12) + k21 (k22 + km11 + km12)) km22 +
        (k21 + k22 + km11 + km12) (km12 km22 (2 km21 + s) + km11 km21 (2 km22 + s))) +
    k12 (k11 (k21 + k22 + km11 + km12) km22 (k21^2 + k21 (3 k22 + km11 + 2 km12 + s) +
            k22 (2 k22 + km11 + 2 (km12 + s))) + (k21 + k22 + km11 + km12 + s)
         (2 km11 (km11 + km12) km21 km22 + k22^2 km22 (2 km21 + s) + k22
              (km11 + km12) km22 (2 km21 + s) + k21^2 km21 (km22 + s) + k21 (km11 + km12)
             km21 (3 km22 + s) + k21 k22 (km22 s + km21 (3 km22 + s)))))) /
((k11 k12 k21^2 + 2 k11 k12 k21 k22 + k11 k12 k22^2 + k11 k12 k21 km11 +
    k11 k12 k22 km11 + k11 k12 k21 km12 + k11 k12 k22 km12 +
    k12 k21 k22 km21 + k12 k22^2 km21 + k12 k21 km11 km21 + k12 km11^2 km21 +
    2 k12 k21 km12 km21 + k12 k22 km12 km21 + k12 km11 km12 km21 +
    gammam1 (k21 + k22 + km11 + km12) (k11 (k21 + k22) + (km11 + km12) km21) +
    k11 k21^2 km22 + k11 k21 k22 km22 + k11 k21 km11 km22 + 2 k11 k22 km11 km22 +
    k11 k22 km12 km22 + k11 km11 km12 km22 + k11 km12^2 km22 + k21 km11 km21 km22 +
    k22 km11 km21 km22 + km11^2 km21 km22 + k21 km12 km21 km22 +
    k22 km12 km21 km22 + 2 km11 km12 km21 km22 + km12^2 km21 km22 +
    gamma1 (k21 + k22 + km11 + km12) (k12 (k21 + k22) + (km11 + km12) km22))
  (k11 k12 k21^2 + 2 k11 k12 k21 k22 + k11 k12 k22^2 + k11 k12 k21 km11 +
    k11 k12 k22 km11 + k11 k12 k21 km12 + k11 k12 k22 km12 + k12 k21 k22 km21 +
    k12 k22^2 km21 + k12 k21 km11 km21 + k12 k22 km11 km21 + k12 km11^2 km21 +
    k12 k21 km12 km21 + k12 k22 km12 km21 + k12 km11 km12 km21 +
    k11 k21^2 km22 + k11 k21 k22 km22 + k11 k21 km11 km22 + k11 k22 km11 km22 +
    k11 k21 km12 km22 + k11 k22 km12 km22 + k11 km11 km12 km22 +
    k11 km12^2 km22 + k21 km11 km21 km22 + k22 km11 km21 km22 + km11^2 km21 km22 +
    k21 km12 km21 km22 + k22 km12 km21 km22 + 2 km11 km12 km21 km22 +
    km12^2 km21 km22 + 2 k11 k12 k21 s + k11 k21^2 s + k12 k21^2 s + 2 k11 k12 k22 s +
    2 k11 k21 k22 s + 2 k12 k21 k22 s + k11 k22^2 s + k12 k22^2 s + k11 k12 km11 s +
    k11 k21 km11 s + 2 k12 k21 km11 s + k11 k22 km11 s + 2 k12 k22 km11 s +
    k12 km11^2 s + k11 k12 km12 s + 2 k11 k21 km12 s + k12 k21 km12 s +
```

```
2 k11 k22 km12 s + k12 k22 km12 s + k11 km11 km12 s + k12 km11 km12 s +
k11 km12^2 s + k12 k21 km21 s + 2 k12 k22 km21 s + k21 k22 km21 s + k22^2 km21 s +
2 k12 km11 km21 s + k21 km11 km21 s + 2 k22 km11 km21 s + km11^2 km21 s +
k12 km12 km21 s + k21 km12 km21 s + 2 k22 km12 km21 s + 2 km11 km12 km21 s +
km12^2 km21 s + 2 k11 k21 km22 s + k21^2 km22 s + k11 k22 km22 s + k21 k22 km22 s +
k11 km11 km22 s + 2 k21 km11 km22 s + k22 km11 km22 s + km11^2 km22 s +
2 k11 km12 km22 s + 2 k21 km12 km22 s + k22 km12 km22 s + 2 km11 km12 km22 s +
km12^2 km22 s + k21 km21 km22 s + k22 km21 km22 s + 2 km11 km21 km22 s +
2 km12 km21 km22 s + k11 k12 s^2 + 2 k11 k21 s^2 + 2 k12 k21 s^2 + k21^2 s^2 +
2 k11 k22 s^2 + 2 k12 k22 s^2 + 2 k21 k22 s^2 + k22^2 s^2 + k11 km11 s^2 + 2 k12 km11 s^2 +
2 k21 km11 s^2 + 2 k22 km11 s^2 + km11^2 s^2 + 2 k11 km12 s^2 + k12 km12 s^2 +
2 k21 km12 s^2 + 2 k22 km12 s^2 + 2 km11 km12 s^2 + km12^2 s^2 + k12 km21 s^2 +
k21 km21 s^2 + 2 k22 km21 s^2 + 2 km11 km21 s^2 + 2 km12 km21 s^2 + k11 km22 s^2 +
2 k21 km22 s^2 + k22 km22 s^2 + 2 km11 km22 s^2 + 2 km12 km22 s^2 + km21 km22 s^2 +
k11 s^3 + k12 s^3 + 2 k21 s^3 + 2 k22 s^3 + 2 km11 s^3 + 2 km12 s^3 + km21 s^3 +
km22 s^3 + s^4 + gammam1 (k21 + k22 + km11 + km12 + s) (km12 km21 + k21 s +
    k22 s + km12 s + km21 s + s^2 + k11 (k21 + k22 + s) + km11 (km21 + s)) +
gamma1 (k21 + k22 + km11 + km12 + s) (km12 km22 + k21 s + k22 s + km12 s +
    km22 s + s^2 + k12 (k21 + k22 + s) + km11 (km22 + s))))]
```

Out[41]=

```
Function[s,
 ((km11 + km12) (k11 k12^2 k21^3 km21 + 2 k11 k12^2 k21^2 k22 km21 + k11 k12^2 k21 k22^2 km21 +
      2 k11 k12^2 k21^2 km11 km21 + 3 k11 k12^2 k21 k22 km11 km21 + k11 k12^2 k22^2 km11 km21 +
      k11 k12^2 k21 km11^2 km21 + k11 k12^2 k22 km11^2 km21 + k11 k12^2 k21^2 km12 km21 +
      k11 k12^2 k21 k22 km12 km21 + k11 k12^2 k21 km11 km12 km21 + k11 k12^2 k22 km11 km12 km21 +
      k12^2 k21^2 k22 km21^2 + k12^2 k21 k22^2 km21^2 + k12^2 k21^2 km11 km21^2 +
      2 k12^2 k21 k22 km11 km21^2 + k12^2 k22^2 km11 km21^2 + 2 k12^2 k21 km11^2 km21^2 +
      k12^2 k22 km11^2 km21^2 + k12^2 km11^3 km21^2 + k12^2 k21^2 km12 km21^2 +
      k12^2 k21 k22 km12 km21^2 + 2 k12^2 k21 km11 km12 km21^2 + k12^2 k22 km11 km12 km21^2 +
      k12^2 km11^2 km12 km21^2 + k11^2 k12 k21^2 k22 km22 + 2 k11^2 k12 k21 k22^2 km22 +
      k11^2 k12 k22^3 km22 + k11^2 k12 k21 k22 km11 km22 + k11^2 k12 k22^2 km11 km22 +
      k11^2 k12 k21^2 km12 km22 + 3 k11^2 k12 k21 k22 km12 km22 + 2 k11^2 k12 k22^2 km12 km22 +
      k11^2 k12 k21 km11 km12 km22 + k11^2 k12 k22 km11 km12 km22 + k11^2 k12 k21 km12^2 km22 +
      k11^2 k12 k22 km12^2 km22 + 2 k11 k12 k21^3 km21 km22 + 4 k11 k12 k21^2 k22 km21 km22 +
      4 k11 k12 k21 k22^2 km21 km22 + 2 k11 k12 k22^3 km21 km22 + 4 k11 k12 k21^2 km11 km21 km22 +
      7 k11 k12 k21 k22 km11 km21 km22 + 3 k11 k12 k22^2 km11 km21 km22 +
      2 k11 k12 k21 km11^2 km21 km22 + 3 k11 k12 k22 km11^2 km21 km22 +
      3 k11 k12 k21^2 km12 km21 km22 + 7 k11 k12 k21 k22 km12 km21 km22 +
      4 k11 k12 k22^2 km12 km21 km22 + 5 k11 k12 k21 km11 km12 km21 km22 +
      5 k11 k12 k22 km11 km12 km21 km22 + 2 k11 k12 km11^2 km12 km21 km22 +
      3 k11 k12 k21 km12^2 km21 km22 + 2 k11 k12 k22 km12^2 km21 km22 +
      2 k11 k12 km11 km12^2 km21 km22 + k12 k21^2 k22 km21^2 km22 + 2 k12 k21 k22^2 km21^2 km22 +
      k12 k22^3 km21^2 km22 + 2 k12 k21^2 km11 km21^2 km22 + 4 k12 k21 k22 km11 km21^2 km22 +
```

$2\ k12\ k22^2\ km11\ km21^2\ km22 + 4\ k12\ k21\ km11^2\ km21^2\ km22 + 3\ k12\ k22\ km11^2\ km21^2\ km22 +$
$2\ k12\ km11^3\ km21^2\ km22 + 2\ k12\ k21^2\ km12\ km21^2\ km22 + 4\ k12\ k21\ k22\ km12\ km21^2\ km22 +$
$2\ k12\ k22^2\ km12\ km21^2\ km22 + 6\ k12\ k21\ km11\ km12\ km21^2\ km22 +$
$4\ k12\ k22\ km11\ km12\ km21^2\ km22 + 4\ k12\ km11^2\ km12\ km21^2\ km22 +$
$2\ k12\ k21\ km12^2\ km21^2\ km22 + k12\ k22\ km12^2\ km21^2\ km22 + 2\ k12\ km11\ km12^2\ km21^2\ km22 +$
$k11^2\ k21^2\ k22\ km22^2 + k11^2\ k21\ k22^2\ km22^2 + k11^2\ k21\ k22\ km11\ km22^2 +$
$k11^2\ k22^2\ km11\ km22^2 + k11^2\ k21^2\ km12\ km22^2 + 2\ k11^2\ k21\ k22\ km12\ km22^2 +$
$k11^2\ k22^2\ km12\ km22^2 + k11^2\ k21\ km11\ km12\ km22^2 + 2\ k11^2\ k22\ km11\ km12\ km22^2 +$
$k11^2\ k21\ km12^2\ km22^2 + 2\ k11^2\ k22\ km12^2\ km22^2 + k11^2\ km11\ km12^2\ km22^2 +$
$k11^2\ km12^3\ km22^2 + k11\ k21^3\ km21\ km22^2 + 2\ k11\ k21^2\ k22\ km21\ km22^2 +$
$k11\ k21\ k22^2\ km21\ km22^2 + 2\ k11\ k21^2\ km11\ km21\ km22^2 + 4\ k11\ k21\ k22\ km11\ km21\ km22^2 +$
$2\ k11\ k22^2\ km11\ km21\ km22^2 + k11\ k21\ km11^2\ km21\ km22^2 + 2\ k11\ k22\ km11^2\ km21\ km22^2 +$
$2\ k11\ k21^2\ km12\ km21\ km22^2 + 4\ k11\ k21\ k22\ km12\ km21\ km22^2 + 2\ k11\ k22^2\ km12\ km21\ km22^2 +$
$4\ k11\ k21\ km11\ km12\ km21\ km22^2 + 6\ k11\ k22\ km11\ km12\ km21\ km22^2 +$
$2\ k11\ km11^2\ km12\ km21\ km22^2 + 3\ k11\ k21\ km12^2\ km21\ km22^2 + 4\ k11\ k22\ km12^2\ km21\ km22^2 +$
$4\ k11\ km11\ km12^2\ km21\ km22^2 + 2\ k11\ km12^3\ km21\ km22^2 + k21^2\ km11\ km21^2\ km22^2 +$
$2\ k21\ k22\ km11\ km21^2\ km22^2 + k22^2\ km11\ km21^2\ km22^2 + 2\ k21\ km11^2\ km21^2\ km22^2 +$
$2\ k22\ km11^2\ km21^2\ km22^2 + km11^3\ km21^2\ km22^2 + k21^2\ km12\ km21^2\ km22^2 +$
$2\ k21\ k22\ km12\ km21^2\ km22^2 + k22^2\ km12\ km21^2\ km22^2 + 4\ k21\ km11\ km12\ km21^2\ km22^2 +$
$4\ k22\ km11\ km12\ km21^2\ km22^2 + 3\ km11^2\ km12\ km21^2\ km22^2 + 2\ k21\ km12^2\ km21^2\ km22^2 +$
$2\ k22\ km12^2\ km21^2\ km22^2 + 3\ km11\ km12^2\ km21^2\ km22^2 + km12^3\ km21^2\ km22^2 +$
$k11\ k12^2\ k21^2\ km21\ s + k11\ k12\ k21^3\ km21\ s + k11\ k12^2\ k21\ k22\ km21\ s +$
$2\ k11\ k12\ k21^2\ k22\ km21\ s + k11\ k12\ k21\ k22^2\ km21\ s + k11\ k12^2\ k21\ km11\ km21\ s +$
$2\ k11\ k12\ k21^2\ km11\ km21\ s + 2\ k11\ k12\ k21\ k22\ km11\ km21\ s + k11\ k12\ k21\ km11^2\ km21\ s +$
$k11\ k12^2\ k21\ km12\ km21\ s + 2\ k11\ k12\ k21^2\ km12\ km21\ s + 2\ k11\ k12\ k21\ k22\ km12\ km21\ s +$
$2\ k11\ k12\ k21\ km11\ km12\ km21\ s + k11\ k12\ k21\ km12^2\ km21\ s + k12^2\ k21\ k22\ km21^2\ s +$
$k12\ k21^2\ k22\ km21^2\ s + k12\ k21\ k22^2\ km21^2\ s + k12^2\ k21\ km11\ km21^2\ s +$
$k12\ k21^2\ km11\ km21^2\ s + 2\ k12\ k21\ k22\ km11\ km21^2\ s + k12^2\ km11^2\ km21^2\ s +$
$2\ k12\ k21\ km11^2\ km21^2\ s + k12\ k22\ km11^2\ km21^2\ s + k12\ km11^3\ km21^2\ s +$
$k12^2\ k21\ km12\ km21^2\ s + k12\ k21^2\ km12\ km21^2\ s + 2\ k12\ k21\ k22\ km12\ km21^2\ s +$
$2\ k12\ k21\ km11\ km12\ km21^2\ s + k12\ km11^2\ km12\ km21^2\ s + k12\ k21\ km12^2\ km21^2\ s +$
$k11^2\ k12\ k21\ k22\ km22\ s + k11\ k12\ k21^2\ k22\ km22\ s + k11^2\ k12\ k22^2\ km22\ s +$
$2\ k11\ k12\ k21\ k22^2\ km22\ s + k11\ k12\ k22^3\ km22\ s + k11^2\ k12\ k22\ km11\ km22\ s +$
$2\ k11\ k12\ k21\ k22\ km11\ km22\ s + 2\ k11\ k12\ k22^2\ km11\ km22\ s + k11\ k12\ k22\ km11^2\ km22\ s +$
$k11^2\ k12\ k22\ km12\ km22\ s + 2\ k11\ k12\ k21\ k22\ km12\ km22\ s + 2\ k11\ k12\ k22^2\ km12\ km22\ s +$
$2\ k11\ k12\ k22\ km11\ km12\ km22\ s + k11\ k12\ k22\ km12^2\ km22\ s + 2\ k11\ k12\ k21^2\ km21\ km22\ s +$
$k11\ k21^3\ km21\ km22\ s + 2\ k11\ k12\ k21\ k22\ km21\ km22\ s + k11\ k21^2\ k22\ km21\ km22\ s +$
$2\ k11\ k12\ k22^2\ km21\ km22\ s + k12\ k21\ k22^2\ km21\ km22\ s + k12\ k22^3\ km21\ km22\ s +$
$2\ k11\ k12\ k21\ km11\ km21\ km22\ s + 2\ k11\ k21^2\ km11\ km21\ km22\ s +$
$2\ k11\ k12\ k22\ km11\ km21\ km22\ s + 2\ k11\ k21\ k22\ km11\ km21\ km22\ s +$
$k11\ k22^2\ km11\ km21\ km22\ s + k12\ k22^2\ km11\ km21\ km22\ s + k11\ k21\ km11^2\ km21\ km22\ s +$
$k11\ k22\ km11^2\ km21\ km22\ s + 2\ k11\ k12\ k21\ km12\ km21\ km22\ s +$
$k11\ k21^2\ km12\ km21\ km22\ s + k12\ k21^2\ km12\ km21\ km22\ s + 2\ k11\ k12\ k22\ km12\ km21\ km22\ s +$
$2\ k12\ k21\ k22\ km12\ km21\ km22\ s + 2\ k12\ k22^2\ km12\ km21\ km22\ s +$

$2\ k11\ k12\ km11\ km12\ km21\ km22\ s + 2\ k11\ k21\ km11\ km12\ km21\ km22\ s +$
$2\ k12\ k21\ km11\ km12\ km21\ km22\ s + 2\ k11\ k22\ km11\ km12\ km21\ km22\ s +$
$2\ k12\ k22\ km11\ km12\ km21\ km22\ s + k11\ km11^2\ km12\ km21\ km22\ s +$
$k12\ km11^2\ km12\ km21\ km22\ s + k12\ k21\ km12^2\ km21\ km22\ s + k12\ k22\ km12^2\ km21\ km22\ s +$
$k11\ km11\ km12^2\ km21\ km22\ s + k12\ km11\ km12^2\ km21\ km22\ s + k12\ k21\ k22\ km21^2\ km22\ s +$
$k12\ k22^2\ km21^2\ km22\ s + 2\ k12\ k21\ km11\ km21^2\ km22\ s + k21^2\ km11\ km21^2\ km22\ s +$
$k12\ k22\ km11\ km21^2\ km22\ s + 2\ k21\ k22\ km11\ km21^2\ km22\ s + k22^2\ km11\ km21^2\ km22\ s +$
$2\ k12\ km11^2\ km21^2\ km22\ s + 2\ k21\ km11^2\ km21^2\ km22\ s + 2\ k22\ km11^2\ km21^2\ km22\ s +$
$km11^3\ km21^2\ km22\ s + 2\ k12\ k21\ km12\ km21^2\ km22\ s + k12\ k22\ km12\ km21^2\ km22\ s +$
$2\ k12\ km11\ km12\ km21^2\ km22\ s + 2\ k21\ km11\ km12\ km21^2\ km22\ s +$
$2\ k22\ km11\ km12\ km21^2\ km22\ s + 2\ km11^2\ km12\ km21^2\ km22\ s + km11\ km12^2\ km21^2\ km22\ s +$
$k11^2\ k21\ k22\ km22^2\ s + k11\ k21^2\ k22\ km22^2\ s + k11\ k21\ k22^2\ km22^2\ s +$
$k11^2\ k22\ km11\ km22^2\ s + 2\ k11\ k21\ k22\ km11\ km22^2\ s + k11\ k22^2\ km11\ km22^2\ s +$
$k11\ k22\ km11^2\ km22^2\ s + k11^2\ k22\ km12\ km22^2\ s + 2\ k11\ k21\ k22\ km12\ km22^2\ s +$
$k11\ k22^2\ km12\ km22^2\ s + 2\ k11\ k22\ km11\ km12\ km22^2\ s + k11^2\ km12^2\ km22^2\ s +$
$k11\ k21\ km12^2\ km22^2\ s + 2\ k11\ k22\ km12^2\ km22^2\ s + k11\ km11\ km12^2\ km22^2\ s +$
$k11\ km12^3\ km22^2\ s + k11\ k21^2\ km21\ km22^2\ s + k11\ k21\ k22\ km21\ km22^2\ s +$
$k11\ k21\ km11\ km21\ km22^2\ s + 2\ k11\ k22\ km11\ km21\ km22^2\ s +$
$k11\ k21\ km12\ km21\ km22^2\ s + k21^2\ km12\ km21\ km22^2\ s + 2\ k11\ k22\ km12\ km21\ km22^2\ s +$
$2\ k21\ k22\ km12\ km21\ km22^2\ s + k22^2\ km12\ km21\ km22^2\ s + 2\ k11\ km11\ km12\ km21\ km22^2\ s +$
$2\ k21\ km11\ km12\ km21\ km22^2\ s + 2\ k22\ km11\ km12\ km21\ km22^2\ s +$
$km11^2\ km12\ km21\ km22^2\ s + 2\ k11\ km12^2\ km21\ km22^2\ s + 2\ k21\ km12^2\ km21\ km22^2\ s +$
$2\ k22\ km12^2\ km21\ km22^2\ s + 2\ km11\ km12^2\ km21\ km22^2\ s + km12^3\ km21\ km22^2\ s +$
$k21\ km11\ km21^2\ km22^2\ s + k22\ km11\ km21^2\ km22^2\ s + km11^2\ km21^2\ km22^2\ s +$
$k21\ km12\ km21^2\ km22^2\ s + k22\ km12\ km21^2\ km22^2\ s + 2\ km11\ km12\ km21^2\ km22^2\ s +$
$km12^2\ km21^2\ km22^2\ s + k11\ k12\ k21^2\ km21\ s^2 + k11\ k12\ k21\ k22\ km21\ s^2 +$
$k11\ k12\ k21\ km11\ km21\ s^2 + k11\ k12\ k21\ km12\ km21\ s^2 + k12\ k21\ k22\ km21^2\ s^2 +$
$k12\ k21\ km11\ km21^2\ s^2 + k12\ km11^2\ km21^2\ s^2 + k12\ k21\ km12\ km21^2\ s^2 +$
$k11\ k12\ k21\ k22\ km22\ s^2 + k11\ k12\ k22^2\ km22\ s^2 + k11\ k12\ k22\ km11\ km22\ s^2 +$
$k11\ k12\ k22\ km12\ km22\ s^2 + k11\ k21^2\ km21\ km22\ s^2 + k12\ k22^2\ km21\ km22\ s^2 +$
$k11\ k21\ km11\ km21\ km22\ s^2 + k11\ k22\ km11\ km21\ km22\ s^2 + k12\ k21\ km12\ km21\ km22\ s^2 +$
$k12\ k22\ km12\ km21\ km22\ s^2 + k11\ km11\ km12\ km21\ km22\ s^2 + k12\ km11\ km12\ km21\ km22\ s^2 +$
$k21\ km11\ km21^2\ km22\ s^2 + k22\ km11\ km21^2\ km22\ s^2 + km11^2\ km21^2\ km22\ s^2 +$
$km11\ km12\ km21^2\ km22\ s^2 + k11\ k21\ k22\ km22^2\ s^2 + k11\ k22\ km11\ km22^2\ s^2 +$
$k11\ k22\ km12\ km22^2\ s^2 + k11\ km12^2\ km22^2\ s^2 + k21\ km12\ km21\ km22^2\ s^2 +$
$k22\ km12\ km21\ km22^2\ s^2 + km11\ km12\ km21\ km22^2\ s^2 + km12^2\ km21\ km22^2\ s^2 +$
$gammam1^2\ (k21 + k22 + km11 + km12)\ km21\ (k11\ (k21 + k22) + (km11 + km12)\ km21)$
$(k21 + k22 + km11 + km12 + s) + gamma1^2\ (k21 + k22 + km11 + km12)\ km22$
$(k12\ (k21 + k22) + (km11 + km12)\ km22)\ (k21 + k22 + km11 + km12 + s) +$
$gammam1\ \Big(gamma1\ (k21 + k22 + km11 + km12)\ (k12\ (k21 + k22)\ km21 +$
$k11\ (k21 + k22)\ km22 + 2\ (km11 + km12)\ km21\ km22)\ (k21 + k22 + km11 + km12 + s) +$
$k11^2\ (k21 + k22 + km11 + km12)\ km22\ (k21\ (k22 + km12) + k22\ (k22 + km12 + s)) + km21$
$(k21 + k22 + km11 + km12 + s)\ \Big(k12\ \Big(k22^2 + k22\ (km11 + km12) + 2\ km11\ (km11 + km12) +$

k21 (k22 + 2 (km11 + km12))) km21 + (k21 + k22 + km11 + km12) (km12 km22
(2 km21 + s) + km11 km21 (2 km22 + s))) + k11 (k12 (k21 + k22 + km11 + km12)
km21 (2 k21^2 + k22 (k22 + 2 km11 + km12 + s) + k21 (3 k22 + 2 km11 + km12 + 2 s)) +
(k21 + k22 + km11 + km12 + s) (2 km12 (km11 + km12) km21 km22 + k22^2 km22 (km21 +
s) + k22 (km11 + km12) km22 (3 km21 + s) + k21^2 km21 (2 km22 + s) + k21
(km11 + km12) km21 (2 km22 + s) + k21 k22 (km22 s + km21 (3 km22 + s))))) +
gamma1 (k12^2 (k21 + k22 + km11 + km12) km21 (k21^2 + k22 km11 + k21 (k22 + km11 + s)) +
km22 (k21 + k22 + km11 + km12 + s)
(k11 (k21^2 + 2 (k22 + km12) (km11 + km12) + k21 (k22 + km11 + km12)) km22 +
(k21 + k22 + km11 + km12) (km12 km22 (2 km21 + s) + km11 km21 (2 km22 + s))) +
k12 (k11 (k21 + k22 + km11 + km12) km22 (k21^2 + k21 (3 k22 + km11 + 2 km12 + s) +
k22 (2 k22 + km11 + 2 (km12 + s))) + (k21 + k22 + km11 + km12 + s)
(2 km11 (km11 + km12) km21 km22 + k22^2 km22 (2 km21 + s) + k22
(km11 + km12) km22 (2 km21 + s) + k21^2 km21 (km22 + s) + k21 (km11 + km12)
km21 (3 km22 + s) + k21 k22 (km22 s + km21 (3 km22 + s)))))) /
((k11 k12 k21^2 + 2 k11 k12 k21 k22 + k11 k12 k22^2 + k11 k12 k21 km11 +
k11 k12 k22 km11 + k11 k12 k21 km12 + k11 k12 k22 km12 +
k12 k21 k22 km21 + k12 k22^2 km21 + k12 k21 km11 km21 + k12 km11^2 km21 +
2 k12 k21 km12 km21 + k12 k22 km12 km21 + k12 km11 km12 km21 +
gammam1 (k21 + k22 + km11 + km12) (k11 (k21 + k22) + (km11 + km12) km21) +
k11 k21^2 km22 + k11 k21 k22 km22 + k11 k21 km11 km22 + 2 k11 k22 km11 km22 +
k11 k22 km12 km22 + k11 km11 km12 km22 + k11 km12^2 km22 + k21 km11 km21 km22 +
k22 km11 km21 km22 + km11^2 km21 km22 + k21 km12 km21 km22 +
k22 km12 km21 km22 + 2 km11 km12 km21 km22 + km12^2 km21 km22 +
gamma1 (k21 + k22 + km11 + km12) (k12 (k21 + k22) + (km11 + km12) km22))
(k11 k12 k21^2 + 2 k11 k12 k21 k22 + k11 k12 k22^2 + k11 k12 k21 km11 +
k11 k12 k22 km11 + k11 k12 k21 km12 + k11 k12 k22 km12 + k12 k21 k22 km21 +
k12 k22^2 km21 + k12 k21 km11 km21 + k12 k22 km11 km21 + k12 km11^2 km21 +
k12 k21 km12 km21 + k12 k22 km12 km21 + k12 km11 km12 km21 +
k11 k21^2 km22 + k11 k21 k22 km22 + k11 k21 km11 km22 + k11 k22 km11 km22 +
k11 k21 km12 km22 + k11 k22 km12 km22 + k11 km11 km12 km22 +
k11 km12^2 km22 + k21 km11 km21 km22 + k22 km11 km21 km22 + km11^2 km21 km22 +
k21 km12 km21 km22 + k22 km12 km21 km22 + 2 km11 km12 km21 km22 +
km12^2 km21 km22 + 2 k11 k12 k21 s + k11 k21^2 s + k12 k21^2 s + 2 k11 k12 k22 s +
2 k11 k21 k22 s + 2 k12 k21 k22 s + k11 k22^2 s + k12 k22^2 s + k11 k12 km11 s +
k11 k21 km11 s + 2 k12 k21 km11 s + k11 k22 km11 s + 2 k12 k22 km11 s +
k12 km11^2 s + k11 k12 km12 s + 2 k11 k21 km12 s + k12 k21 km12 s +
2 k11 k22 km12 s + k12 k22 km12 s + k11 km11 km12 s + k12 km11 km12 s +
k11 km12^2 s + k12 k21 km21 s + 2 k12 k22 km21 s + k21 k22 km21 s + k22^2 km21 s +
2 k12 km11 km21 s + k21 km11 km21 s + 2 k22 km11 km21 s + km11^2 km21 s +
k12 km12 km21 s + k21 km12 km21 s + 2 k22 km12 km21 s + 2 km11 km12 km21 s +
km12^2 km21 s + 2 k11 k21 km22 s + k21^2 km22 s + k11 k22 km22 s +

```
k21 k22 km22 s + k11 km11 km22 s + 2 k21 km11 km22 s + k22 km11 km22 s +
km11^2 km22 s + 2 k11 km12 km22 s + 2 k21 km12 km22 s + k22 km12 km22 s +
2 km11 km12 km22 s + km12^2 km22 s + k21 km21 km22 s + k22 km21 km22 s +
2 km11 km21 km22 s + 2 km12 km21 km22 s + k11 k12 s^2 + 2 k11 k21 s^2 +
2 k12 k21 s^2 + k21^2 s^2 + 2 k11 k22 s^2 + 2 k12 k22 s^2 + 2 k21 k22 s^2 + k22^2 s^2 +
k11 km11 s^2 + 2 k12 km11 s^2 + 2 k21 km11 s^2 + 2 k22 km11 s^2 + km11^2 s^2 +
2 k11 km12 s^2 + k12 km12 s^2 + 2 k21 km12 s^2 + 2 k22 km12 s^2 + 2 km11 km12 s^2 +
km12^2 s^2 + k12 km21 s^2 + k21 km21 s^2 + 2 k22 km21 s^2 + 2 km11 km21 s^2 +
2 km12 km21 s^2 + k11 km22 s^2 + 2 k21 km22 s^2 + k22 km22 s^2 + 2 km11 km22 s^2 +
2 km12 km22 s^2 + km21 km22 s^2 + k11 s^3 + k12 s^3 + 2 k21 s^3 + 2 k22 s^3 + 2 km11 s^3 +
2 km12 s^3 + km21 s^3 + km22 s^3 + s^4 + gammam1 (k21 + k22 + km11 + km12 + s)
  (km12 km21 + k21 s + k22 s + km12 s + km21 s + s^2 + k11 (k21 + k22 + s) + km11 (km21 + s)) +
gamma1 (k21 + k22 + km11 + km12 + s) (km12 km22 + k21 s + k22 s +
    km12 s + km22 s + s^2 + k12 (k21 + k22 + s) + km11 (km22 + s)))))]
```

In[42]:= **pplus = Factor[Simplify[Together[Pplus[0]]]]**

Out[42]=

```
((k21 + k22) (gammam1 k11 k21 + gamma1 k12 k21 + k11 k12 k21 +
    gammam1 k11 k22 + gamma1 k12 k22 + k11 k12 k22 + gammam1 k11 km11 +
    gamma1 k12 km11 + k11 k12 km11 + gammam1 k11 km12 + gamma1 k12 km12 +
    k11 k12 km12 + k12 k22 km21 + k12 km12 km21 + k11 k21 km22 + k11 km11 km22)) /
 (gammam1 k11 k21^2 + gamma1 k12 k21^2 + k11 k12 k21^2 + 2 gammam1 k11 k21 k22 +
   2 gamma1 k12 k21 k22 + 2 k11 k12 k21 k22 + gammam1 k11 k22^2 + gamma1 k12 k22^2 +
   k11 k12 k22^2 + gammam1 k11 k21 km11 + gamma1 k12 k21 km11 + k11 k12 k21 km11 +
   gammam1 k11 k22 km11 + gamma1 k12 k22 km11 + k11 k12 k22 km11 + gammam1 k11 k21 km12 +
   gamma1 k12 k21 km12 + k11 k12 k21 km12 + gammam1 k11 k22 km12 + gamma1 k12 k22 km12 +
   k11 k12 k22 km12 + k12 k21 k22 km21 + k12 k22^2 km21 + gammam1 k21 km11 km21 +
   k12 k21 km11 km21 + gammam1 k22 km11 km21 + gammam1 km11^2 km21 + k12 km11^2 km21 +
   gammam1 k21 km12 km21 + 2 k12 k21 km12 km21 + gammam1 k22 km12 km21 + k12 k22 km12 km21 +
   2 gammam1 km11 km12 km21 + k12 km11 km12 km21 + gammam1 km12^2 km21 + k11 k21^2 km22 +
   k11 k21 k22 km22 + gamma1 k21 km11 km22 + k11 k21 km11 km22 + gamma1 k22 km11 km22 +
   2 k11 k22 km11 km22 + gamma1 km11^2 km22 + gamma1 k21 km12 km22 + gamma1 k22 km12 km22 +
   k11 k22 km12 km22 + 2 gamma1 km11 km12 km22 + k11 km11 km12 km22 + gamma1 km12^2 km22 +
   k11 km12^2 km22 + k21 km11 km21 km22 + k22 km11 km21 km22 + km11^2 km21 km22 +
   k21 km12 km21 km22 + k22 km12 km21 km22 + 2 km11 km12 km21 km22 + km12^2 km21 km22)
```

In[43]:= 
```
pminus = Factor[Simplify[Together[Pminus[0]]]]
```

Out[43]=

$$((km11 + km12)\ (gammam1\ k21\ km21 + k12\ k21\ km21 + gammam1\ k22\ km21 + gammam1\ km11\ km21 + k12\ km11\ km21 + gammam1\ km12\ km21 + gamma1\ k21\ km22 + gamma1\ k22\ km22 + k11\ k22\ km22 + gamma1\ km11\ km22 + gamma1\ km12\ km22 + k11\ km12\ km22 + k21\ km21\ km22 + k22\ km21\ km22 + km11\ km21\ km22 + km12\ km21\ km22)) \Big/ \Big(gammam1\ k11\ k21^2 + gamma1\ k12\ k21^2 + k11\ k12\ k21^2 + 2\ gammam1\ k11\ k21\ k22 + 2\ gamma1\ k12\ k21\ k22 + 2\ k11\ k12\ k21\ k22 + gammam1\ k11\ k22^2 + gamma1\ k12\ k22^2 + k11\ k12\ k22^2 + gammam1\ k11\ k21\ km11 + gamma1\ k12\ k21\ km11 + k11\ k12\ k21\ km11 + gammam1\ k11\ k22\ km11 + gamma1\ k12\ k22\ km11 + k11\ k12\ k22\ km11 + gammam1\ k11\ k21\ km12 + gamma1\ k12\ k21\ km12 + k11\ k12\ k21\ km12 + gammam1\ k11\ k22\ km12 + gamma1\ k12\ k22\ km12 + k11\ k12\ k22\ km12 + k12\ k21\ k22\ km21 + k12\ k22^2\ km21 + gammam1\ k21\ km11\ km21 + k12\ k21\ km11\ km21 + gammam1\ k22\ km11\ km21 + gammam1\ km11^2\ km21 + k12\ km11^2\ km21 + gammam1\ k21\ km12\ km21 + 2\ k12\ k21\ km12\ km21 + gammam1\ k22\ km12\ km21 + k12\ k22\ km12\ km21 + 2\ gammam1\ km11\ km12\ km21 + k12\ km11\ km12\ km21 + gammam1\ km12^2\ km21 + k11\ k21^2\ km22 + k11\ k21\ k22\ km22 + gamma1\ k21\ km11\ km22 + k11\ k21\ km11\ km22 + gamma1\ k22\ km11\ km22 + 2\ k11\ k22\ km11\ km22 + gamma1\ km11^2\ km22 + gamma1\ k21\ km12\ km22 + gamma1\ k22\ km12\ km22 + k11\ k22\ km12\ km22 + 2\ gamma1\ km11\ km12\ km22 + k11\ km11\ km12\ km22 + gamma1\ km12^2\ km22 + k11\ km12^2\ km22 + k21\ km11\ km21\ km22 + k22\ km11\ km21\ km22 + km11^2\ km21\ km22 + k21\ km12\ km21\ km22 + k22\ km12\ km21\ km22 + 2\ km11\ km12\ km21\ km22 + km12^2\ km21\ km22\Big)$$

In[44]:= 
```
Km = {{gamma1 + k11 + km21, -gammam1, -k21 - km11},
   {-gamma1, gammam1 + k12 + km22, -k22 - km12},
   {-k11 - km21, -k12 - km22, k21 + k22 + km11 + km12}}
```

Out[44]=
```
{{gamma1 + k11 + km21, -gammam1, -k21 - km11},
 {-gamma1, gammam1 + k12 + km22, -k22 - km12},
 {-k11 - km21, -k12 - km22, k21 + k22 + km11 + km12}}
```

In[45]:= 
```
rhos = {{rhos1}, {rhos2}, {1 - rhos1 - rhos2}}
```

Out[45]=
```
{{rhos1}, {rhos2}, {1 - rhos1 - rhos2}}
```

In[46]:= 
```
Simplify[Together[Solve[Km.rhos == 0, {rhos1, rhos2}]]]
```

Out[46]=
```
{{rhos1 → (gammam1 (k21 + k22 + km11 + km12) + (k21 + km11) (k12 + km22)) /
     (k11 k12 + k12 k21 + k11 k22 + k12 km11 + k11 km12 + k12 km21 + k22 km21 +
       km12 km21 + gammam1 (k11 + k21 + k22 + km11 + km12 + km21) + k11 km22 + k21 km22 +
       km11 km22 + km21 km22 + gamma1 (k12 + k21 + k22 + km11 + km12 + km22)),
   rhos2 → (gamma1 (k21 + k22 + km11 + km12) + (k22 + km12) (k11 + km21)) /
     (k11 k12 + k12 k21 + k11 k22 + k12 km11 + k11 km12 + k12 km21 + k22 km21 +
       km12 km21 + gammam1 (k11 + k21 + k22 + km11 + km12 + km21) + k11 km22 + k21 km22 +
       km11 km22 + km21 km22 + gamma1 (k12 + k21 + k22 + km11 + km12 + km22))}}
```

In[47]:=
```
rhos1 = (gammam1 (k21 + k22 + km11 + km12) + (k21 + km11) (k12 + km22)) /
   (k11 k12 + k12 k21 + k11 k22 + k12 km11 + k11 km12 + k12 km21 + k22 km21 +
     km12 km21 + gammam1 (k11 + k21 + k22 + km11 + km12 + km21) + k11 km22 +
     k21 km22 + km11 km22 + km21 km22 + gamma1 (k12 + k21 + k22 + km11 + km12 + km22))
```
Out[47]=
```
(gammam1 (k21 + k22 + km11 + km12) + (k21 + km11) (k12 + km22)) /
  (k11 k12 + k12 k21 + k11 k22 + k12 km11 + k11 km12 + k12 km21 + k22 km21 +
    km12 km21 + gammam1 (k11 + k21 + k22 + km11 + km12 + km21) + k11 km22 +
    k21 km22 + km11 km22 + km21 km22 + gamma1 (k12 + k21 + k22 + km11 + km12 + km22))
```
In[48]:=
```
rhos2 = (gamma1 (k21 + k22 + km11 + km12) + (k22 + km12) (k11 + km21)) /
   (k11 k12 + k12 k21 + k11 k22 + k12 km11 + k11 km12 + k12 km21 + k22 km21 +
     km12 km21 + gammam1 (k11 + k21 + k22 + km11 + km12 + km21) + k11 km22 +
     k21 km22 + km11 km22 + km21 km22 + gamma1 (k12 + k21 + k22 + km11 + km12 + km22))
```
Out[48]=
```
(gamma1 (k21 + k22 + km11 + km12) + (k22 + km12) (k11 + km21)) /
  (k11 k12 + k12 k21 + k11 k22 + k12 km11 + k11 km12 + k12 km21 + k22 km21 +
    km12 km21 + gammam1 (k11 + k21 + k22 + km11 + km12 + km21) + k11 km22 +
    k21 km22 + km11 km22 + km21 km22 + gamma1 (k12 + k21 + k22 + km11 + km12 + km22))
```
In[49]:=
```
Factor[Simplify[Together[rhos]]]
```
Out[49]=
```
{{(gammam1 k21 + k12 k21 + gammam1 k22 +
      gammam1 km11 + k12 km11 + gammam1 km12 + k21 km22 + km11 km22) /
    (gammam1 k11 + gamma1 k12 + k11 k12 + gamma1 k21 + gammam1 k21 + k12 k21 + gamma1 k22 +
      gammam1 k22 + k11 k22 + gamma1 km11 + gammam1 km11 + k12 km11 +
      gamma1 km12 + gammam1 km12 + k11 km12 + gammam1 km21 + k12 km21 + k22 km21 +
      km12 km21 + gamma1 km22 + k11 km22 + k21 km22 + km11 km22 + km21 km22)},
  {(gamma1 k21 + gamma1 k22 + k11 k22 + gamma1 km11 + gamma1 km12 + k11 km12 + k22 km21 +
      km12 km21) / (gammam1 k11 + gamma1 k12 + k11 k12 + gamma1 k21 + gammam1 k21 +
      k12 k21 + gamma1 k22 + gammam1 k22 + k11 k22 + gamma1 km11 + gammam1 km11 +
      k12 km11 + gamma1 km12 + gammam1 km12 + k11 km12 + gammam1 km21 + k12 km21 +
      k22 km21 + km12 km21 + gamma1 km22 + k11 km22 + k21 km22 + km11 km22 + km21 km22)},
  {(gammam1 k11 + gamma1 k12 + k11 k12 + gammam1 km21 + k12 km21 +
      gamma1 km22 + k11 km22 + km21 km22) /
    (gammam1 k11 + gamma1 k12 + k11 k12 + gamma1 k21 + gammam1 k21 + k12 k21 +
      gamma1 k22 + gammam1 k22 + k11 k22 + gamma1 km11 + gammam1 km11 + k12 km11 +
      gamma1 km12 + gammam1 km12 + k11 km12 + gammam1 km21 + k12 km21 + k22 km21 +
      km12 km21 + gamma1 km22 + k11 km22 + k21 km22 + km11 km22 + km21 km22)}}
```
In[50]:=
```
gamma = gamma1 + gammam1
```
Out[50]=
```
gamma1 + gammam1
```

```
In[51]:= J = Simplify[Together[(gamma1 * rhos1 - gammam1 * rhos2) / gamma]]
Out[51]=
(-gammam1 (k22 + km12) (k11 + km21) + gamma1 (k21 + km11) (k12 + km22)) /
  ((gamma1 + gammam1) (k11 k12 + k12 k21 + k11 k22 + k12 km11 + k11 km12 + k12 km21 +
      k22 km21 + km12 km21 + gammam1 (k11 + k21 + k22 + km11 + km12 + km21) + k11 km22 +
      k21 km22 + km11 km22 + km21 km22 + gamma1 (k12 + k21 + k22 + km11 + km12 + km22)))

In[52]:= Solve[k11 * k21 * km12 * km22 - k12 * k22 * km11 * km21 == 0 &&
   k11 * km12 * gammam1 - k12 * km11 * gamma1 == 0, {k12, gammam1}]
Out[52]=
{{k12 -> (k11 k21 km12 km22)/(k22 km11 km21), gammam1 -> (gamma1 k21 km22)/(k22 km21)}}

In[53]:= k12 = (k11 k21 km12 km22)/(k22 km11 km21)
Out[53]=
(k11 k21 km12 km22)/(k22 km11 km21)

In[54]:= gammam1 = (gamma1 k21 km22)/(k22 km21)
Out[54]=
(gamma1 k21 km22)/(k22 km21)

In[55]:= Factor[Simplify[Together[Pplus[s] / Pminus[s] - k11 * k21 / (km11 * km21)]]]
Out[55]=
- ((k11 (k22 km11 - k21 km12)
      (gamma1 k11^2 k21^4 k22 km11^2 km22 + 2 gamma1 k11^2 k21^3 k22^2 km11^2 km22 +
        gamma1 k11^2 k21^2 k22^3 km11^2 km22 + gamma1 k11^2 k21^3 k22 km11^3 km22 +
        gamma1 k11^2 k21^2 k22^2 km11^3 km22 - gamma1 k11^2 k21^5 km11 km12 km22 -
        gamma1 k11^2 k21^4 k22 km11 km12 km22 + k11^3 k21^4 k22 km11 km12 km22 +
        gamma1 k11^2 k21^3 k22^2 km11 km12 km22 + 2 k11^3 k21^3 k22^2 km11 km12 km22 +
        gamma1 k11^2 k21^2 k22^3 km11 km12 km22 + k11^3 k21^2 k22^3 km11 km12 km22 -
        gamma1 k11^2 k21^4 km11^2 km12 km22 + gamma1 k11^2 k21^3 k22 km11^2 km12 km22 +
        k11^3 k21^3 k22 km11^2 km12 km22 + 2 gamma1 k11^2 k21^2 k22^2 km11^2 km12 km22 +
        k11^3 k21^2 k22^2 km11^2 km12 km22 - gamma1 k11^2 k21^5 km12^2 km22 -
        k11^3 k21^5 km12^2 km22 - 2 gamma1 k11^2 k21^4 k22 km12^2 km22 -
        2 k11^3 k21^4 k22 km12^2 km22 - gamma1 k11^2 k21^3 k22^2 km12^2 km22 -
        k11^3 k21^3 k22^2 km12^2 km22 - 2 gamma1 k11^2 k21^4 km11 km12^2 km22 -
        k11^3 k21^4 km11 km12^2 km22 - gamma1 k11^2 k21^3 k22 km11 km12^2 km22 +
        gamma1 k11^2 k21^2 k22^2 km11 km12^2 km22 + k11^3 k21^2 k22^2 km11 km12^2 km22 -
        gamma1 k11^2 k21^4 km12^3 km22 - k11^3 k21^4 km12^3 km22 - gamma1 k11^2 k21^3 k22 km12^3 km22 -
        k11^3 k21^3 k22 km12^3 km22 + k11^2 k21^3 k22^2 km11^2 km21 km22 +
        k11^2 k21^2 k22^3 km11^2 km21 km22 + k11^2 k21^2 k22^2 km11^3 km21 km22 +
        k11^2 k21 k22^3 km11^3 km21 km22 - k11^2 k21^4 k22 km11 km12 km21 km22 +
```

$k11^2\ k21^2\ k22^3\ km11\ km12\ km21\ km22 - k11^2\ k21^3\ k22\ km11^2\ km12\ km21\ km22 -$
$k11^2\ k21^2\ k22^2\ km11^2\ km12\ km21\ km22 - k11^2\ k21^4\ k22\ km12^2\ km21\ km22 -$
$k11^2\ k21^3\ k22^2\ km12^2\ km21\ km22 + k11^2\ k21^3\ k22\ km11\ km12^2\ km21\ km22 +$
$k11^2\ k21^2\ k22^2\ km11\ km12^2\ km21\ km22 - k11^2\ k21^4\ km12^3\ km21\ km22 -$
$k11^2\ k21^3\ k22\ km12^3\ km21\ km22 - gamma1\ k21^2\ k22\ km11^4\ km21^2\ km22 -$
$2\ gamma1\ k21\ k22^2\ km11^4\ km21^2\ km22 - gamma1\ k22^3\ km11^4\ km21^2\ km22 -$
$k11\ k22^3\ km11^4\ km21^2\ km22 - gamma1\ k21\ k22\ km11^5\ km21^2\ km22 -$
$gamma1\ k22^2\ km11^5\ km21^2\ km22 + gamma1\ k21^3\ km11^3\ km12\ km21^2\ km22 +$
$gamma1\ k21^2\ k22\ km11^3\ km12\ km21^2\ km22 - k11\ k21^2\ k22\ km11^3\ km12\ km21^2\ km22 -$
$gamma1\ k21\ k22^2\ km11^3\ km12\ km21^2\ km22 + k11\ k21\ k22^2\ km11^3\ km12\ km21^2\ km22 -$
$gamma1\ k22^3\ km11^3\ km12\ km21^2\ km22 - k11\ k22^3\ km11^3\ km12\ km21^2\ km22 +$
$gamma1\ k21^2\ km11^4\ km12\ km21^2\ km22 - gamma1\ k21\ k22\ km11^4\ km12\ km21^2\ km22 -$
$k11\ k21\ k22\ km11^4\ km12\ km21^2\ km22 - 2\ gamma1\ k22^2\ km11^4\ km12\ km21^2\ km22 -$
$k11\ k22^2\ km11^4\ km12\ km21^2\ km22 + gamma1\ k21^3\ km11^2\ km12^2\ km21^2\ km22 +$
$k11\ k21^3\ km11^2\ km12^2\ km21^2\ km22 + 2\ gamma1\ k21^2\ k22\ km11^2\ km12^2\ km21^2\ km22 -$
$k11\ k21^2\ k22\ km11^2\ km12^2\ km21^2\ km22 + gamma1\ k21\ k22^2\ km11^2\ km12^2\ km21^2\ km22 +$
$k11\ k21\ k22^2\ km11^2\ km12^2\ km21^2\ km22 + 2\ gamma1\ k21^2\ km11^3\ km12^2\ km21^2\ km22 +$
$k11\ k21^2\ km11^3\ km12^2\ km21^2\ km22 + gamma1\ k21\ k22\ km11^3\ km12^2\ km21^2\ km22 -$
$gamma1\ k22^2\ km11^3\ km12^2\ km21^2\ km22 - k11\ k22^2\ km11^3\ km12^2\ km21^2\ km22 +$
$k11\ k21^3\ km11\ km12^3\ km21^2\ km22 + gamma1\ k21^2\ km11^2\ km12^3\ km21^2\ km22 +$
$k11\ k21^2\ km11^2\ km12^3\ km21^2\ km22 + gamma1\ k21\ k22\ km11^2\ km12^3\ km21^2\ km22 +$
$k11\ k21\ k22\ km11^2\ km12^3\ km21^2\ km22 - k21\ k22^2\ km11^4\ km21^3\ km22 -$
$k22^3\ km11^4\ km21^3\ km22 - k22^2\ km11^5\ km21^3\ km22 + k21^2\ k22\ km11^3\ km12\ km21^3\ km22 -$
$k22^3\ km11^3\ km12\ km21^3\ km22 + k21\ k22\ km11^4\ km12\ km21^3\ km22 -$
$2\ k22^2\ km11^4\ km12\ km21^3\ km22 + k21^2\ k22\ km11^2\ km12^2\ km21^3\ km22 +$
$k21\ k22^2\ km11^2\ km12^2\ km21^3\ km22 + 2\ k21\ k22\ km11^3\ km12^2\ km21^3\ km22 -$
$k22^2\ km11^3\ km12^2\ km21^3\ km22 + k21\ k22\ km11^2\ km12^3\ km21^3\ km22 -$
$gamma1\ k11\ k21^4\ k22\ km11^2\ km21\ s - 2\ gamma1\ k11\ k21^3\ k22^2\ km11^2\ km21\ s -$
$gamma1\ k11\ k21^2\ k22^3\ km11^2\ km21\ s - 2\ gamma1\ k11\ k21^3\ k22\ km11^3\ km21\ s -$
$2\ gamma1\ k11\ k21^2\ k22^2\ km11^3\ km21\ s - gamma1\ k11\ k21^2\ k22\ km11^4\ km21\ s -$
$gamma1\ k11\ k21^4\ k22\ km11\ km12\ km21\ s - k11^2\ k21^4\ k22\ km11\ km12\ km21\ s -$
$2\ gamma1\ k11\ k21^3\ k22^2\ km11\ km12\ km21\ s - 2\ k11^2\ k21^3\ k22^2\ km11\ km12\ km21\ s -$
$gamma1\ k11\ k21^2\ k22^3\ km11\ km12\ km21\ s - k11^2\ k21^2\ k22^3\ km11\ km12\ km21\ s -$
$4\ gamma1\ k11\ k21^3\ k22\ km11^2\ km12\ km21\ s - 2\ k11^2\ k21^3\ k22\ km11^2\ km12\ km21\ s -$
$4\ gamma1\ k11\ k21^2\ k22^2\ km11^2\ km12\ km21\ s - 2\ k11^2\ k21^2\ k22^2\ km11^2\ km12\ km21\ s -$
$3\ gamma1\ k11\ k21^2\ k22\ km11^3\ km12\ km21\ s - k11^2\ k21^2\ k22\ km11^3\ km12\ km21\ s -$
$2\ gamma1\ k11\ k21^3\ k22\ km11\ km12^2\ km21\ s - 2\ k11^2\ k21^3\ k22\ km11\ km12^2\ km21\ s -$
$2\ gamma1\ k11\ k21^2\ k22^2\ km11\ km12^2\ km21\ s - 2\ k11^2\ k21^2\ k22^2\ km11\ km12^2\ km21\ s -$
$3\ gamma1\ k11\ k21^2\ k22\ km11^2\ km12^2\ km21\ s - 2\ k11^2\ k21^2\ k22\ km11^2\ km12^2\ km21\ s -$
$gamma1\ k11\ k21^2\ k22\ km11\ km12^3\ km21\ s - k11^2\ k21^2\ k22\ km11\ km12^3\ km21\ s -$
$k11\ k21^3\ k22^2\ km11^2\ km21^2\ s - k11\ k21^2\ k22^3\ km11^2\ km21^2\ s -$
$gamma1\ k21^3\ k22\ km11^3\ km21^2\ s - 3\ gamma1\ k21^2\ k22^2\ km11^3\ km21^2\ s -$
$2\ k11\ k21^2\ k22^2\ km11^3\ km21^2\ s - 3\ gamma1\ k21\ k22^3\ km11^3\ km21^2\ s -$
$2\ k11\ k21\ k22^3\ km11^3\ km21^2\ s - gamma1\ k22^4\ km11^3\ km21^2\ s - k11\ k22^4\ km11^3\ km21^2\ s -$

$2 gamma1 k21^2 k22 km11^4 km21^2 s - 4 gamma1 k21 k22^2 km11^4 km21^2 s -$
$k11 k21 k22^2 km11^4 km21^2 s - 2 gamma1 k22^3 km11^4 km21^2 s - k11 k22^3 km11^4 km21^2 s -$
$gamma1 k21 k22 km11^5 km21^2 s - gamma1 k22^2 km11^5 km21^2 s -$
$k11 k21^3 k22^2 km11 km12 km21^2 s - k11 k21^2 k22^3 km11 km12 km21^2 s -$
$k11 k21^3 k22 km11^2 km12 km21^2 s - 3 k11 k21^2 k22^2 km11^2 km12 km21^2 s -$
$2 gamma1 k21^2 k22 km11^3 km12 km21^2 s - 2 k11 k21^2 k22 km11^3 km12 km21^2 s -$
$4 gamma1 k21 k22^2 km11^3 km12 km21^2 s - 3 k11 k21 k22^2 km11^3 km12 km21^2 s -$
$2 gamma1 k22^3 km11^3 km12 km21^2 s - 2 k11 k22^3 km11^3 km12 km21^2 s -$
$2 gamma1 k21 k22 km11^4 km12 km21^2 s - k11 k21 k22 km11^4 km12 km21^2 s -$
$2 gamma1 k22^2 km11^4 km12 km21^2 s - k11 k22^2 km11^4 km12 km21^2 s -$
$k11 k21^3 k22 km11 km12^2 km21^2 s - 2 k11 k21^2 k22^2 km11 km12^2 km21^2 s -$
$2 k11 k21^2 k22 km11^2 km12^2 km21^2 s - gamma1 k21 k22 km11^3 km12^2 km21^2 s -$
$k11 k21 k22 km11^3 km12^2 km21^2 s - gamma1 k22^2 km11^3 km12^2 km21^2 s -$
$k11 k22^2 km11^3 km12^2 km21^2 s - k11 k21^2 k22 km11 km12^3 km21^2 s -$
$k21^2 k22^2 km11^3 km21^3 s - 2 k21 k22^3 km11^3 km21^3 s - k22^4 km11^3 km21^3 s -$
$2 k21 k22^2 km11^4 km21^3 s - 2 k22^3 km11^4 km21^3 s - k22^2 km11^5 km21^3 s -$
$2 k21 k22^2 km11^3 km12 km21^3 s - 2 k22^3 km11^3 km12 km21^3 s - 2 k22^2 km11^4 km12 km21^3 s -$
$k22^2 km11^3 km12^2 km21^3 s + gamma1 k11^2 k21^3 k22 km11^2 km22 s +$
$gamma1 k11 k21^4 k22 km11^2 km22 s + gamma1 k11^2 k21^2 k22^2 km11^2 km22 s +$
$2 gamma1 k11 k21^3 k22^2 km11^2 km22 s + gamma1 k11 k21^2 k22^3 km11^2 km22 s +$
$gamma1 k11^2 k21^2 k22 km11^3 km22 s + 2 gamma1 k11 k21^3 k22 km11^3 km22 s +$
$2 gamma1 k11 k21^2 k22^2 km11^3 km22 s + gamma1 k11 k21^2 k22 km11^4 km22 s -$
$gamma1 k11^2 k21^4 km11 km12 km22 s + k11^3 k21^3 k22 km11 km12 km22 s +$
$gamma1 k11 k21^4 k22 km11 km12 km22 s + k11^2 k21^4 k22 km11 km12 km22 s +$
$gamma1 k11^2 k21^2 k22^2 km11 km12 km22 s + k11^3 k21^2 k22^2 km11 km12 km22 s +$
$2 gamma1 k11 k21^3 k22^2 km11 km12 km22 s + 2 k11^2 k21^3 k22^2 km11 km12 km22 s +$
$gamma1 k11 k21^2 k22^3 km11 km12 km22 s + k11^2 k21^2 k22^3 km11 km12 km22 s -$
$gamma1 k11^2 k21^3 km11^2 km12 km22 s + 2 gamma1 k11^2 k21^2 k22 km11^2 km12 km22 s +$
$k11^3 k21^2 k22 km11^2 km12 km22 s + 4 gamma1 k11 k21^3 k22 km11^2 km12 km22 s +$
$2 k11^2 k21^3 k22 km11^2 km12 km22 s + 4 gamma1 k11 k21^2 k22^2 km11^2 km12 km22 s +$
$2 k11^2 k21^2 k22^2 km11^2 km12 km22 s + 3 gamma1 k11 k21^2 k22 km11^3 km12 km22 s +$
$k11^2 k21^2 k22 km11^3 km12 km22 s - gamma1 k11^2 k21^4 km12^2 km22 s -$
$k11^3 k21^4 km12^2 km22 s - gamma1 k11^2 k21^3 k22 km12^2 km22 s -$
$k11^3 k21^3 k22 km12^2 km22 s - 2 gamma1 k11^2 k21^3 km11 km12^2 km22 s -$
$k11^3 k21^3 km11 km12^2 km22 s + gamma1 k11^2 k21^2 k22 km11 km12^2 km22 s +$
$k11^3 k21^2 k22 km11 km12^2 km22 s + 2 gamma1 k11 k21^3 k22 km11 km12^2 km22 s +$
$2 k11^2 k21^3 k22 km11 km12^2 km22 s + 2 gamma1 k11 k21^2 k22^2 km11 km12^2 km22 s +$
$2 k11^2 k21^2 k22^2 km11 km12^2 km22 s + 3 gamma1 k11 k21^2 k22 km11^2 km12^2 km22 s +$
$2 k11^2 k21^2 k22 km11^2 km12^2 km22 s - gamma1 k11^2 k21^3 km12^3 km22 s -$
$k11^3 k21^3 km12^3 km22 s + gamma1 k11 k21^2 k22 km11 km12^3 km22 s +$
$k11^2 k21^2 k22 km11 km12^3 km22 s + k11^2 k21^2 k22^2 km11^2 km21 km22 s +$
$k11 k21^3 k22^2 km11^2 km21 km22 s + k11 k21^2 k22^3 km11^2 km21 km22 s +$
$k11^2 k21 k22^2 km11^3 km21 km22 s + 2 k11 k21^2 k22^2 km11^3 km21 km22 s +$
$k11 k21 k22^3 km11^3 km21 km22 s + k11 k21 k22^2 km11^4 km21 km22 s -$

$k11^2\ k21^3\ k22\ km11\ km12\ km21\ km22\ s + k11^2\ k21^2\ k22^2\ km11\ km12\ km21\ km22\ s +$
$k11\ k21^3\ k22^2\ km11\ km12\ km21\ km22\ s + k11\ k21^2\ k22^3\ km11\ km12\ km21\ km22\ s +$
$gamma1\ k21^4\ km11^2\ km12\ km21\ km22\ s - k11^2\ k21^2\ k22\ km11^2\ km12\ km21\ km22\ s +$
$3\ gamma1\ k21^3\ k22\ km11^2\ km12\ km21\ km22\ s + 3\ gamma1\ k21^2\ k22^2\ km11^2\ km12\ km21\ km22\ s +$
$3\ k11\ k21^2\ k22^2\ km11^2\ km12\ km21\ km22\ s + gamma1\ k21\ k22^3\ km11^2\ km12\ km21\ km22\ s +$
$k11\ k21\ k22^3\ km11^2\ km12\ km21\ km22\ s + 2\ gamma1\ k21^3\ km11^3\ km12\ km21\ km22\ s +$
$4\ gamma1\ k21^2\ k22\ km11^3\ km12\ km21\ km22\ s + 2\ gamma1\ k21\ k22^2\ km11^3\ km12\ km21\ km22\ s +$
$2\ k11\ k21\ k22^2\ km11^3\ km12\ km21\ km22\ s + gamma1\ k21^2\ km11^4\ km12\ km21\ km22\ s +$
$gamma1\ k21\ k22\ km11^4\ km12\ km21\ km22\ s - k11^2\ k21^3\ k22\ km12^2\ km21\ km22\ s +$
$k11\ k21^4\ km11\ km12^2\ km21\ km22\ s + k11^2\ k21^2\ k22\ km11\ km12^2\ km21\ km22\ s +$
$2\ k11\ k21^3\ k22\ km11\ km12^2\ km21\ km22\ s + 2\ k11\ k21^2\ k22^2\ km11\ km12^2\ km21\ km22\ s +$
$2\ gamma1\ k21^3\ km11^2\ km12^2\ km21\ km22\ s + 2\ k11\ k21^3\ km11^2\ km12^2\ km21\ km22\ s +$
$4\ gamma1\ k21^2\ k22\ km11^2\ km12^2\ km21\ km22\ s + 3\ k11\ k21^2\ k22\ km11^2\ km12^2\ km21\ km22\ s +$
$2\ gamma1\ k21\ k22^2\ km11^2\ km12^2\ km21\ km22\ s + 2\ k11\ k21\ k22^2\ km11^2\ km12^2\ km21\ km22\ s +$
$2\ gamma1\ k21^2\ km11^3\ km12^2\ km21\ km22\ s + k11\ k21^2\ km11^3\ km12^2\ km21\ km22\ s +$
$2\ gamma1\ k21\ k22\ km11^3\ km12^2\ km21\ km22\ s + k11\ k21\ k22\ km11^3\ km12^2\ km21\ km22\ s -$
$k11^2\ k21^3\ km12^3\ km21\ km22\ s + k11\ k21^3\ km11\ km12^3\ km21\ km22\ s +$
$k11\ k21^2\ k22\ km11\ km12^3\ km21\ km22\ s + gamma1\ k21^2\ km11^2\ km12^3\ km21\ km22\ s +$
$k11\ k21^2\ km11^2\ km12^3\ km21\ km22\ s + gamma1\ k21\ k22\ km11^2\ km12^3\ km21\ km22\ s +$
$k11\ k21\ k22\ km11^2\ km12^3\ km21\ km22\ s - gamma1\ k21^2\ k22\ km11^3\ km21^2\ km22\ s -$
$2\ gamma1\ k21\ k22^2\ km11^3\ km21^2\ km22\ s - gamma1\ k22^3\ km11^3\ km21^2\ km22\ s -$
$k11\ k22^3\ km11^3\ km21^2\ km22\ s - gamma1\ k21\ k22\ km11^4\ km21^2\ km22\ s -$
$gamma1\ k22^2\ km11^4\ km21^2\ km22\ s + gamma1\ k21^3\ km11^2\ km12\ km21^2\ km22\ s +$
$2\ gamma1\ k21^2\ k22\ km11^2\ km12\ km21^2\ km22\ s - k11\ k21^2\ k22\ km11^2\ km12\ km21^2\ km22\ s +$
$k21^3\ k22\ km11^2\ km12\ km21^2\ km22\ s + gamma1\ k21\ k22^2\ km11^2\ km12\ km21^2\ km22\ s +$
$k11\ k21\ k22^2\ km11^2\ km12\ km21^2\ km22\ s + 2\ k21^2\ k22^2\ km11^2\ km12\ km21^2\ km22\ s +$
$k21\ k22^3\ km11^2\ km12\ km21^2\ km22\ s + gamma1\ k21^2\ km11^3\ km12\ km21^2\ km22\ s -$
$k11\ k21\ k22\ km11^3\ km12\ km21^2\ km22\ s + 2\ k21^2\ k22\ km11^3\ km12\ km21^2\ km22\ s -$
$gamma1\ k22^2\ km11^3\ km12\ km21^2\ km22\ s - k11\ k22^2\ km11^3\ km12\ km21^2\ km22\ s +$
$2\ k21\ k22^2\ km11^3\ km12\ km21^2\ km22\ s + k21\ k22\ km11^4\ km12\ km21^2\ km22\ s +$
$k11\ k21^3\ km11\ km12^2\ km21^2\ km22\ s + gamma1\ k21^2\ km11^2\ km12^2\ km21^2\ km22\ s +$
$k11\ k21^2\ km11^2\ km12^2\ km21^2\ km22\ s + gamma1\ k21\ k22\ km11^2\ km12^2\ km21^2\ km22\ s +$
$k11\ k21\ k22\ km11^2\ km12^2\ km21^2\ km22\ s + 2\ k21^2\ k22\ km11^2\ km12^2\ km21^2\ km22\ s +$
$2\ k21\ k22^2\ km11^2\ km12^2\ km21^2\ km22\ s + 2\ k21\ k22\ km11^3\ km12^2\ km21^2\ km22\ s +$
$k21\ k22\ km11^2\ km12^3\ km21^2\ km22\ s - k21\ k22^2\ km11^3\ km21^3\ km22\ s -$
$k22^3\ km11^3\ km21^3\ km22\ s - k22^2\ km11^4\ km21^3\ km22\ s + k21^2\ k22\ km11^2\ km12\ km21^3\ km22\ s +$
$k21\ k22^2\ km11^2\ km12\ km21^3\ km22\ s + k21\ k22\ km11^3\ km12\ km21^3\ km22\ s -$
$k22^2\ km11^3\ km12\ km21^3\ km22\ s + k21\ k22\ km11^2\ km12^2\ km21^3\ km22\ s -$
$gamma1\ k11\ k21^3\ k22\ km11^2\ km21\ s^2 - gamma1\ k11\ k21^2\ k22^2\ km11^2\ km21\ s^2 -$
$gamma1\ k11\ k21^2\ k22\ km11^3\ km21\ s^2 - gamma1\ k11\ k21^3\ k22\ km11\ km12\ km21\ s^2 -$
$k11^2\ k21^3\ k22\ km11\ km12\ km21\ s^2 - gamma1\ k11\ k21^2\ k22^2\ km11\ km12\ km21\ s^2 -$
$k11^2\ k21^2\ k22^2\ km11\ km12\ km21\ s^2 - 2\ gamma1\ k11\ k21^2\ k22\ km11^2\ km12\ km21\ s^2 -$
$k11^2\ k21^2\ k22\ km11^2\ km12\ km21\ s^2 - gamma1\ k11\ k21^2\ k22\ km11\ km12^2\ km21\ s^2 -$
$k11^2\ k21^2\ k22\ km11\ km12^2\ km21\ s^2 - k11\ k21^2\ k22^2\ km11^2\ km21^2\ s^2 -$

$gamma1\ k21^2\ k22\ km11^3\ km21^2\ s^2 - 2\ gamma1\ k21\ k22^2\ km11^3\ km21^2\ s^2 -$
$k11\ k21\ k22^2\ km11^3\ km21^2\ s^2 - gamma1\ k22^3\ km11^3\ km21^2\ s^2 - k11\ k22^3\ km11^3\ km21^2\ s^2 -$
$gamma1\ k21\ k22\ km11^4\ km21^2\ s^2 - gamma1\ k22^2\ km11^4\ km21^2\ s^2 -$
$k11\ k21^2\ k22^2\ km11\ km12\ km21^2\ s^2 - k11\ k21^2\ k22\ km11^2\ km12\ km21^2\ s^2 -$
$gamma1\ k21\ k22\ km11^3\ km12\ km21^2\ s^2 - k11\ k21\ k22\ km11^3\ km12\ km21^2\ s^2 -$
$gamma1\ k22^2\ km11^3\ km12\ km21^2\ s^2 - k11\ k22^2\ km11^3\ km12\ km21^2\ s^2 -$
$k11\ k21^2\ k22\ km11\ km12^2\ km21^2\ s^2 - k21\ k22^2\ km11^3\ km21^3\ s^2 -$
$k22^3\ km11^3\ km21^3\ s^2 - k22^2\ km11^4\ km21^3\ s^2 - k22^2\ km11^3\ km12\ km21^3\ s^2 +$
$gamma1\ k11\ k21^3\ k22\ km11^2\ km22\ s^2 + gamma1\ k11\ k21^2\ k22^2\ km11^2\ km22\ s^2 +$
$gamma1\ k11\ k21^2\ k22\ km11^3\ km22\ s^2 + gamma1\ k11\ k21^3\ k22\ km11\ km12\ km22\ s^2 +$
$k11^2\ k21^3\ k22\ km11\ km12\ km22\ s^2 + gamma1\ k11\ k21^2\ k22^2\ km11\ km12\ km22\ s^2 +$
$k11^2\ k21^2\ k22^2\ km11\ km12\ km22\ s^2 + 2\ gamma1\ k11\ k21^2\ k22\ km11^2\ km12\ km22\ s^2 +$
$k11^2\ k21^2\ k22\ km11^2\ km12\ km22\ s^2 + gamma1\ k11\ k21^2\ k22\ km11\ km12^2\ km22\ s^2 +$
$k11^2\ k21^2\ k22\ km11\ km12^2\ km22\ s^2 + k11\ k21^2\ k22^2\ km11^2\ km21\ km22\ s^2 +$
$k11\ k21\ k22^2\ km11^3\ km21\ km22\ s^2 + k11\ k21^2\ k22^2\ km11\ km12\ km21\ km22\ s^2 +$
$gamma1\ k21^3\ km11^2\ km12\ km21\ km22\ s^2 + 2\ gamma1\ k21^2\ k22\ km11^2\ km12\ km21\ km22\ s^2 +$
$gamma1\ k21\ k22^2\ km11^2\ km12\ km21\ km22\ s^2 + k11\ k21\ k22^2\ km11^2\ km12\ km21\ km22\ s^2 +$
$gamma1\ k21^2\ km11^3\ km12\ km21\ km22\ s^2 + gamma1\ k21\ k22\ km11^3\ km12\ km21\ km22\ s^2 +$
$k11\ k21^3\ km11\ km12^2\ km21\ km22\ s^2 + k11\ k21^2\ k22\ km11\ km12^2\ km21\ km22\ s^2 +$
$gamma1\ k21^2\ km11^2\ km12^2\ km21\ km22\ s^2 + k11\ k21^2\ km11^2\ km12^2\ km21\ km22\ s^2 +$
$gamma1\ k21\ k22\ km11^2\ km12^2\ km21\ km22\ s^2 + k11\ k21\ k22\ km11^2\ km12^2\ km21\ km22\ s^2 +$
$k21^2\ k22\ km11^2\ km12\ km21^2\ km22\ s^2 + k21\ k22^2\ km11^2\ km12\ km21^2\ km22\ s^2 +$
$k21\ k22\ km11^3\ km12\ km21^2\ km22\ s^2 + k21\ k22\ km11^2\ km12^2\ km21^2\ km22\ s^2))\ /$
$(km11\ (km11 + km12)\ km21\ (gamma1^2\ k11\ k21^5\ km11^2\ km22 +$
$4\ gamma1^2\ k11\ k21^4\ k22\ km11^2\ km22 + 6\ gamma1^2\ k11\ k21^3\ k22^2\ km11^2\ km22 +$
$gamma1\ k11^2\ k21^3\ k22^2\ km11^2\ km22 + 4\ gamma1^2\ k11\ k21^2\ k22^3\ km11^2\ km22 +$
$2\ gamma1\ k11^2\ k21^2\ k22^3\ km11^2\ km22 + gamma1^2\ k11\ k21\ k22^4\ km11^2\ km22 +$
$gamma1\ k11^2\ k21\ k22^4\ km11^2\ km22 + 2\ gamma1^2\ k11\ k21^4\ km11^3\ km22 +$
$6\ gamma1^2\ k11\ k21^3\ k22\ km11^3\ km22 + 6\ gamma1^2\ k11\ k21^2\ k22^2\ km11^3\ km22 +$
$gamma1\ k11^2\ k21^2\ k22^2\ km11^3\ km22 + 2\ gamma1^2\ k11\ k21\ k22^3\ km11^3\ km22 +$
$gamma1\ k11^2\ k21\ k22^3\ km11^3\ km22 + gamma1^2\ k11\ k21^3\ km11^4\ km22 +$
$2\ gamma1^2\ k11\ k21^2\ k22\ km11^4\ km22 + gamma1^2\ k11\ k21\ k22^2\ km11^4\ km22 +$
$gamma1^2\ k11\ k21^5\ km11\ km12\ km22 + 2\ gamma1\ k11^2\ k21^5\ km11\ km12\ km22 +$
$4\ gamma1^2\ k11\ k21^4\ k22\ km11\ km12\ km22 + 6\ gamma1\ k11^2\ k21^4\ k22\ km11\ km12\ km22 +$
$6\ gamma1^2\ k11\ k21^3\ k22^2\ km11\ km12\ km22 + 8\ gamma1\ k11^2\ k21^3\ k22^2\ km11\ km12\ km22 +$
$k11^3\ k21^3\ k22^2\ km11\ km12\ km22 + 4\ gamma1^2\ k11\ k21^2\ k22^3\ km11\ km12\ km22 +$
$6\ gamma1\ k11^2\ k21^2\ k22^3\ km11\ km12\ km22 + 2\ k11^3\ k21^2\ k22^3\ km11\ km12\ km22 +$
$gamma1^2\ k11\ k21\ k22^4\ km11\ km12\ km22 + 2\ gamma1\ k11^2\ k21\ k22^4\ km11\ km12\ km22 +$
$k11^3\ k21\ k22^4\ km11\ km12\ km22 + 4\ gamma1^2\ k11\ k21^4\ km11^2\ km12\ km22 +$
$4\ gamma1\ k11^2\ k21^4\ km11^2\ km12\ km22 + 12\ gamma1^2\ k11\ k21^3\ k22\ km11^2\ km12\ km22 +$
$10\ gamma1\ k11^2\ k21^3\ k22\ km11^2\ km12\ km22 + 12\ gamma1^2\ k11\ k21^2\ k22^2\ km11^2\ km12\ km22 +$
$11\ gamma1\ k11^2\ k21^2\ k22^2\ km11^2\ km12\ km22 + k11^3\ k21^2\ k22^2\ km11^2\ km12\ km22 +$
$4\ gamma1^2\ k11\ k21\ k22^3\ km11^2\ km12\ km22 + 5\ gamma1\ k11^2\ k21\ k22^3\ km11^2\ km12\ km22 +$

$k11^3 k21 k22^3 km11^2 km12 km22 + 3 gamma1^2 k11 k21^3 km11^3 km12 km22 +$
$2 gamma1 k11^2 k21^3 km11^3 km12 km22 + 6 gamma1^2 k11 k21^2 k22 km11^3 km12 km22 +$
$4 gamma1 k11^2 k21^2 k22 km11^3 km12 km22 + 3 gamma1^2 k11 k21 k22^2 km11^3 km12 km22 +$
$2 gamma1 k11^2 k21 k22^2 km11^3 km12 km22 + gamma1 k11^2 k21^5 km12^2 km22 +$
$k11^3 k21^5 km12^2 km22 + 2 gamma1 k11^2 k21^4 k22 km12^2 km22 + 2 k11^3 k21^4 k22 km12^2 km22 +$
$gamma1 k11^2 k21^3 k22^2 km12^2 km22 + k11^3 k21^3 k22^2 km12^2 km22 +$
$2 gamma1^2 k11 k21^4 km11 km12^2 km22 + 5 gamma1 k11^2 k21^4 km11 km12^2 km22 +$
$2 k11^3 k21^4 km11 km12^2 km22 + 6 gamma1^2 k11 k21^3 k22 km11 km12^2 km22 +$
$11 gamma1 k11^2 k21^3 k22 km11 km12^2 km22 + 4 k11^3 k21^3 k22 km11 km12^2 km22 +$
$6 gamma1^2 k11 k21^2 k22^2 km11 km12^2 km22 + 10 gamma1 k11^2 k21^2 k22^2 km11 km12^2 km22 +$
$4 k11^3 k21^2 k22^2 km11 km12^2 km22 + 2 gamma1^2 k11 k21 k22^3 km11 km12^2 km22 +$
$4 gamma1 k11^2 k21 k22^3 km11 km12^2 km22 + 2 k11^3 k21 k22^3 km11 km12^2 km22 +$
$3 gamma1^2 k11 k21^3 km11^2 km12^2 km22 + 4 gamma1 k11^2 k21^3 km11^2 km12^2 km22 +$
$k11^3 k21^3 km11^2 km12^2 km22 + 6 gamma1^2 k11 k21^2 k22 km11^2 km12^2 km22 +$
$8 gamma1 k11^2 k21^2 k22 km11^2 km12^2 km22 + 2 k11^3 k21^2 k22 km11^2 km12^2 km22 +$
$3 gamma1^2 k11 k21 k22^2 km11^2 km12^2 km22 + 4 gamma1 k11^2 k21 k22^2 km11^2 km12^2 km22 +$
$k11^3 k21 k22^2 km11^2 km12^2 km22 + gamma1 k11^2 k21^4 km12^3 km22 +$
$k11^3 k21^4 km12^3 km22 + gamma1 k11^2 k21^3 k22 km12^3 km22 +$
$k11^3 k21^3 k22 km12^3 km22 + gamma1^2 k11 k21^3 km11 km12^3 km22 +$
$2 gamma1 k11^2 k21^3 km11 km12^3 km22 + k11^3 k21^3 km11 km12^3 km22 +$
$2 gamma1^2 k11 k21^2 k22 km11 km12^3 km22 + 4 gamma1 k11^2 k21^2 k22 km11 km12^3 km22 +$
$2 k11^3 k21^2 k22 km11 km12^3 km22 + gamma1^2 k11 k21 k22^2 km11 km12^3 km22 +$
$2 gamma1 k11^2 k21 k22^2 km11 km12^3 km22 + k11^3 k21 k22^2 km11 km12^3 km22 +$
$2 gamma1 k11 k21^4 k22 km11^2 km21 km22 + 6 gamma1 k11 k21^3 k22^2 km11^2 km21 km22 +$
$6 gamma1 k11 k21^2 k22^3 km11^2 km21 km22 + k11^2 k21^2 k22^3 km11^2 km21 km22 +$
$2 gamma1 k11 k21 k22^4 km11^2 km21 km22 + k11^2 k21 k22^4 km11^2 km21 km22 +$
$gamma1^2 k21^4 km11^3 km21 km22 + 4 gamma1^2 k21^3 k22 km11^3 km21 km22 +$
$4 gamma1 k11 k21^3 k22 km11^3 km21 km22 + 6 gamma1^2 k21^2 k22^2 km11^3 km21 km22 +$
$10 gamma1 k11 k21^2 k22^2 km11^3 km21 km22 + 4 gamma1^2 k21 k22^3 km11^3 km21 km22 +$
$8 gamma1 k11 k21 k22^3 km11^3 km21 km22 + k11^2 k21 k22^3 km11^3 km21 km22 +$
$gamma1^2 k22^4 km11^3 km21 km22 + 2 gamma1 k11 k22^4 km11^3 km21 km22 +$
$k11^2 k22^4 km11^3 km21 km22 + 2 gamma1^2 k21^3 km11^4 km21 km22 +$
$6 gamma1^2 k21^2 k22 km11^4 km21 km22 + 2 gamma1 k11 k21^2 k22 km11^4 km21 km22 +$
$6 gamma1^2 k21 k22^2 km11^4 km21 km22 + 4 gamma1 k11 k21 k22^2 km11^4 km21 km22 +$
$2 gamma1^2 k22^3 km11^4 km21 km22 + 2 gamma1 k11 k22^3 km11^4 km21 km22 +$
$gamma1^2 k21^2 km11^5 km21 km22 + 2 gamma1^2 k21 k22 km11^5 km21 km22 +$
$gamma1^2 k22^2 km11^5 km21 km22 + 2 gamma1 k11 k21^4 k22 km11 km12 km21 km22 +$
$2 k11^2 k21^4 k22 km11 km12 km21 km22 + 6 gamma1 k11 k21^3 k22^2 km11 km12 km21 km22 +$
$4 k11^2 k21^3 k22^2 km11 km12 km21 km22 + 6 gamma1 k11 k21^2 k22^3 km11 km12 km21 km22 +$
$4 k11^2 k21^2 k22^3 km11 km12 km21 km22 + 2 gamma1 k11 k21 k22^4 km11 km12 km21 km22 +$
$2 k11^2 k21 k22^4 km11 km12 km21 km22 + gamma1^2 k21^4 km11^2 km12 km21 km22 +$
$2 gamma1 k11 k21^4 km11^2 km12 km21 km22 + 4 gamma1^2 k21^3 k22 km11^2 km12 km21 km22 +$
$12 gamma1 k11 k21^3 k22 km11^2 km12 km21 km22 +$
$4 k11^2 k21^3 k22 km11^2 km12 km21 km22 + 6 gamma1^2 k21^2 k22^2 km11^2 km12 km21 km22 +$

$20\ gamma1\ k11\ k21^2\ k22^2\ km11^2\ km12\ km21\ km22 +$
$8\ k11^2\ k21^2\ k22^2\ km11^2\ km12\ km21\ km22 + 4\ gamma1^2\ k21\ k22^3\ km11^2\ km12\ km21\ km22 +$
$12\ gamma1\ k11\ k21\ k22^3\ km11^2\ km12\ km21\ km22 + 5\ k11^2\ k21\ k22^3\ km11^2\ km12\ km21\ km22 +$
$gamma1^2\ k22^4\ km11^2\ km12\ km21\ km22 + 2\ gamma1\ k11\ k22^4\ km11^2\ km12\ km21\ km22 +$
$k11^2\ k22^4\ km11^2\ km12\ km21\ km22 + 4\ gamma1^2\ k21^3\ km11^3\ km12\ km21\ km22 +$
$4\ gamma1\ k11\ k21^3\ km11^3\ km12\ km21\ km22 + 12\ gamma1^2\ k21^2\ k22\ km11^3\ km12\ km21\ km22 +$
$14\ gamma1\ k11\ k21^2\ k22\ km11^3\ km12\ km21\ km22 +$
$2\ k11^2\ k21^2\ k22\ km11^3\ km12\ km21\ km22 + 12\ gamma1^2\ k21\ k22^2\ km11^3\ km12\ km21\ km22 +$
$16\ gamma1\ k11\ k21\ k22^2\ km11^3\ km12\ km21\ km22 +$
$4\ k11^2\ k21\ k22^2\ km11^3\ km12\ km21\ km22 + 4\ gamma1^2\ k22^3\ km11^3\ km12\ km21\ km22 +$
$6\ gamma1\ k11\ k22^3\ km11^3\ km12\ km21\ km22 + 2\ k11^2\ k22^3\ km11^3\ km12\ km21\ km22 +$
$3\ gamma1^2\ k21^2\ km11^4\ km12\ km21\ km22 + 2\ gamma1\ k11\ k21^2\ km11^4\ km12\ km21\ km22 +$
$6\ gamma1^2\ k21\ k22\ km11^4\ km12\ km21\ km22 + 4\ gamma1\ k11\ k21\ k22\ km11^4\ km12\ km21\ km22 +$
$3\ gamma1^2\ k22^2\ km11^4\ km12\ km21\ km22 + 2\ gamma1\ k11\ k22^2\ km11^4\ km12\ km21\ km22 +$
$k11^2\ k21^4\ k22\ km12^2\ km21\ km22 + k11^2\ k21^3\ k22^2\ km12^2\ km21\ km22 +$
$2\ gamma1\ k11\ k21^4\ km11\ km12^2\ km21\ km22 + k11^2\ k21^4\ km11\ km12^2\ km21\ km22 +$
$8\ gamma1\ k11\ k21^3\ k22\ km11\ km12^2\ km21\ km22 + 5\ k11^2\ k21^3\ k22\ km11\ km12^2\ km21\ km22 +$
$10\ gamma1\ k11\ k21^2\ k22^2\ km11\ km12^2\ km21\ km22 + 8\ k11^2\ k21^2\ k22^2\ km11\ km12^2\ km21\ km22 +$
$4\ gamma1\ k11\ k21\ k22^3\ km11\ km12^2\ km21\ km22 + 4\ k11^2\ k21\ k22^3\ km11\ km12^2\ km21\ km22 +$
$2\ gamma1^2\ k21^3\ km11^2\ km12^2\ km21\ km22 + 6\ gamma1\ k11\ k21^3\ km11^2\ km12^2\ km21\ km22 +$
$2\ k11^2\ k21^3\ km11^2\ km12^2\ km21\ km22 + 6\ gamma1^2\ k21^2\ k22\ km11^2\ km12^2\ km21\ km22 +$
$16\ gamma1\ k11\ k21^2\ k22\ km11^2\ km12^2\ km21\ km22 +$
$6\ k11^2\ k21^2\ k22\ km11^2\ km12^2\ km21\ km22 + 6\ gamma1^2\ k21\ k22^2\ km11^2\ km12^2\ km21\ km22 +$
$14\ gamma1\ k11\ k21\ k22^2\ km11^2\ km12^2\ km21\ km22 + 6\ k11^2\ k21\ k22^2\ km11^2\ km12^2\ km21\ km22 +$
$2\ gamma1^2\ k22^3\ km11^2\ km12^2\ km21\ km22 + 4\ gamma1\ k11\ k22^3\ km11^2\ km12^2\ km21\ km22 +$
$2\ k11^2\ k22^3\ km11^2\ km12^2\ km21\ km22 + 3\ gamma1^2\ k21^2\ km11^3\ km12^2\ km21\ km22 +$
$4\ gamma1\ k11\ k21^2\ km11^3\ km12^2\ km21\ km22 + k11^2\ k21^2\ km11^3\ km12^2\ km21\ km22 +$
$6\ gamma1^2\ k21\ k22\ km11^3\ km12^2\ km21\ km22 + 8\ gamma1\ k11\ k21\ k22\ km11^3\ km12^2\ km21\ km22 +$
$2\ k11^2\ k21\ k22\ km11^3\ km12^2\ km21\ km22 + 3\ gamma1^2\ k22^2\ km11^3\ km12^2\ km21\ km22 +$
$4\ gamma1\ k11\ k22^2\ km11^3\ km12^2\ km21\ km22 + k11^2\ k22^2\ km11^3\ km12^2\ km21\ km22 +$
$k11^2\ k21^4\ km12^3\ km21\ km22 + k11^2\ k21^3\ k22\ km12^3\ km21\ km22 +$
$2\ gamma1\ k11\ k21^3\ km11\ km12^3\ km21\ km22 + 2\ k11^2\ k21^3\ km11\ km12^3\ km21\ km22 +$
$4\ gamma1\ k11\ k21^2\ k22\ km11\ km12^3\ km21\ km22 + 4\ k11^2\ k21^2\ k22\ km11\ km12^3\ km21\ km22 +$
$2\ gamma1\ k11\ k21\ k22^2\ km11\ km12^3\ km21\ km22 + 2\ k11^2\ k21\ k22^2\ km11\ km12^3\ km21\ km22 +$
$gamma1^2\ k21^2\ km11^2\ km12^3\ km21\ km22 + 2\ gamma1\ k11\ k21^2\ km11^2\ km12^3\ km21\ km22 +$
$k11^2\ k21^2\ km11^2\ km12^3\ km21\ km22 + 2\ gamma1^2\ k21\ k22\ km11^2\ km12^3\ km21\ km22 +$
$4\ gamma1\ k11\ k21\ k22\ km11^2\ km12^3\ km21\ km22 + 2\ k11^2\ k21\ k22\ km11^2\ km12^3\ km21\ km22 +$
$gamma1^2\ k22^2\ km11^2\ km12^3\ km21\ km22 + 2\ gamma1\ k11\ k22^2\ km11^2\ km12^3\ km21\ km22 +$
$k11^2\ k22^2\ km11^2\ km12^3\ km21\ km22 + k11\ k21^3\ k22^2\ km11^2\ km21^2\ km22 +$
$2\ k11\ k21^2\ k22^3\ km11^2\ km21^2\ km22 + k11\ k21\ k22^4\ km11^2\ km21^2\ km22 +$
$2\ gamma1\ k21^3\ k22\ km11^3\ km21^2\ km22 + 6\ gamma1\ k21^2\ k22^2\ km11^3\ km21^2\ km22 +$
$2\ k11\ k21^2\ k22^2\ km11^3\ km21^2\ km22 + 6\ gamma1\ k21\ k22^3\ km11^3\ km21^2\ km22 +$
$4\ k11\ k21\ k22^3\ km11^3\ km21^2\ km22 + 2\ gamma1\ k22^4\ km11^3\ km21^2\ km22 +$
$2\ k11\ k22^4\ km11^3\ km21^2\ km22 + 4\ gamma1\ k21^2\ k22\ km11^4\ km21^2\ km22 +$

$8 gamma1 k21 k22^2 km11^4 km21^2 km22 + k11 k21 k22^2 km11^4 km21^2 km22 +$
$4 gamma1 k22^3 km11^4 km21^2 km22 + 2 k11 k22^3 km11^4 km21^2 km22 +$
$2 gamma1 k21 k22 km11^5 km21^2 km22 + 2 gamma1 k22^2 km11^5 km21^2 km22 +$
$k11 k21^3 k22^2 km11 km12 km21^2 km22 + 2 k11 k21^2 k22^3 km11 km12 km21^2 km22 +$
$k11 k21 k22^4 km11 km12 km21^2 km22 + 2 gamma1 k21^3 k22 km11^2 km12 km21^2 km22 +$
$2 k11 k21^3 k22 km11^2 km12 km21^2 km22 + 6 gamma1 k21^2 k22^2 km11^2 km12 km21^2 km22 +$
$6 k11 k21^2 k22^2 km11^2 km12 km21^2 km22 + 6 gamma1 k21 k22^3 km11^2 km12 km21^2 km22 +$
$6 k11 k21 k22^3 km11^2 km12 km21^2 km22 + 2 gamma1 k22^4 km11^2 km12 km21^2 km22 +$
$2 k11 k22^4 km11^2 km12 km21^2 km22 + 8 gamma1 k21^2 k22 km11^3 km12 km21^2 km22 +$
$4 k11 k21^2 k22 km11^3 km12 km21^2 km22 + 16 gamma1 k21 k22^2 km11^3 km12 km21^2 km22 +$
$7 k11 k21 k22^2 km11^3 km12 km21^2 km22 + 8 gamma1 k22^3 km11^3 km12 km21^2 km22 +$
$6 k11 k22^3 km11^3 km12 km21^2 km22 + 6 gamma1 k21 k22 km11^4 km12 km21^2 km22 +$
$2 k11 k21 k22 km11^4 km12 km21^2 km22 + 6 gamma1 k22^2 km11^4 km12 km21^2 km22 +$
$2 k11 k22^2 km11^4 km12 km21^2 km22 + 2 k11 k21^3 k22 km11 km12^2 km21^2 km22 +$
$4 k11 k21^2 k22^2 km11 km12^2 km21^2 km22 + 2 k11 k21 k22^3 km11 km12^2 km21^2 km22 +$
$4 gamma1 k21^2 k22 km11^2 km12^2 km21^2 km22 + 6 k11 k21^2 k22 km11^2 km12^2 km21^2 km22 +$
$8 gamma1 k21 k22^2 km11^2 km12^2 km21^2 km22 + 7 k11 k21 k22^2 km11^2 km12^2 km21^2 km22 +$
$4 gamma1 k22^3 km11^2 km12^2 km21^2 km22 + 4 k11 k22^3 km11^2 km12^2 km21^2 km22 +$
$6 gamma1 k21 k22 km11^3 km12^2 km21^2 km22 + 4 k11 k21 k22 km11^3 km12^2 km21^2 km22 +$
$6 gamma1 k22^2 km11^3 km12^2 km21^2 km22 + 4 k11 k22^2 km11^3 km12^2 km21^2 km22 +$
$2 k11 k21^2 k22 km11 km12^3 km21^2 km22 + k11 k21 k22^2 km11 km12^3 km21^2 km22 +$
$2 gamma1 k21 k22 km11^2 km12^3 km21^2 km22 + 2 k11 k21 k22 km11^2 km12^3 km21^2 km22 +$
$2 gamma1 k22^2 km11^2 km12^3 km21^2 km22 + 2 k11 k22^2 km11^2 km12^3 km21^2 km22 +$
$k21^2 k22^2 km11^3 km21^3 km22 + 2 k21 k22^3 km11^3 km21^3 km22 + k22^4 km11^3 km21^3 km22 +$
$2 k21 k22^2 km11^4 km21^3 km22 + 2 k22^3 km11^4 km21^3 km22 + k22^2 km11^5 km21^3 km22 +$
$k21^2 k22^2 km11^2 km12 km21^3 km22 + 2 k21 k22^3 km11^2 km12 km21^3 km22 +$
$k22^4 km11^2 km12 km21^3 km22 + 4 k21 k22^2 km11^3 km12 km21^3 km22 +$
$4 k22^3 km11^3 km12 km21^3 km22 + 3 k22^2 km11^4 km12 km21^3 km22 +$
$2 k21 k22^2 km11^2 km12^2 km21^3 km22 + 2 k22^3 km11^2 km12^2 km21^3 km22 +$
$3 k22^2 km11^3 km12^2 km21^3 km22 + k22^2 km11^2 km12^3 km21^3 km22 +$
$gamma1 k11 k21^4 k22 km11^2 km21 s + 2 gamma1 k11 k21^3 k22^2 km11^2 km21 s +$
$gamma1 k11 k21^2 k22^3 km11^2 km21 s + 2 gamma1 k11 k21^3 k22 km11^3 km21 s +$
$2 gamma1 k11 k21^2 k22^2 km11^3 km21 s + gamma1 k11 k21^2 k22 km11^4 km21 s +$
$gamma1 k11 k21^4 k22 km11 km12 km21 s + k11^2 k21^4 k22 km11 km12 km21 s +$
$2 gamma1 k11 k21^3 k22^2 km11 km12 km21 s + 2 k11^2 k21^3 k22^2 km11 km12 km21 s +$
$gamma1 k11 k21^2 k22^3 km11 km12 km21 s + k11^2 k21^2 k22^3 km11 km12 km21 s +$
$4 gamma1 k11 k21^3 k22 km11^2 km12 km21 s + 2 k11^2 k21^3 k22 km11^2 km12 km21 s +$
$4 gamma1 k11 k21^2 k22^2 km11^2 km12 km21 s + 2 k11^2 k21^2 k22^2 km11^2 km12 km21 s +$
$3 gamma1 k11 k21^2 k22 km11^3 km12 km21 s + k11^2 k21^2 k22 km11^3 km12 km21 s +$
$2 gamma1 k11 k21^3 k22 km11 km12^2 km21 s + 2 k11^2 k21^3 k22 km11 km12^2 km21 s +$
$2 gamma1 k11 k21^2 k22^2 km11 km12^2 km21 s + 2 k11^2 k21^2 k22^2 km11 km12^2 km21 s +$
$3 gamma1 k11 k21^2 k22 km11^2 km12^2 km21 s + 2 k11^2 k21^2 k22 km11^2 km12^2 km21 s +$
$gamma1 k11 k21^2 k22 km11 km12^3 km21 s + k11^2 k21^2 k22 km11 km12^3 km21 s +$
$k11 k21^3 k22^2 km11^2 km21^2 s + k11 k21^2 k22^3 km11^2 km21^2 s +$

$\text{gamma1}\ k21^3\ k22\ km11^3\ km21^2\ s + 3\ \text{gamma1}\ k21^2\ k22^2\ km11^3\ km21^2\ s +$
$2\ k11\ k21^2\ k22^2\ km11^3\ km21^2\ s + 3\ \text{gamma1}\ k21\ k22^3\ km11^3\ km21^2\ s +$
$2\ k11\ k21\ k22^3\ km11^3\ km21^2\ s + \text{gamma1}\ k22^4\ km11^3\ km21^2\ s + k11\ k22^4\ km11^3\ km21^2\ s +$
$2\ \text{gamma1}\ k21^2\ k22\ km11^4\ km21^2\ s + 4\ \text{gamma1}\ k21\ k22^2\ km11^4\ km21^2\ s +$
$k11\ k21\ k22^2\ km11^4\ km21^2\ s + 2\ \text{gamma1}\ k22^3\ km11^4\ km21^2\ s + k11\ k22^3\ km11^4\ km21^2\ s +$
$\text{gamma1}\ k21\ k22\ km11^5\ km21^2\ s + \text{gamma1}\ k22^2\ km11^5\ km21^2\ s +$
$k11\ k21^3\ k22^2\ km11\ km12\ km21^2\ s + k11\ k21^2\ k22^3\ km11\ km12\ km21^2\ s +$
$k11\ k21^3\ k22\ km11^2\ km12\ km21^2\ s + 3\ k11\ k21^2\ k22^2\ km11^2\ km12\ km21^2\ s +$
$2\ \text{gamma1}\ k21^2\ k22\ km11^3\ km12\ km21^2\ s + 2\ k11\ k21^2\ k22\ km11^3\ km12\ km21^2\ s +$
$4\ \text{gamma1}\ k21\ k22^2\ km11^3\ km12\ km21^2\ s + 3\ k11\ k21\ k22^2\ km11^3\ km12\ km21^2\ s +$
$2\ \text{gamma1}\ k22^3\ km11^3\ km12\ km21^2\ s + 2\ k11\ k22^3\ km11^3\ km12\ km21^2\ s +$
$2\ \text{gamma1}\ k21\ k22\ km11^4\ km12\ km21^2\ s + k11\ k21\ k22\ km11^4\ km12\ km21^2\ s +$
$2\ \text{gamma1}\ k22^2\ km11^4\ km12\ km21^2\ s + k11\ k22^2\ km11^4\ km12\ km21^2\ s +$
$k11\ k21^3\ k22\ km11\ km12^2\ km21^2\ s + 2\ k11\ k21^2\ k22^2\ km11\ km12^2\ km21^2\ s +$
$2\ k11\ k21^2\ k22\ km11^2\ km12^2\ km21^2\ s + \text{gamma1}\ k21\ k22\ km11^3\ km12^2\ km21^2\ s +$
$k11\ k21\ k22\ km11^3\ km12^2\ km21^2\ s + \text{gamma1}\ k22^2\ km11^3\ km12^2\ km21^2\ s +$
$k11\ k22^2\ km11^3\ km12^2\ km21^2\ s + k11\ k21^2\ k22\ km11\ km12^3\ km21^2\ s +$
$k21^2\ k22^2\ km11^3\ km21^3\ s + 2\ k21\ k22^3\ km11^3\ km21^3\ s + k22^4\ km11^3\ km21^3\ s +$
$2\ k21\ k22^2\ km11^4\ km21^3\ s + 2\ k22^3\ km11^4\ km21^3\ s + k22^2\ km11^5\ km21^3\ s +$
$2\ k21\ k22^2\ km11^3\ km12\ km21^3\ s + 2\ k22^3\ km11^3\ km12\ km21^3\ s +$
$2\ k22^2\ km11^4\ km12\ km21^3\ s + k22^2\ km11^3\ km12^2\ km21^3\ s +$
$\text{gamma1}^2\ k11\ k21^4\ km11^2\ km22\ s + 3\ \text{gamma1}^2\ k11\ k21^3\ k22\ km11^2\ km22\ s +$
$3\ \text{gamma1}^2\ k11\ k21^2\ k22^2\ km11^2\ km22\ s + \text{gamma1}\ k11^2\ k21^2\ k22^2\ km11^2\ km22\ s +$
$\text{gamma1}\ k11\ k21^3\ k22^2\ km11^2\ km22\ s + \text{gamma1}^2\ k11\ k21\ k22^3\ km11^2\ km22\ s +$
$\text{gamma1}\ k11^2\ k21\ k22^3\ km11^2\ km22\ s + 2\ \text{gamma1}\ k11\ k21^2\ k22^3\ km11^2\ km22\ s +$
$\text{gamma1}\ k11\ k21\ k22^4\ km11^2\ km22\ s + \text{gamma1}^2\ k11\ k21^3\ km11^3\ km22\ s +$
$2\ \text{gamma1}^2\ k11\ k21^2\ k22\ km11^3\ km22\ s + \text{gamma1}^2\ k11\ k21\ k22^2\ km11^3\ km22\ s +$
$\text{gamma1}\ k11^2\ k21\ k22^2\ km11^3\ km22\ s + 2\ \text{gamma1}\ k11\ k21^2\ k22^2\ km11^3\ km22\ s +$
$2\ \text{gamma1}\ k11\ k21\ k22^3\ km11^3\ km22\ s + \text{gamma1}\ k11\ k21\ k22^2\ km11^4\ km22\ s +$
$\text{gamma1}^2\ k11\ k21^4\ km11\ km12\ km22\ s + 2\ \text{gamma1}\ k11^2\ k21^4\ km11\ km12\ km22\ s +$
$3\ \text{gamma1}^2\ k11\ k21^3\ k22\ km11\ km12\ km22\ s + 4\ \text{gamma1}\ k11^2\ k21^3\ k22\ km11\ km12\ km22\ s +$
$3\ \text{gamma1}^2\ k11\ k21^2\ k22^2\ km11\ km12\ km22\ s + 4\ \text{gamma1}\ k11^2\ k21^2\ k22^2\ km11\ km12\ km22\ s +$
$k11^3\ k21^2\ k22^2\ km11\ km12\ km22\ s + \text{gamma1}\ k11\ k21^3\ k22^2\ km11\ km12\ km22\ s +$
$k11^2\ k21^3\ k22^2\ km11\ km12\ km22\ s + \text{gamma1}^2\ k11\ k21\ k22^3\ km11\ km12\ km22\ s +$
$2\ \text{gamma1}\ k11^2\ k21\ k22^3\ km11\ km12\ km22\ s + k11^3\ k21\ k22^3\ km11\ km12\ km22\ s +$
$2\ \text{gamma1}\ k11\ k21^2\ k22^3\ km11\ km12\ km22\ s + 2\ k11^2\ k21^2\ k22^3\ km11\ km12\ km22\ s +$
$\text{gamma1}\ k11\ k21\ k22^4\ km11\ km12\ km22\ s + k11^2\ k21\ k22^4\ km11\ km12\ km22\ s +$
$2\ \text{gamma1}^2\ k11\ k21^3\ km11^2\ km12\ km22\ s + 2\ \text{gamma1}\ k11^2\ k21^3\ km11^2\ km12\ km22\ s +$
$4\ \text{gamma1}^2\ k11\ k21^2\ k22\ km11^2\ km12\ km22\ s + 2\ \text{gamma1}\ k11^2\ k21^2\ k22\ km11^2\ km12\ km22\ s +$
$2\ \text{gamma1}^2\ k11\ k21\ k22^2\ km11^2\ km12\ km22\ s + 3\ \text{gamma1}\ k11^2\ k21\ k22^2\ km11^2\ km12\ km22\ s +$
$k11^3\ k21\ k22^2\ km11^2\ km12\ km22\ s + 4\ \text{gamma1}\ k11\ k21^2\ k22^2\ km11^2\ km12\ km22\ s +$
$2\ k11^2\ k21^2\ k22^2\ km11^2\ km12\ km22\ s + 4\ \text{gamma1}\ k11\ k21\ k22^3\ km11^2\ km12\ km22\ s +$
$2\ k11^2\ k21\ k22^3\ km11^2\ km12\ km22\ s + 3\ \text{gamma1}\ k11\ k21\ k22^2\ km11^3\ km12\ km22\ s +$
$k11^2\ k21\ k22^2\ km11^3\ km12\ km22\ s + \text{gamma1}\ k11^2\ k21^4\ km12^2\ km22\ s +$

$k11^3 k21^4 km12^2 km22 s + gamma1 k11^2 k21^3 k22 km12^2 km22 s +$
$k11^3 k21^3 k22 km12^2 km22 s + gamma1^2 k11 k21^3 km11 km12^2 km22 s +$
$3 gamma1 k11^2 k21^3 km11 km12^2 km22 s + k11^3 k21^3 km11 km12^2 km22 s +$
$2 gamma1^2 k11 k21^2 k22 km11 km12^2 km22 s + 2 gamma1 k11^2 k21^2 k22 km11 km12^2 km22 s +$
$gamma1^2 k11 k21 k22^2 km11 km12^2 km22 s + 2 gamma1 k11^2 k21 k22^2 km11 km12^2 km22 s +$
$k11^3 k21 k22^2 km11 km12^2 km22 s + 2 gamma1 k11 k21^2 k22^2 km11 km12^2 km22 s +$
$2 k11^2 k21^2 k22^2 km11 km12^2 km22 s + 2 gamma1 k11 k21 k22^3 km11 km12^2 km22 s +$
$2 k11^2 k21 k22^3 km11 km12^2 km22 s + 3 gamma1 k11 k21 k22^2 km11^2 km12^2 km22 s +$
$2 k11^2 k21 k22^2 km11^2 km12^2 km22 s + gamma1 k11^2 k21^3 km12^3 km22 s +$
$k11^3 k21^3 km12^3 km22 s + gamma1 k11 k21 k22^2 km11 km12^3 km22 s +$
$k11^2 k21 k22^2 km11 km12^3 km22 s + 2 gamma1 k11 k21^3 k22 km11^2 km21 km22 s +$
$4 gamma1 k11 k21^2 k22^2 km11^2 km21 km22 s + 2 gamma1 k11 k21 k22^3 km11^2 km21 km22 s +$
$k11^2 k21 k22^3 km11^2 km21 km22 s + k11 k21^2 k22^3 km11^2 km21 km22 s +$
$k11 k21 k22^4 km11^2 km21 km22 s + gamma1^2 k21^3 km11^3 km21 km22 s +$
$3 gamma1^2 k21^2 k22 km11^3 km21 km22 s + 2 gamma1 k11 k21^2 k22 km11^3 km21 km22 s +$
$3 gamma1^2 k21 k22^2 km11^3 km21 km22 s + 4 gamma1 k11 k21 k22^2 km11^3 km21 km22 s +$
$gamma1^2 k22^3 km11^3 km21 km22 s + 2 gamma1 k11 k22^3 km11^3 km21 km22 s +$
$k11^2 k22^3 km11^3 km21 km22 s + 2 k11 k21 k22^3 km11^3 km21 km22 s +$
$k11 k22^4 km11^3 km21 km22 s + gamma1^2 k21^2 km11^4 km21 km22 s +$
$2 gamma1^2 k21 k22 km11^4 km21 km22 s + gamma1^2 k22^2 km11^4 km21 km22 s +$
$k11 k22^3 km11^4 km21 km22 s + 2 gamma1 k11 k21^3 k22 km11 km12 km21 km22 s +$
$2 k11^2 k21^3 k22 km11 km12 km21 km22 s + 4 gamma1 k11 k21^2 k22^2 km11 km12 km21 km22 s +$
$2 k11^2 k21^2 k22^2 km11 km12 km21 km22 s + 2 gamma1 k11 k21 k22^3 km11 km12 km21 km22 s +$
$2 k11^2 k21 k22^3 km11 km12 km21 km22 s + k11 k21^2 k22^3 km11 km12 km21 km22 s +$
$k11 k21 k22^4 km11 km12 km21 km22 s + gamma1^2 k21^3 km11^2 km12 km21 km22 s +$
$2 gamma1 k11 k21^3 km11^2 km12 km21 km22 s + 3 gamma1^2 k21^2 k22 km11^2 km12 km21 km22 s +$
$6 gamma1 k11 k21^2 k22 km11^2 km12 km21 km22 s + 2 k11^2 k21^2 k22 km11^2 km12 km21 km22 s +$
$gamma1 k21^3 k22 km11^2 km12 km21 km22 s + 3 gamma1^2 k21 k22^2 km11^2 km12 km21 km22 s +$
$6 gamma1 k11 k21 k22^2 km11^2 km12 km21 km22 s +$
$2 k11^2 k21 k22^2 km11^2 km12 km21 km22 s + 3 gamma1 k21^2 k22^2 km11^2 km12 km21 km22 s +$
$gamma1^2 k22^3 km11^2 km12 km21 km22 s + 2 gamma1 k11 k22^3 km11^2 km12 km21 km22 s +$
$k11^2 k22^3 km11^2 km12 km21 km22 s + 3 gamma1 k21 k22^3 km11^2 km12 km21 km22 s +$
$3 k11 k21 k22^3 km11^2 km12 km21 km22 s + gamma1 k22^4 km11^2 km12 km21 km22 s +$
$k11 k22^4 km11^2 km12 km21 km22 s + 2 gamma1^2 k21^2 km11^3 km12 km21 km22 s +$
$2 gamma1 k11 k21^2 km11^3 km12 km21 km22 s + 4 gamma1^2 k21 k22 km11^3 km12 km21 km22 s +$
$4 gamma1 k11 k21 k22 km11^3 km12 km21 km22 s +$
$2 gamma1 k21^2 k22 km11^3 km12 km21 km22 s + 2 gamma1^2 k22^2 km11^3 km12 km21 km22 s +$
$2 gamma1 k11 k22^2 km11^3 km12 km21 km22 s + 4 gamma1 k21 k22^2 km11^3 km12 km21 km22 s +$
$2 gamma1 k22^3 km11^3 km12 km21 km22 s + 2 k11 k22^3 km11^3 km12 km21 km22 s +$
$gamma1 k21 k22 km11^4 km12 km21 km22 s + gamma1 k22^2 km11^4 km12 km21 km22 s +$
$k11^2 k21^3 k22 km12^2 km21 km22 s + 2 gamma1 k11 k21^3 km11 km12^2 km21 km22 s +$
$k11^2 k21^3 km11 km12^2 km21 km22 s + 4 gamma1 k11 k21^2 k22 km11 km12^2 km21 km22 s +$
$2 k11^2 k21^2 k22 km11 km12^2 km21 km22 s + k11 k21^3 k22 km11 km12^2 km21 km22 s +$
$2 gamma1 k11 k21 k22^2 km11 km12^2 km21 km22 s + 2 k11^2 k21 k22^2 km11 km12^2 km21 km22 s +$

$2 k11 k21^{2} k22^{2} km11 km12^{2} km21 km22 s + 2 k11 k21 k22^{3} km11 km12^{2} km21 km22 s +$
$gamma1^{2} k21^{2} km11^{2} km12^{2} km21 km22 s + 2 gamma1 k11 k21^{2} km11^{2} km12^{2} km21 km22 s +$
$k11^{2} k21^{2} km11^{2} km12^{2} km21 km22 s + 2 gamma1^{2} k21 k22 km11^{2} km12^{2} km21 km22 s +$
$4 gamma1 k11 k21 k22 km11^{2} km12^{2} km21 km22 s +$
$2 k11^{2} k21 k22 km11^{2} km12^{2} km21 km22 s + 2 gamma1 k21^{2} k22 km11^{2} km12^{2} km21 km22 s +$
$2 k11 k21^{2} k22 km11^{2} km12^{2} km21 km22 s + gamma1^{2} k22^{2} km11^{2} km12^{2} km21 km22 s +$
$2 gamma1 k11 k22^{2} km11^{2} km12^{2} km21 km22 s + k11^{2} k22^{2} km11^{2} km12^{2} km21 km22 s +$
$4 gamma1 k21 k22^{2} km11^{2} km12^{2} km21 km22 s + 3 k11 k21 k22^{2} km11^{2} km12^{2} km21 km22 s +$
$2 gamma1 k22^{3} km11^{2} km12^{2} km21 km22 s + 2 k11 k22^{3} km11^{2} km12^{2} km21 km22 s +$
$2 gamma1 k21 k22 km11^{3} km12^{2} km21 km22 s + k11 k21 k22 km11^{3} km12^{2} km21 km22 s +$
$2 gamma1 k22^{2} km11^{3} km12^{2} km21 km22 s + k11 k22^{2} km11^{3} km12^{2} km21 km22 s +$
$k11^{2} k21^{3} km12^{3} km21 km22 s + k11 k21^{2} k22 km11 km12^{3} km21 km22 s +$
$k11 k21 k22^{2} km11 km12^{3} km21 km22 s + gamma1 k21 k22 km11^{2} km12^{3} km21 km22 s +$
$k11 k21 k22 km11^{2} km12^{3} km21 km22 s + gamma1 k22^{2} km11^{2} km12^{3} km21 km22 s +$
$k11 k22^{2} km11^{2} km12^{3} km21 km22 s + k11 k21^{2} k22^{2} km11^{2} km21^{2} km22 s +$
$k11 k21 k22^{3} km11^{2} km21^{2} km22 s + 2 gamma1 k21^{2} k22 km11^{3} km21^{2} km22 s +$
$4 gamma1 k21 k22^{2} km11^{3} km21^{2} km22 s + k11 k21 k22^{2} km11^{3} km21^{2} km22 s +$
$2 gamma1 k22^{3} km11^{3} km21^{2} km22 s + 2 k11 k22^{3} km11^{3} km21^{2} km22 s +$
$2 gamma1 k21 k22 km11^{4} km21^{2} km22 s + 2 gamma1 k22^{2} km11^{4} km21^{2} km22 s +$
$k11 k21^{2} k22^{2} km11 km12 km21^{2} km22 s + k11 k21 k22^{3} km11 km12 km21^{2} km22 s +$
$2 gamma1 k21^{2} k22 km11^{2} km12 km21^{2} km22 s + 2 k11 k21^{2} k22 km11^{2} km12 km21^{2} km22 s +$
$4 gamma1 k21 k22^{2} km11^{2} km12 km21^{2} km22 s + 2 k11 k21 k22^{2} km11^{2} km12 km21^{2} km22 s +$
$k21^{2} k22^{2} km11^{2} km12 km21^{2} km22 s + 2 gamma1 k22^{3} km11^{2} km12 km21^{2} km22 s +$
$2 k11 k22^{3} km11^{2} km12 km21^{2} km22 s + 2 k21 k22^{3} km11^{2} km12 km21^{2} km22 s +$
$k22^{4} km11^{2} km12 km21^{2} km22 s + 4 gamma1 k21 k22 km11^{3} km12 km21^{2} km22 s +$
$2 k11 k21 k22 km11^{3} km12 km21^{2} km22 s + 4 gamma1 k22^{2} km11^{3} km12 km21^{2} km22 s +$
$2 k11 k22^{2} km11^{3} km12 km21^{2} km22 s + 2 k21 k22^{2} km11^{3} km12 km21^{2} km22 s +$
$2 k22^{3} km11^{3} km12 km21^{2} km22 s + k22^{2} km11^{4} km12 km21^{2} km22 s +$
$2 k11 k21^{2} k22 km11 km12^{2} km21^{2} km22 s + k11 k21 k22^{2} km11 km12^{2} km21^{2} km22 s +$
$2 gamma1 k21 k22 km11^{2} km12^{2} km21^{2} km22 s + 2 k11 k21 k22 km11^{2} km12^{2} km21^{2} km22 s +$
$2 gamma1 k22^{2} km11^{2} km12^{2} km21^{2} km22 s + 2 k11 k22^{2} km11^{2} km12^{2} km21^{2} km22 s +$
$2 k21 k22^{2} km11^{2} km12^{2} km21^{2} km22 s + 2 k22^{3} km11^{2} km12^{2} km21^{2} km22 s +$
$2 k22^{2} km11^{3} km12^{2} km21^{2} km22 s + k22^{2} km11^{2} km12^{3} km21^{2} km22 s +$
$k21 k22^{2} km11^{3} km21^{3} km22 s + k22^{3} km11^{3} km21^{3} km22 s + k22^{2} km11^{4} km21^{3} km22 s +$
$k21 k22^{2} km11^{2} km12 km21^{3} km22 s + k22^{3} km11^{2} km12 km21^{3} km22 s +$
$2 k22^{2} km11^{3} km12 km21^{3} km22 s + k22^{2} km11^{2} km12^{2} km21^{3} km22 s +$
$gamma1 k11 k21^{3} k22 km11^{2} km21 s^{2} + gamma1 k11 k21^{2} k22^{2} km11^{2} km21 s^{2} +$
$gamma1 k11 k21^{2} k22 km11^{3} km21 s^{2} + gamma1 k11 k21^{3} k22 km11 km12 km21 s^{2} +$
$k11^{2} k21^{3} k22 km11 km12 km21 s^{2} + gamma1 k11 k21^{2} k22^{2} km11 km12 km21 s^{2} +$
$k11^{2} k21^{2} k22^{2} km11 km12 km21 s^{2} + 2 gamma1 k11 k21^{2} k22 km11^{2} km12 km21 s^{2} +$
$k11^{2} k21^{2} k22 km11^{2} km12 km21 s^{2} + gamma1 k11 k21^{2} k22 km11 km12^{2} km21 s^{2} +$
$k11^{2} k21^{2} k22 km11 km12^{2} km21 s^{2} + k11 k21^{2} k22^{2} km11^{2} km21^{2} s^{2} +$
$gamma1 k21^{2} k22 km11^{3} km21^{2} s^{2} + 2 gamma1 k21 k22^{2} km11^{3} km21^{2} s^{2} +$
$k11 k21 k22^{2} km11^{3} km21^{2} s^{2} + gamma1 k22^{3} km11^{3} km21^{2} s^{2} + k11 k22^{3} km11^{3} km21^{2} s^{2} +$

```
gamma1 k21 k22 km11^4 km21^2 s^2 + gamma1 k22^2 km11^4 km21^2 s^2 +
k11 k21^2 k22^2 km11 km12 km21^2 s^2 + k11 k21^2 k22 km11^2 km12 km21^2 s^2 +
gamma1 k21 k22 km11^3 km12 km21^2 s^2 + k11 k21 k22 km11^3 km12 km21^2 s^2 +
gamma1 k22^2 km11^3 km12 km21^2 s^2 + k11 k22^2 km11^3 km12 km21^2 s^2 +
k11 k21^2 k22 km11 km12^2 km21^2 s^2 + k21 k22^2 km11^3 km21^3 s^2 +
k22^3 km11^3 km21^3 s^2 + k22^2 km11^4 km21^3 s^2 + k22^2 km11^3 km12 km21^3 s^2 +
gamma1 k11 k21^2 k22^2 km11^2 km22 s^2 + gamma1 k11 k21 k22^3 km11^2 km22 s^2 +
gamma1 k11 k21 k22^2 km11^3 km22 s^2 + gamma1 k11 k21^2 k22^2 km11 km12 km22 s^2 +
k11^2 k21^2 k22^2 km11 km12 km22 s^2 + gamma1 k11 k21 k22^3 km11 km12 km22 s^2 +
k11^2 k21 k22^3 km11 km12 km22 s^2 + 2 gamma1 k11 k21 k22^2 km11^2 km12 km22 s^2 +
k11^2 k21 k22^2 km11^2 km12 km22 s^2 + gamma1 k11 k21 k22^2 km11 km12^2 km22 s^2 +
k11^2 k21 k22^2 km11 km12^2 km22 s^2 + k11 k21 k22^3 km11^2 km21 km22 s^2 +
k11 k22^3 km11^3 km21 km22 s^2 + k11 k21 k22^3 km11 km12 km21 km22 s^2 +
gamma1 k21^2 k22 km11^2 km12 km21 km22 s^2 + 2 gamma1 k21 k22^2 km11^2 km12 km21 km22 s^2 +
gamma1 k22^3 km11^2 km12 km21 km22 s^2 + k11 k22^3 km11^2 km12 km21 km22 s^2 +
gamma1 k21 k22 km11^3 km12 km21 km22 s^2 + gamma1 k22^2 km11^3 km12 km21 km22 s^2 +
k11 k21^2 k22 km11 km12^2 km21 km22 s^2 + k11 k21 k22^2 km11 km12^2 km21 km22 s^2 +
gamma1 k21 k22 km11^2 km12^2 km21 km22 s^2 + k11 k21 k22 km11^2 km12^2 km21 km22 s^2 +
gamma1 k22^2 km11^2 km12^2 km21 km22 s^2 + k11 k22^2 km11^2 km12^2 km21 km22 s^2 +
k21 k22^2 km11^2 km12 km21^2 km22 s^2 + k22^3 km11^2 km12 km21^2 km22 s^2 +
k22^2 km11^3 km12 km21^2 km22 s^2 + k22^2 km11^2 km12^2 km21^2 km22 s^2)))
```

In[56]:= 
```
Factor[Simplify[Together[pplus / pminus - k11 * k21 / (km11 * km21)]]]
```

Out[56]=
```
-((k11 (k22 km11 - k21 km12)^2 (k11 k21 - km11 km21)) /
  (km11 (km11 + km12) km21 (gamma1 k21^2 km11 + 2 gamma1 k21 k22 km11 + gamma1 k22^2 km11 +
      k11 k22^2 km11 + gamma1 k21 km11^2 + gamma1 k22 km11^2 + k11 k21^2 km12 +
      gamma1 k21 km11 km12 + k11 k21 km11 km12 + gamma1 k22 km11 km12 + k11 k22 km11 km12 +
      k21 k22 km11 km21 + k22^2 km11 km21 + k22 km11^2 km21 + k22 km11 km12 km21)))
```

In[57]:= 
```
Factor[Simplify[Together[J]]]
```

Out[57]=
```
(k22 (k22 km11 - k21 km12) km21 (-k11 k21 + km11 km21) km22) /
 ((k22 km21 + k21 km22) (gamma1 k21 k22 km11 km21 + gamma1 k22^2 km11 km21 +
    k11 k22^2 km11 km21 + gamma1 k22 km11^2 km21 + gamma1 k22 km11 km12 km21 + k11 k22
      km11 km12 km21 + k22^2 km11 km21^2 + k22 km11 km12 km21^2 + gamma1 k11 k21 km11 km22 +
    gamma1 k21^2 km11 km22 + gamma1 k21 k22 km11 km22 + gamma1 k21 km11^2 km22 +
    gamma1 k11 k21 km12 km22 + k11^2 k21 km12 km22 + k11 k21^2 km12 km22 +
    gamma1 k21 km11 km12 km22 + k11 k21 km11 km12 km22 + gamma1 k21 km11 km21 km22 +
    gamma1 k22 km11 km21 km22 + k11 k22 km11 km21 km22 + k21 k22 km11 km21 km22 +
    k22 km11^2 km21 km22 + k11 k21 km12 km21 km22 + k22 km11 km21^2 km22))
```

In[58]:= `zetaeff = Factor[Simplify[Together[(k11 * k21 / (km11 * km21) - pplus / pminus) / J^2]]]`

Out[58]=

$$\Big(k11\ (k22\ km21 + k21\ km22)^2\ \big(gamma1\ k21\ k22\ km11\ km21 + gamma1\ k22^2\ km11\ km21 + k11\ k22^2\ km11\ km21 + gamma1\ k22\ km11^2\ km21 + gamma1\ k22\ km11\ km12\ km21 + k11\ k22\ km11\ km12\ km21 + k22^2\ km11\ km21^2 + k22\ km11\ km12\ km21^2 + gamma1\ k11\ k21\ km11\ km22 + gamma1\ k21^2\ km11\ km22 + gamma1\ k21\ k22\ km11\ km22 + gamma1\ k21\ km11^2\ km22 + gamma1\ k11\ k21\ km12\ km22 + k11^2\ k21\ km12\ km22 + k11\ k21^2\ km12\ km22 + gamma1\ k21\ km11\ km12\ km22 + k11\ k21\ km11\ km12\ km22 + gamma1\ k21\ km11\ km21\ km22 + gamma1\ k22\ km11\ km21\ km22 + k11\ k22\ km11\ km21\ km22 + k21\ k22\ km11\ km21\ km22 + k22\ km11^2\ km21\ km22 + k11\ k21\ km12\ km21\ km22 + k22\ km11\ km21^2\ km22\big)^2\Big) \Big/ \Big(k22^2\ km11\ (km11 + km12)\ km21^3\ (k11\ k21 - km11\ km21)\ \big(gamma1\ k21^2\ km11 + 2\ gamma1\ k21\ k22\ km11 + gamma1\ k22^2\ km11 + k11\ k22^2\ km11 + gamma1\ k21\ km11^2 + gamma1\ k22\ km11^2 + k11\ k21^2\ km12 + gamma1\ k21\ km11\ km12 + k11\ k21\ km11\ km12 + gamma1\ k22\ km11\ km12 + k11\ k22\ km11\ km12 + k21\ k22\ km11\ km21 + k22^2\ km11\ km21 + k22\ km11^2\ km21 + k22\ km11\ km12\ km21\big)\ km22^2\Big)$$
